# Supplementary material for: AR4D: Autoregressive 4D Generation from Monocular Videos
Source: arXiv:2501.01722 source file (2025-01-03)
Supplement: Supplementary file 1 [file X_suppl.tex]

\clearpage
\setcounter{page}{1}
\maketitlesupplementary

In Sec.~\ref{Experimental details}, we provide a  detailed overview of experimental details, including datasets, implementation details, baselines and metrics. Sec.~\ref{More related works} provides an expanded discussion of related works, focusing on 3D generation and 4D reconstruction. We also present additional visualizations, including ablation studies, comparisons with state-of-the-art methods, 4D assets generated by our method, as detailed in Sec.~\ref{More visualizations of ablation studies}, Sec.~\ref{More visualizations of comparisons with state-of-the-art method} and Sec.~\ref{More visualizations of 4D assets generated by AR4D} respectively. The limitations of our approach and potential directions for future work are discussed in Sec.~\ref{Limitations and future works}.

\section{Experimental details} \label{Experimental details}
\subsection{Datasets}
To demonstrate the effectiveness of our proposed method, we follow STAG4D~\cite{zeng2025stag4d} and conduct experiments on its provided dataset, which includes both the Video-to-4D and Text-to-4D datasets. The Video-to-4D dataset contains 28 unique scenes, each featuring a 32-frame monocular video of a single object with a fixed viewpoint, either synthesized or captured. The Text-to-4D process involves two stages: first, a video is generated from the textual input, and second, this video is used to produce a 4D asset. As the Text-to-4D dataset only provides pre-generated videos without the corresponding text descriptions, we utilize these videos directly to create the associated 4D targets. Specifically, the Text-to-4D dataset includes 21 unique scenes, each consisting of a 26-frame monocular video of a single object with a fixed viewpoint.

\subsection{Implementation details}
For 4D object generation, in the \textbf{\textit{Initialization}} stage, we first use MVDream~\cite{shi2023mvdream} to generate four orthogonal views of the first frame from the input video. These views are then fed into LGM~\cite{tang2024lgm} to obtain the corresponding 3D Gaussian representations. Due to the inherent limitations of MVDream, the generated novel views may not always meet quality expectations; in such cases, multiple attempts are encouraged to achieve the most satisfactory results for subsequent stages. After obtaining the 3D representation for the first frame, we fine-tune these 3D Gaussians to better align with the first frame itself. This fine-tuning is performed with a learning rate of $1 \times 10^{-5}$ over 1000 iterations. During the \textbf{\textit{Generation}} stage, the input video is assumed to be bind with a camera pose of azimuth angle equals to $\ang{0}$, elevation angle equals to $\ang{0}$, and radius equals to 1.5. To achieve progressive view sampling, we first render four orthogonal views of the 3D representation that is currently being optimized, with azimuth angle equals to $\{\ang{0}, \ang{90}, \ang{180}, \ang{270}\}$ respectively, and elevation angle equals to $\ang{0}$,  radius equals to 1.5. These views are then input into LGM to generate additional pseudo-labels, on the purpose of prevent overfitting. During the \textbf{\textit{Refinement}} stage, the MLP-based global deformation field may occasionally converge to a local optimum, causing training collapse. In such cases, we recommend re-initializing the network or using an improved architecture, such as the one proposed by~\cite{zhu2024vanilla}. 
All results are rendered at a resolution of 512 $\times$ 512, which is the maximum resolution supported by LGM for processing.

For 4D scene generation, we use Splatt3R~\cite{smart2024splatt3r} as both the 3D generator and large-scale 3D reconstruction model. 
Unlike object-level generation, where LGM~\cite{tang2024lgm} can generate views of an object from any viewpoint, Splatt3R can only produce artifact-free results when generating views that are close to the input video's original viewpoint. In this case, during the \textbf{\textit{Generation}} stage, the proposed progressive view sampling strategy becomes unnecessary, and thus we do not apply it in practice.

\subsection{Baselines}
We compared our proposed AR4D with several state-of-the-art methods, \ie, Consistent4D~\cite{jiang2023consistent4d}, SV4D~\cite{xie2024sv4d}, STAG4D~\cite{zeng2025stag4d}, Deform 3DGS~\cite{yang2024deformable}. We make a brief introduction here.

\paragraph{Consistent4D~\cite{jiang2023consistent4d}}
As one of the first works towards 4D generation, Consistent4D realizes Video-to-4D by leveraging a 3D-aware image diffusion model to supervise the training process of  Dynamic Neural Radiance Fields (DyNeRF), which is further enhanced by a super-resolution based video enhancer. The final obtained 4D assets can be rendered at a resolution of 256 $\times$ 256.

\vspace{-2mm}
\paragraph{SV4D~\cite{xie2024sv4d}}
SV4D is a unified latent diffusion model trained on large-scale multi-modal datasets that can generate novel-view videos of dynamic 3D objects. Subsequently, an implicit 4D representation (\ie, NeRF) will be optimized using these multi-view videos.

\vspace{-2mm}
\paragraph{STAG4D~\cite{zeng2025stag4d}}
Similar to SV4D, STAG4D generates multi-view video sequences by enhancing the attention fusion mechanism within pre-trained multi-view diffusion models. These sequences are then refined using score distillation sampling (SDS) coupled with an adaptive densification strategy, on the purpose of improved performance and consistency across views.

\vspace{-2mm}
\paragraph{Deform 3DGS~\cite{yang2024deformable}}
Given multi-view or monocular videos, Deform 3DGS introduces a deformation field that is jointly optimized with the canonical space to accurately estimate 4D content.

% \vspace{-2mm}
\subsection{Metrics}
To demonstrate the superiority of our proposed method, we report metrics including PSNR, SSIM, LPIPS, CLIP-S, and FVD. In particular, to evaluate alignment with the input videos, we calculate PSNR, SSIM, and LPIPS between the rendered videos and input videos at an azimuth angle of $\ang{0}$, an elevation angle of $\ang{0}$, and a radius of 1.5. To measure the degree of spatial-temporal consistency, we report the average value of CLIP-S and FVD between input videos and novel-view videos  rendered at azimuth angles of $\ang{0},\ang{-45}, \ang{45}$.

\section{More related works} \label{More related works}
\subsection{3D Generation}
The rapid advancements in image generation~\cite{rombach2022high,zhang2023adding,mou2024t2i,podell2023sdxl} and video generation~\cite{wu2023tune,blattmann2023stable,villegas2022phenaki,zhang2024show} have sparked significant interest in the field of 3D generation. To address the challenge of limited 3D datasets, Dreamfusion~\cite{poole2022dreamfusion} proposed the concept of SDS, which has inspired numerous follow-up works~\cite{lin2023magic3d,chen2023fantasia3d,qian2023magic123,liu2024humangaussian,hu2024efficientdreamer}. 
To overcome the inherent limitations of SDS, various improvements have been proposed. For instance, ProlificDreamer~\cite{wang2024prolificdreamer} proposed VSD for synthesizing objects with higher diversity. DreamTime~\cite{huang2023dreamtime} proposed a timestep annealing strategy to overcome the over-saturation problem of SDS. Moreover, LucidDreamer~\cite{liang2024luciddreamer} introduced interval score sampling for high-fidelity generation. DreamGaussian~\cite{tang2023dreamgaussian} introduced the 3D Gaussian Splatting (3DGS) representation, enabling significantly faster 3D generation, where realistic 3D objects can be synthesized within minutes. Recently, with the development of large-scale 3D datasets~\cite{deitke2023objaverse}, several methods~\cite{liu2023zero,liu2024one, shi2023mvdream, tang2024lgm,hong2023lrm} have explored building generalized frameworks for 3D generation, where diverse 3D contents can be generated in a feed-forward process without per-scene optimization. In this paper, we aim to extend the capabilities of existing 3D generation models to the task of 4D generation, without relying on SDS.

\subsection{4D Reconstruction}
4D reconstruction (\ie, dynamic 3D reconstruction) has long been a challenging problem in computer vision and graphics, attracting growing attention in recent years. Early approaches~\cite{pumarola2021d,attal2023hyperreel,fridovich2023k,wang2023neural} extended the static NeRF~\cite{mildenhall2021nerf} framework to dynamic scenes, achieving photorealistic results but suffering from extremely slow training and rendering speeds. Recently, inspired by the powerful abilities of 3DGS~\cite{kerbl20233d}, researchers have begun to explore its integration into 4D reconstruction to improve efficiency. To achieve this goal, similar to~\cite{pumarola2021d}, mainstream methods~\cite{wu20244d,yang2024deformable,pumarola2021d,attal2023hyperreel} typically leverage a canonical space paired with a global deformation field to model motions across frames.
More recently, several methods~\cite{sun20243dgstream,luiten2024dynamic,he2024s4d} proposed to realize efficient 4D reconstruction on a per-frame training manner from multi-view videos, either by introducing Neural Transformation Cache or additional priors such as optical flows. In contrast, our approach targets 4D generation from monocular videos with a fixed viewpoint, a significantly more challenging task that demands precise estimation of motion, geometry, and appearance.

% \vspace{-6mm}
\section{More visualizations of ablation studies}
\label{More visualizations of ablation studies}
To demonstrate the effectiveness of our design choices, we provide additional visualizations of the generated multi-view videos from the ablation studies conducted in Sec.~\ref{sec: ablations}. 
As shown in Fig.~\ref{fig:supply_ablation_1}(a), directly applying typical 4D reconstruction methods results in noticeable artifacts due to the use of monocular videos with a fixed viewpoint for supervision, rather than multi-view videos or monocular videos with varying viewpoints. 
When relying solely on autoregressive generation, severe artifacts tend to appear, especially in later frames, due to the overfitting problem, as shown in Fig.~\ref{fig:supply_ablation_1}(b).
Similarly, as shown in Fig.~\ref{fig:supply_ablation_2}(b), removing autoregressive generation (\ie, using only the progressive view sampling strategy) makes accurate motion estimation difficult, particularly in frames with significant motion changes. By combining autoregressive generation with the progressive view sampling strategy, we can achieve optimal performance, significantly enhancing spatiotemporal consistency, as demonstrated in Fig.~\ref{fig:supply_ablation_1}(c) and Fig.~\ref{fig:supply_ablation_2}(c). We further conduct additional visualizations of ablation studies on the \textbf{\textit{Refinement}} stage. As shown in Fig.~\ref{fig:supply_ablation_3}, removing the refinement stage results in noticeable appearance drift. In contrast, including this refinement significantly improves the spatial-temporal consistency of the 4D objects generated.

\begin{figure*}[t]
    \centering
    \begin{subfigure}[b]{1\textwidth}
        \centering
        \includegraphics[width=0.82\textwidth]{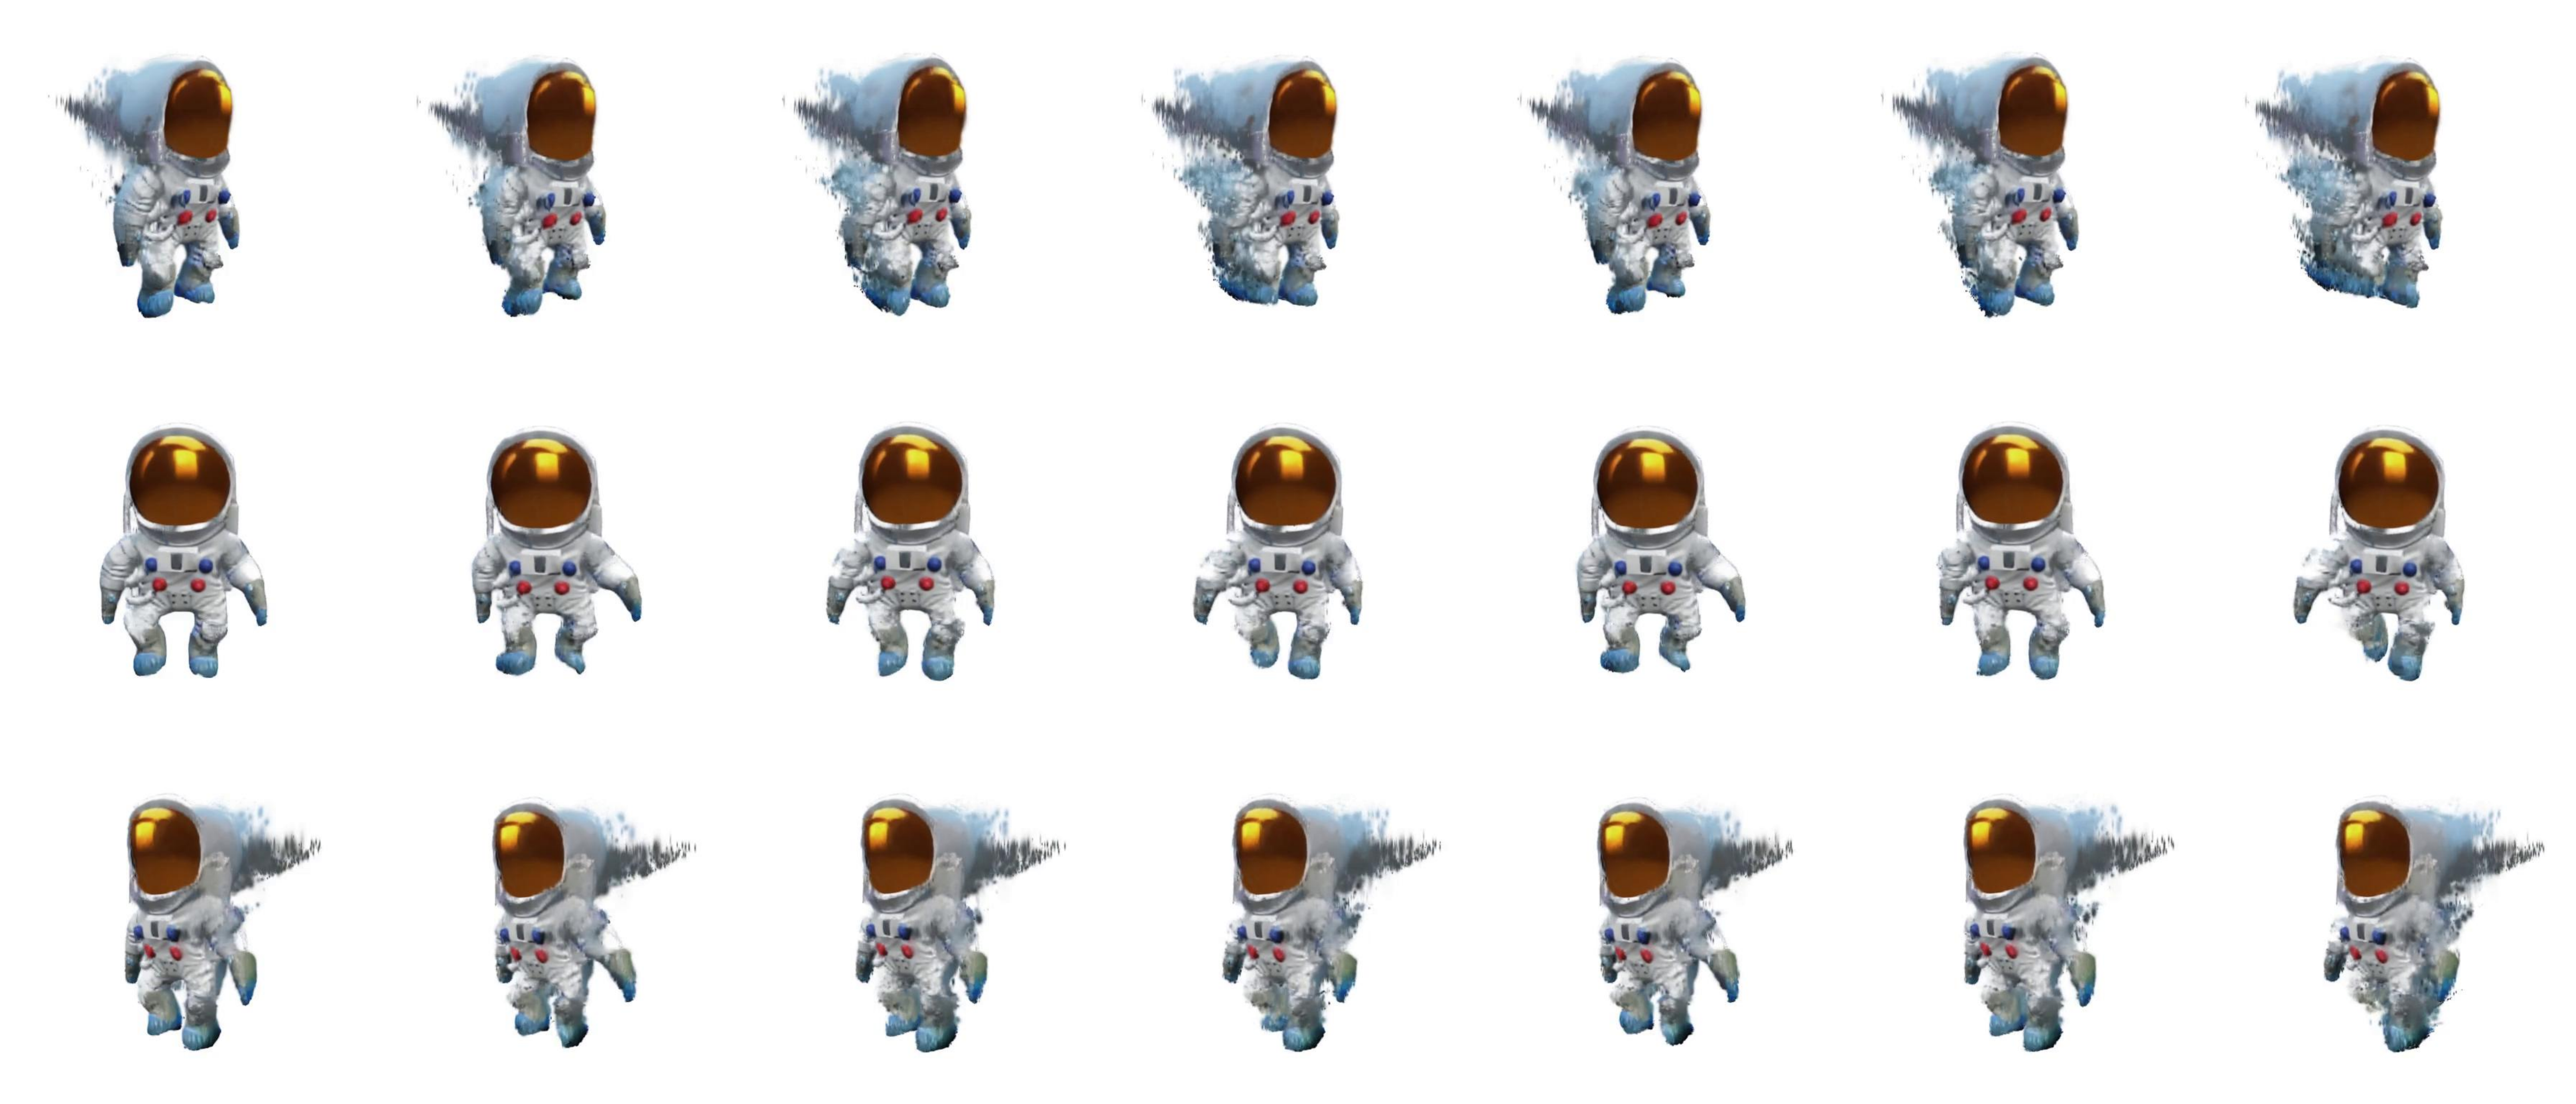}
        \caption{Multi-view videos rendered by directly using typical 4D reconstruction methods.}
    \end{subfigure}
    \hfill
    \begin{subfigure}[b]{1\textwidth}
        \centering
        \includegraphics[width=0.82\textwidth]{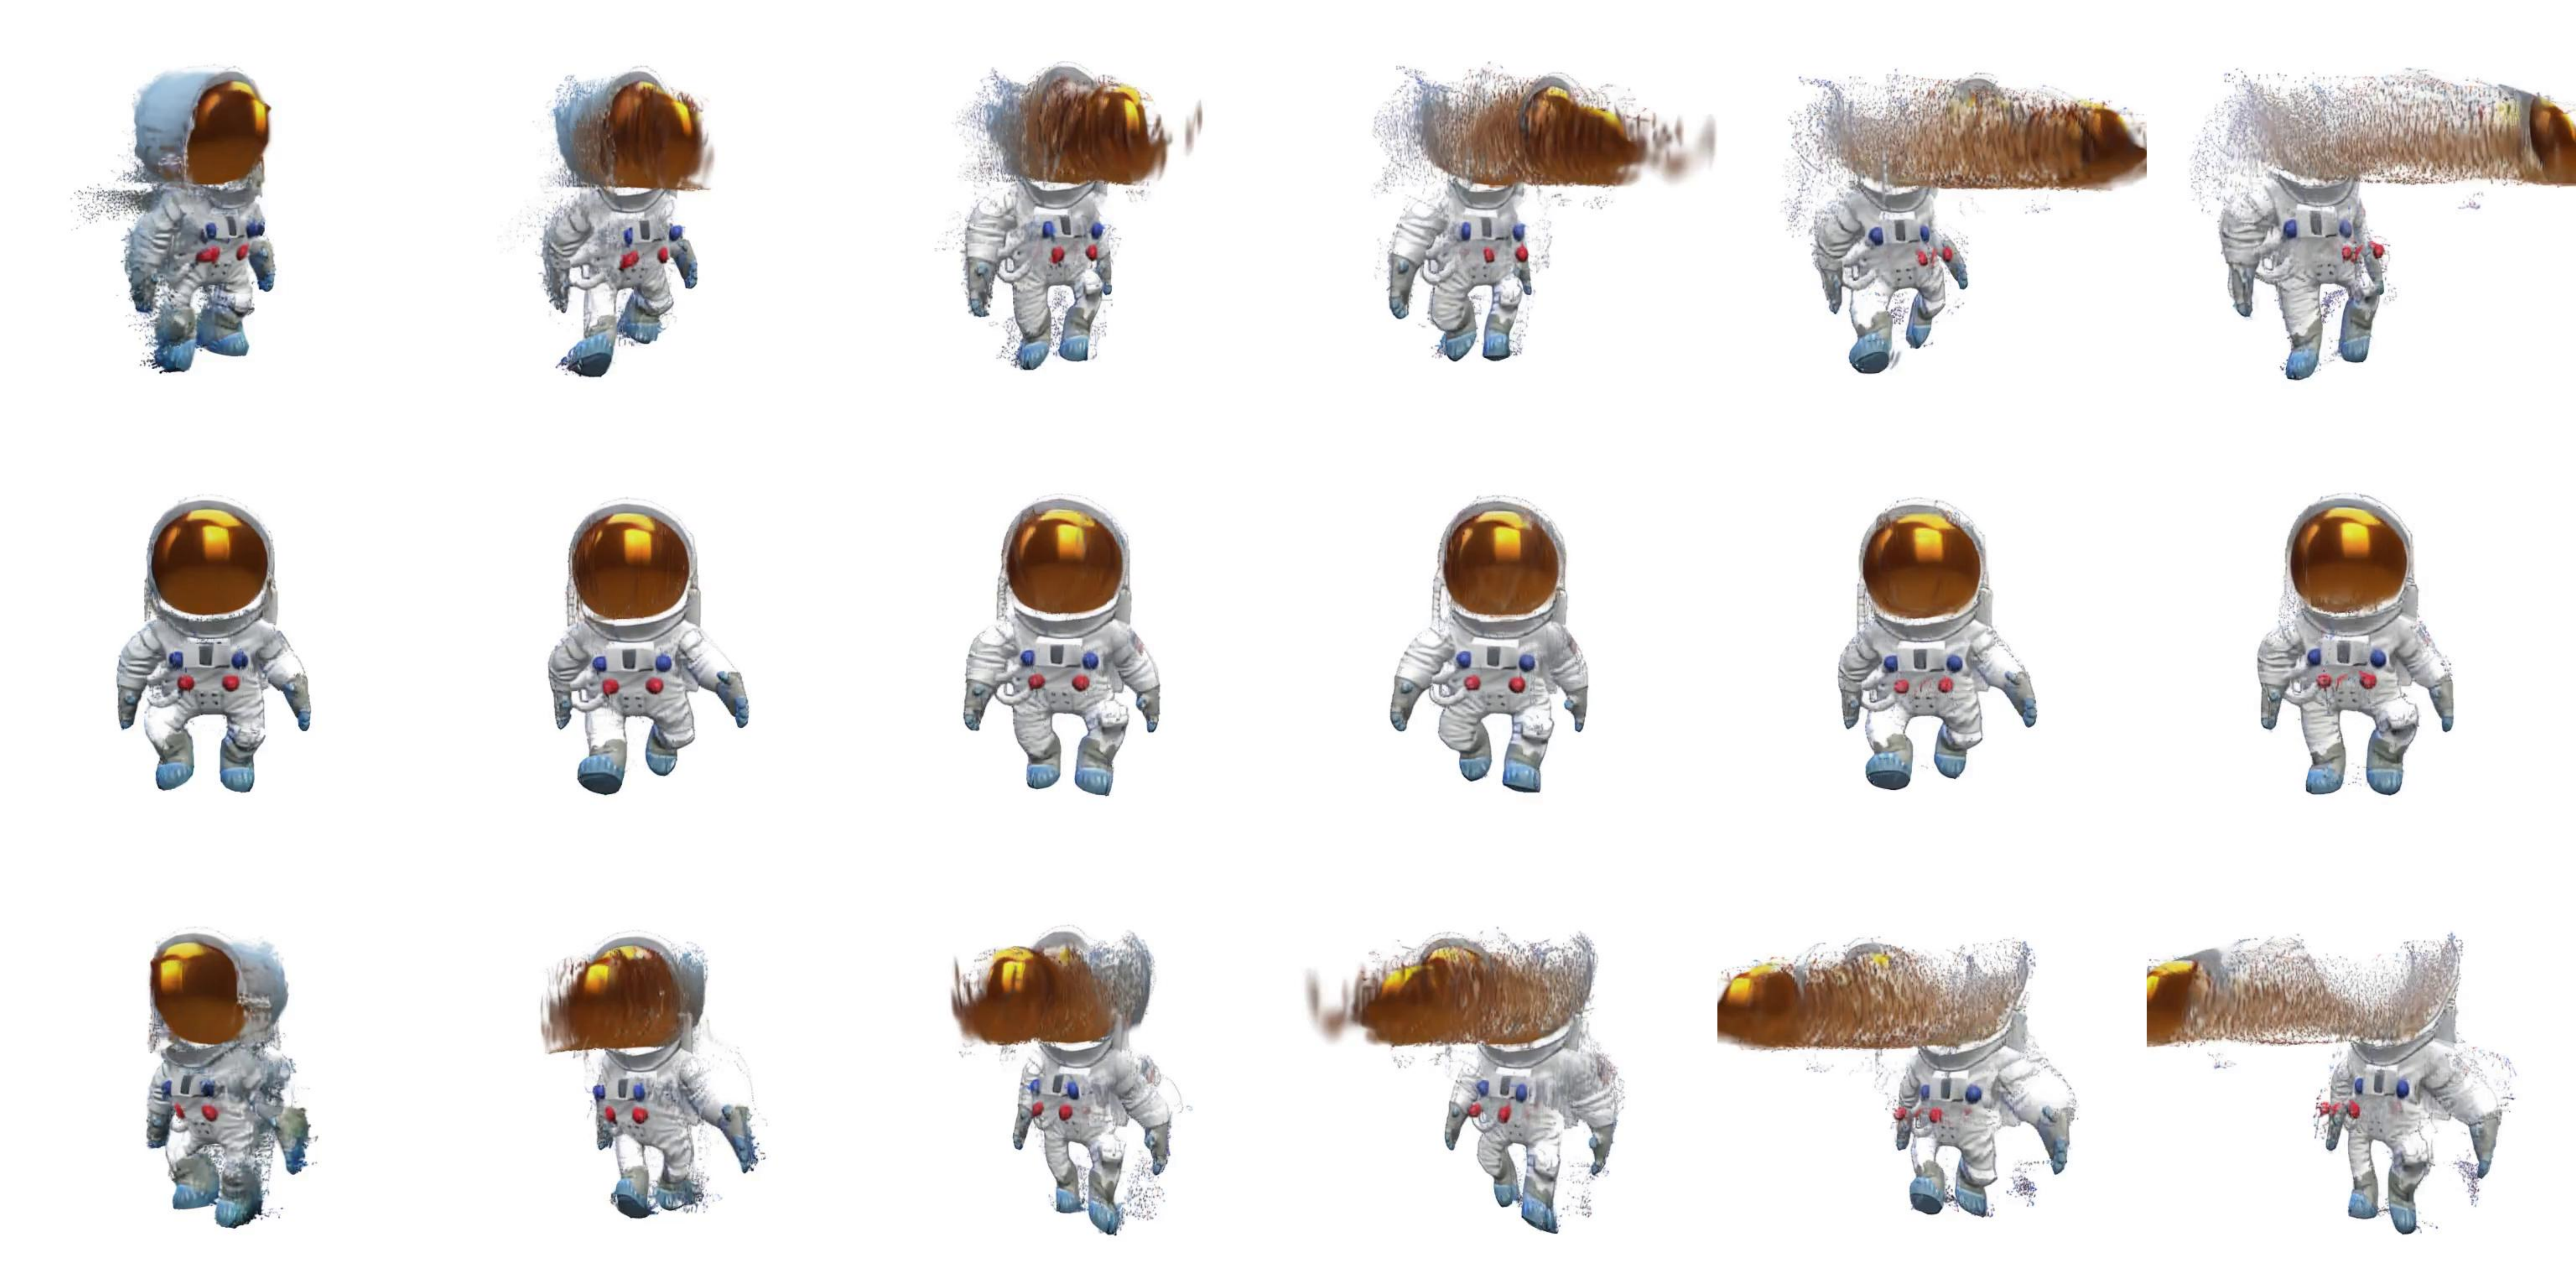}
        \caption{Multi-view videos rendered by autoregressive 4D generation alone.}
    \end{subfigure}
    \hfill
    \begin{subfigure}[b]{1\textwidth}
        \centering
        \includegraphics[width=0.82\textwidth]{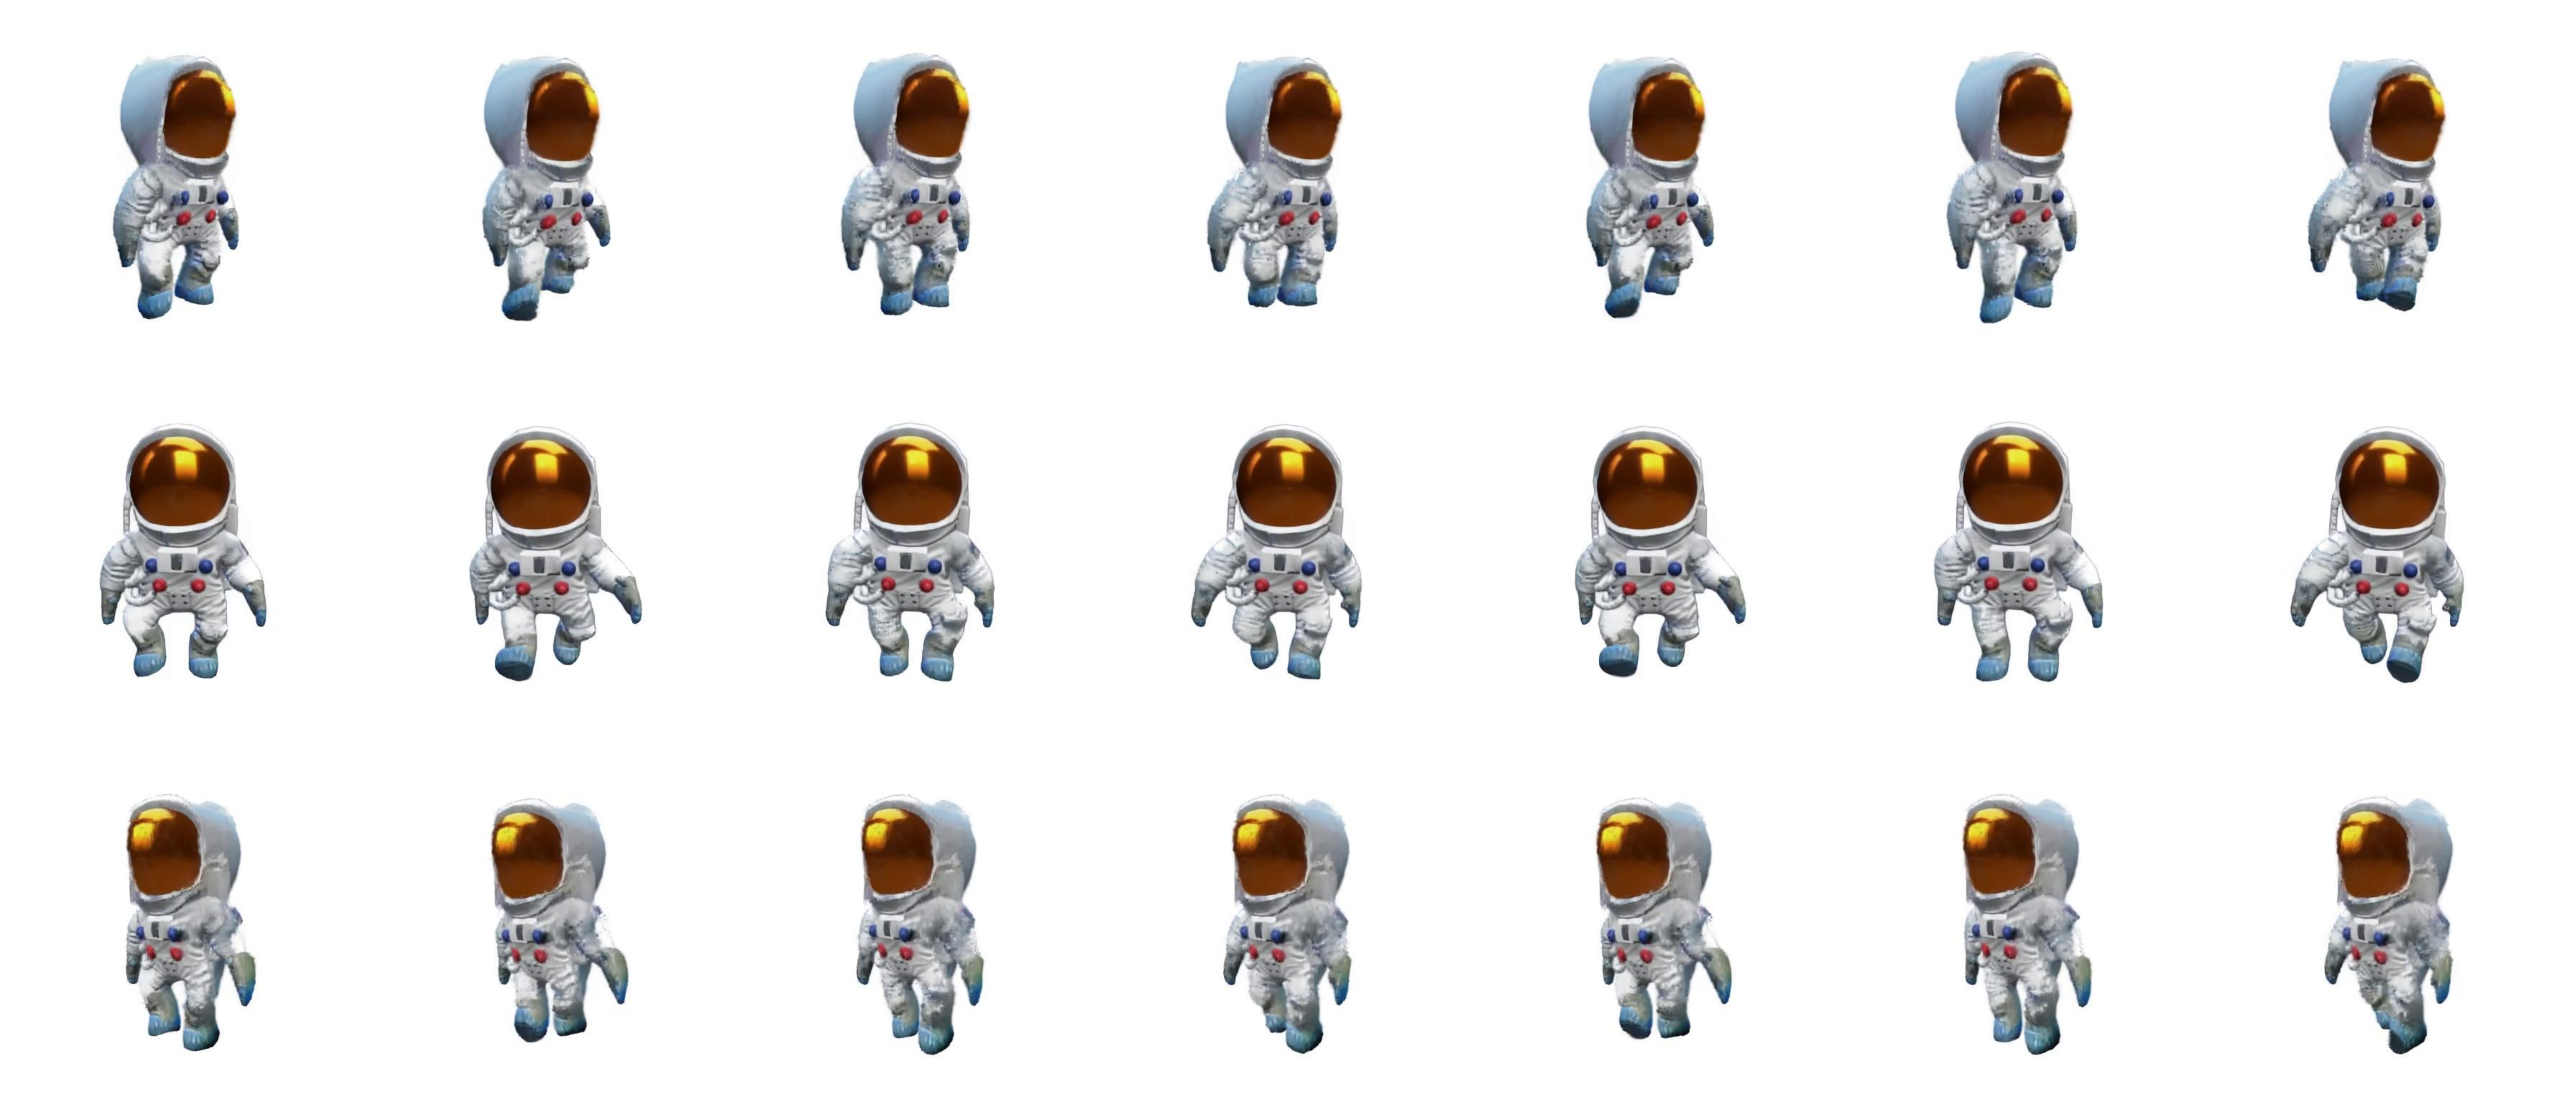}
        \caption{Multi-view videos rendered by autoregressive 4D generation with the progressive view sampling strategy.}
    \end{subfigure}
    \hfill
    \caption{Additional visualizations from the ablation studies on integrating autoregressive 4D generation and progressive view sampling strategy.}
    \label{fig:supply_ablation_1}
\end{figure*}

\begin{figure*}[t]
    \centering
    \begin{subfigure}[b]{1\textwidth}
        \centering
        \includegraphics[width=0.9\textwidth]{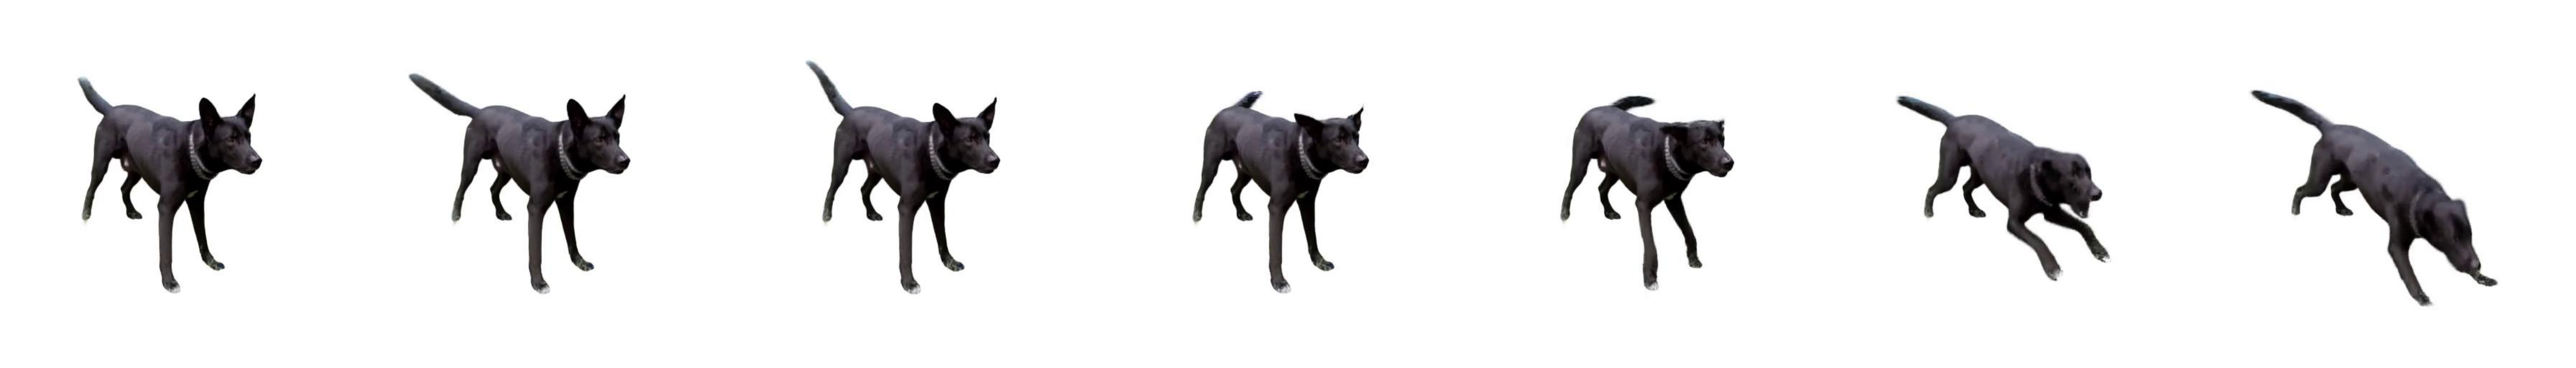}
        \caption{\textbf{Input monocular video.}}
    \end{subfigure}
    \hfill
    \begin{subfigure}[b]{1\textwidth}
        \centering
        \includegraphics[width=0.9\textwidth]{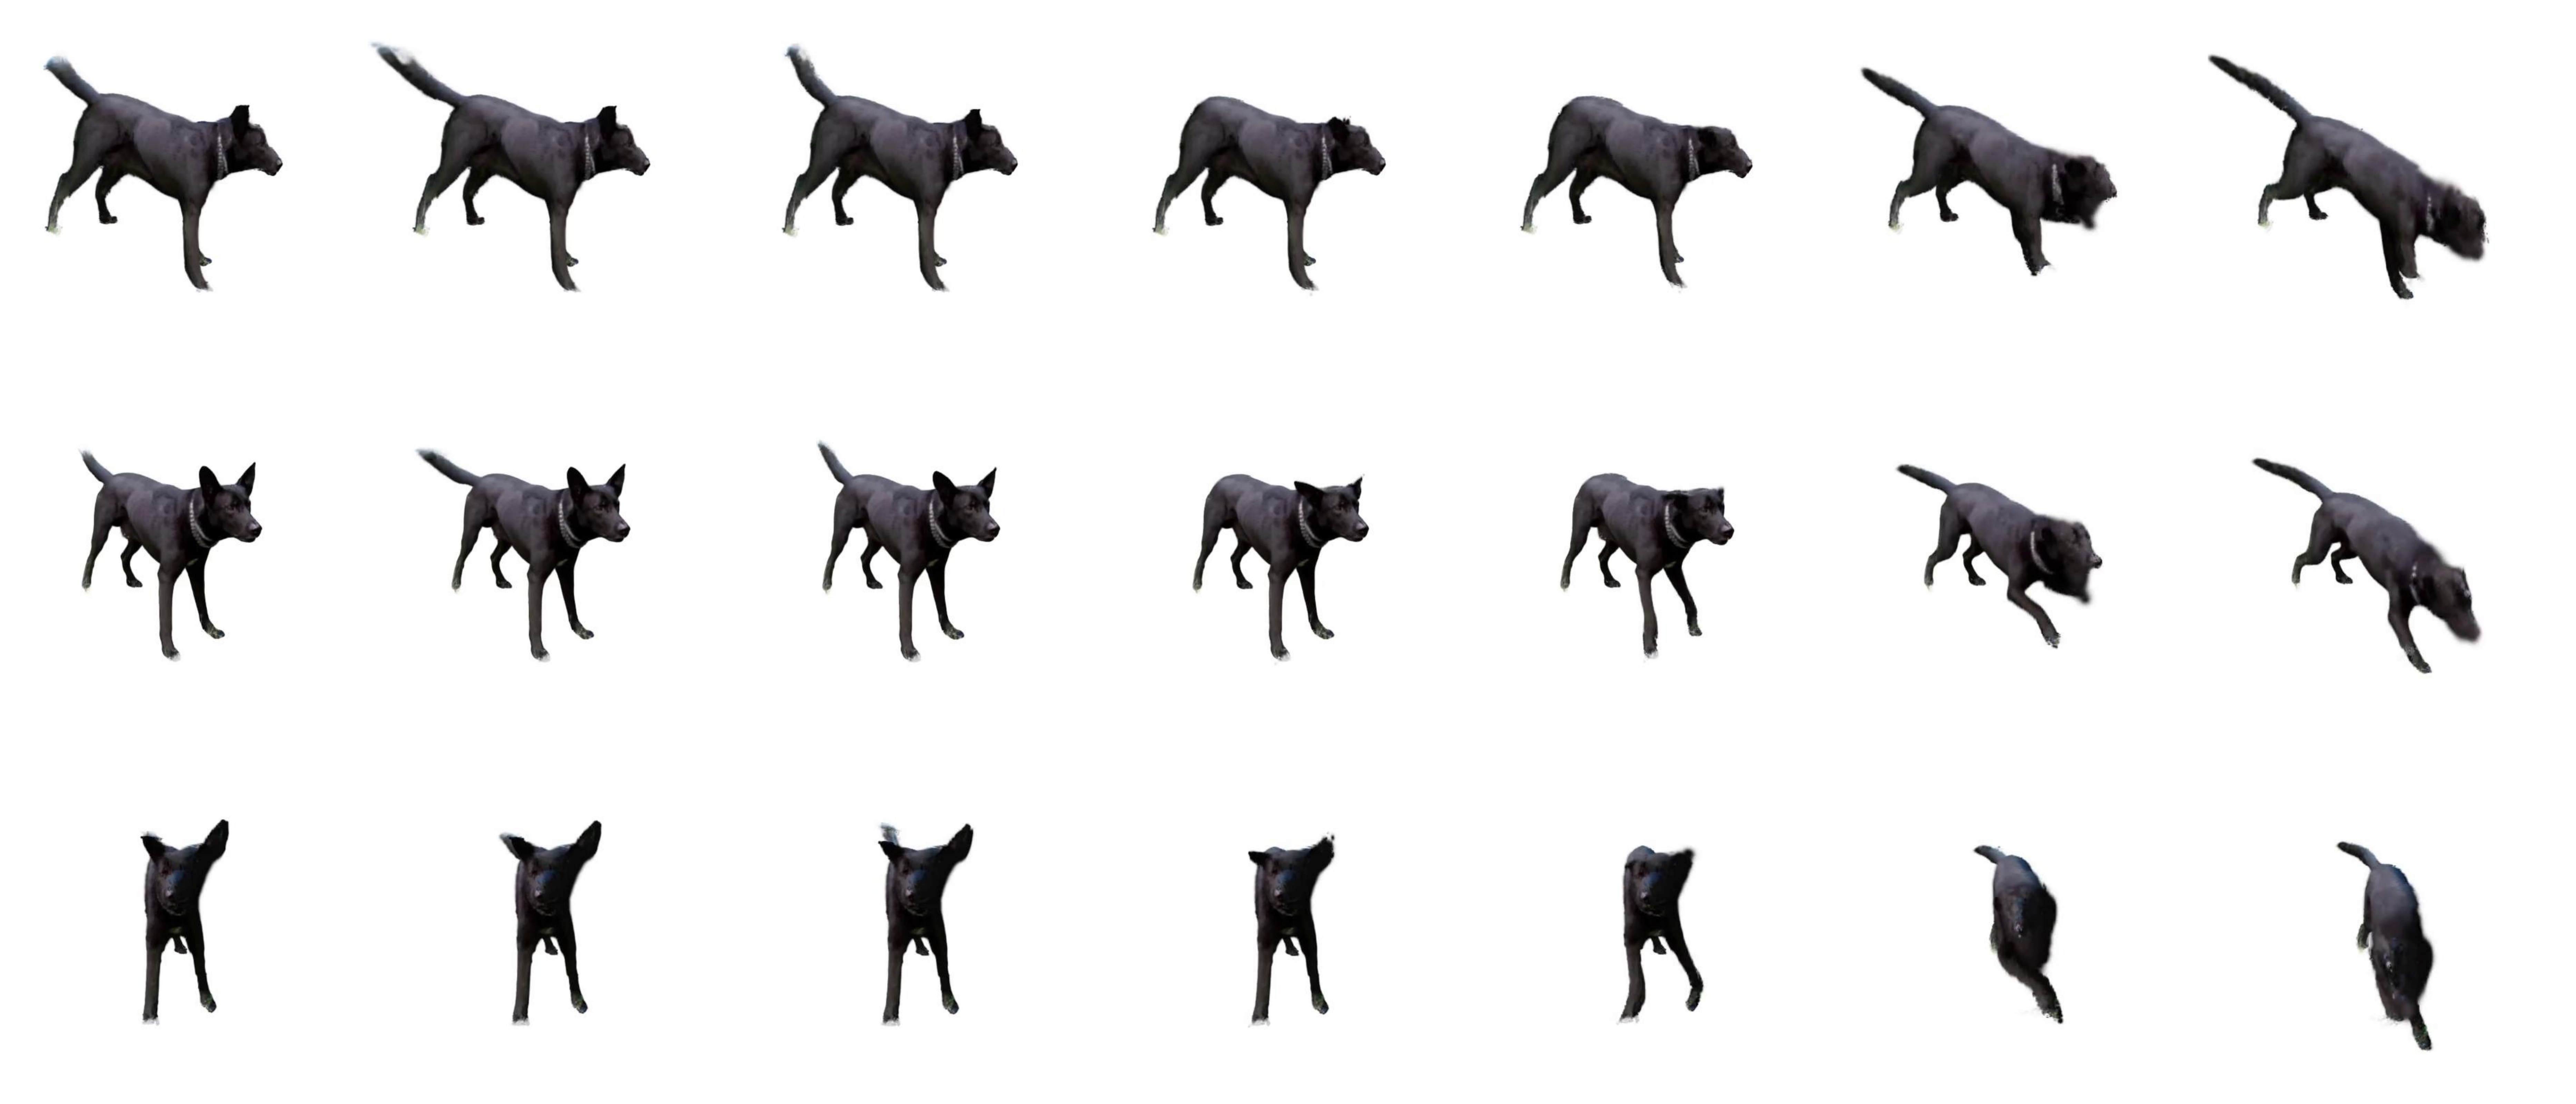}
        \caption{\textbf{Rendered multi-view videos without autoregressive generation:} precise motion estimation is challenging, especially for frames with substantial motion changes.}
    \end{subfigure}
    \hfill
    \begin{subfigure}[b]{1\textwidth}
        \centering
        \includegraphics[width=0.9\textwidth]{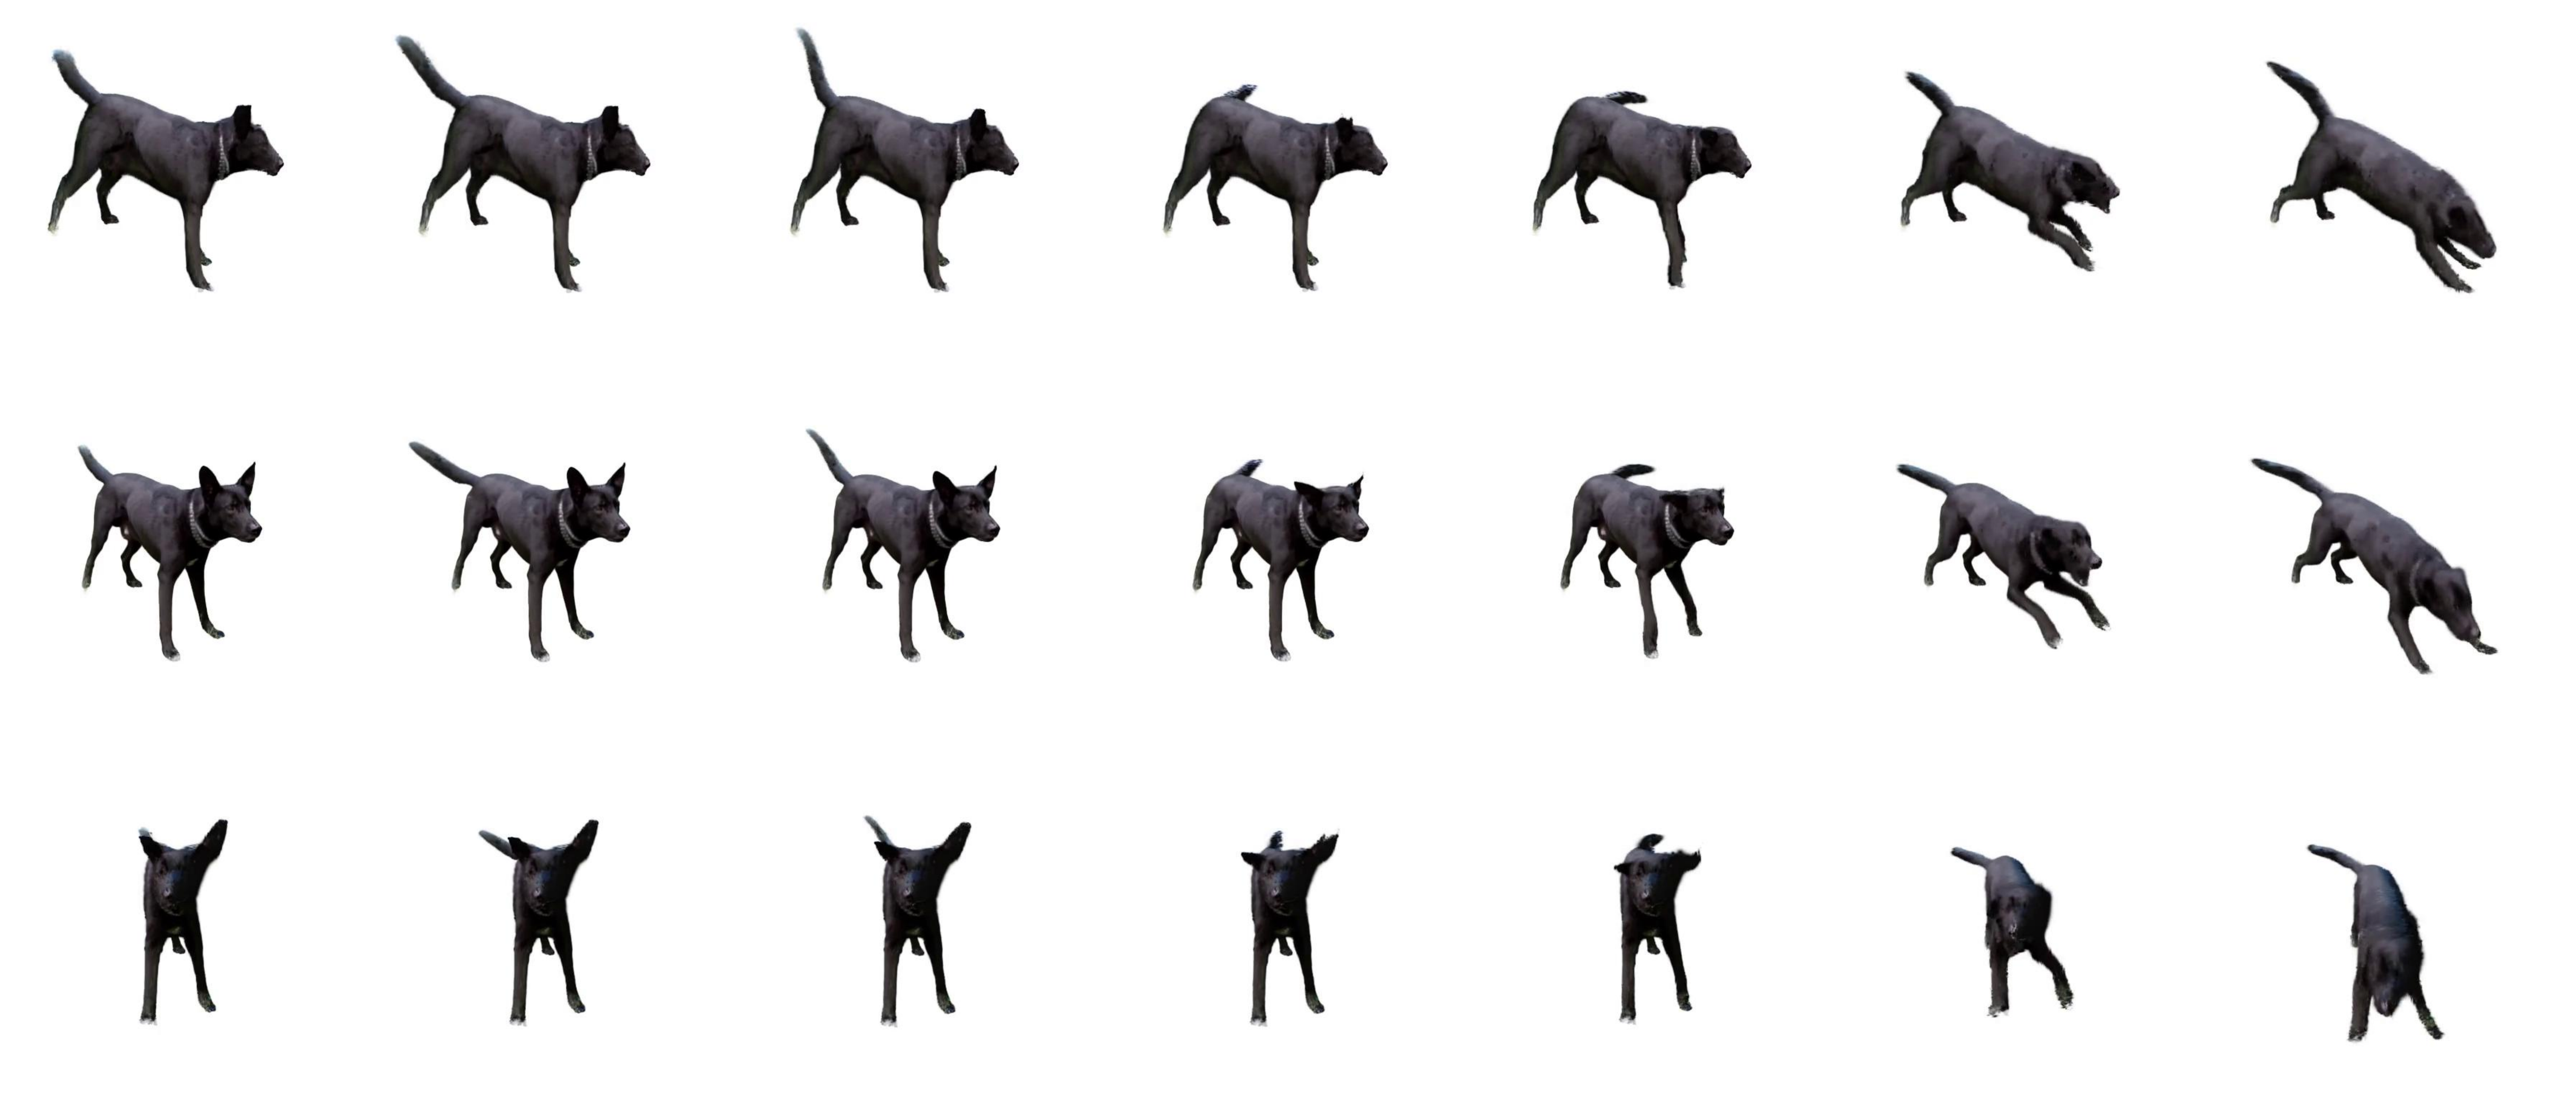}
        \caption{\textbf{Rendered multi-view videos with autoregressive generation:} incorporating autoregressive generation enhances motion and geometry estimation, leading to more accurate and consistent results.}
    \end{subfigure}
    \hfill
    \caption{More visualizations of ablation studies on whether incorporating autoregressive generation.}
    \label{fig:supply_ablation_2}
\end{figure*}

\begin{figure*}[t]
    \centering
    \begin{subfigure}[b]{1\textwidth}
        \centering
        \includegraphics[width=0.9\textwidth]{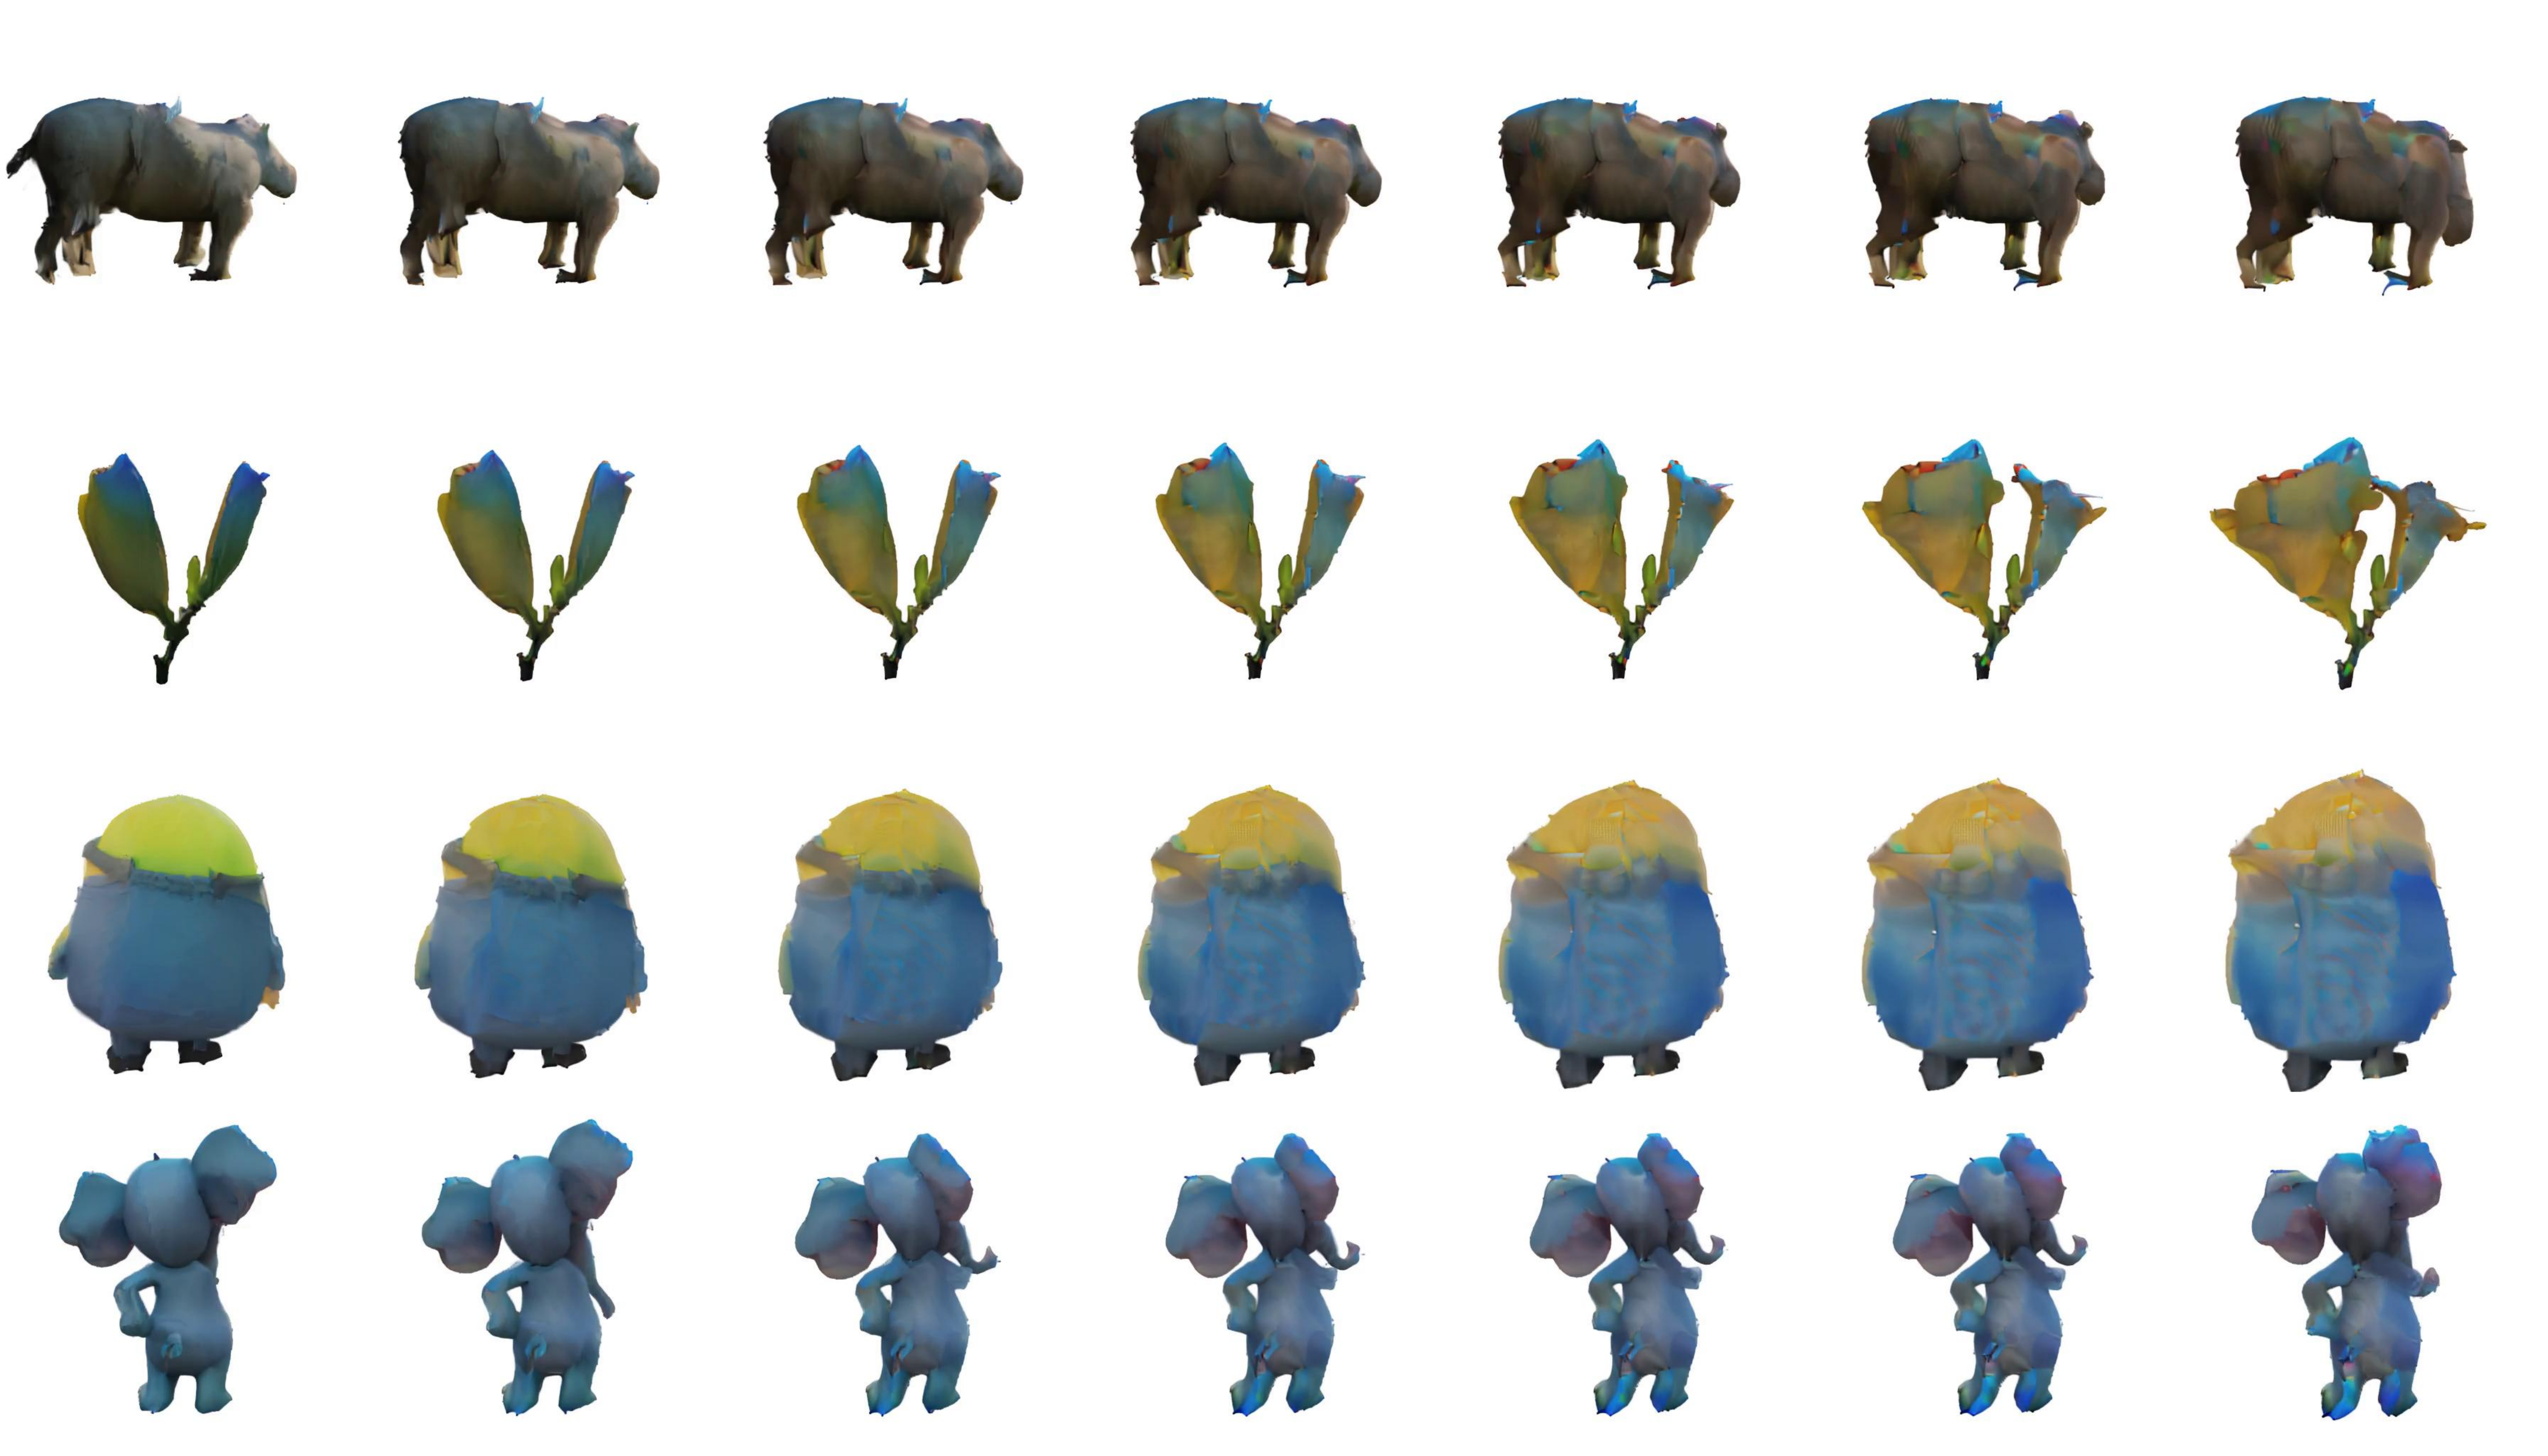}
        \caption{Results obtained without the refinement stage, obvious appearance drift can be observed.}
    \end{subfigure}
    \hfill
    \begin{subfigure}[b]{1\textwidth}
        \centering
        \includegraphics[width=0.9\textwidth]{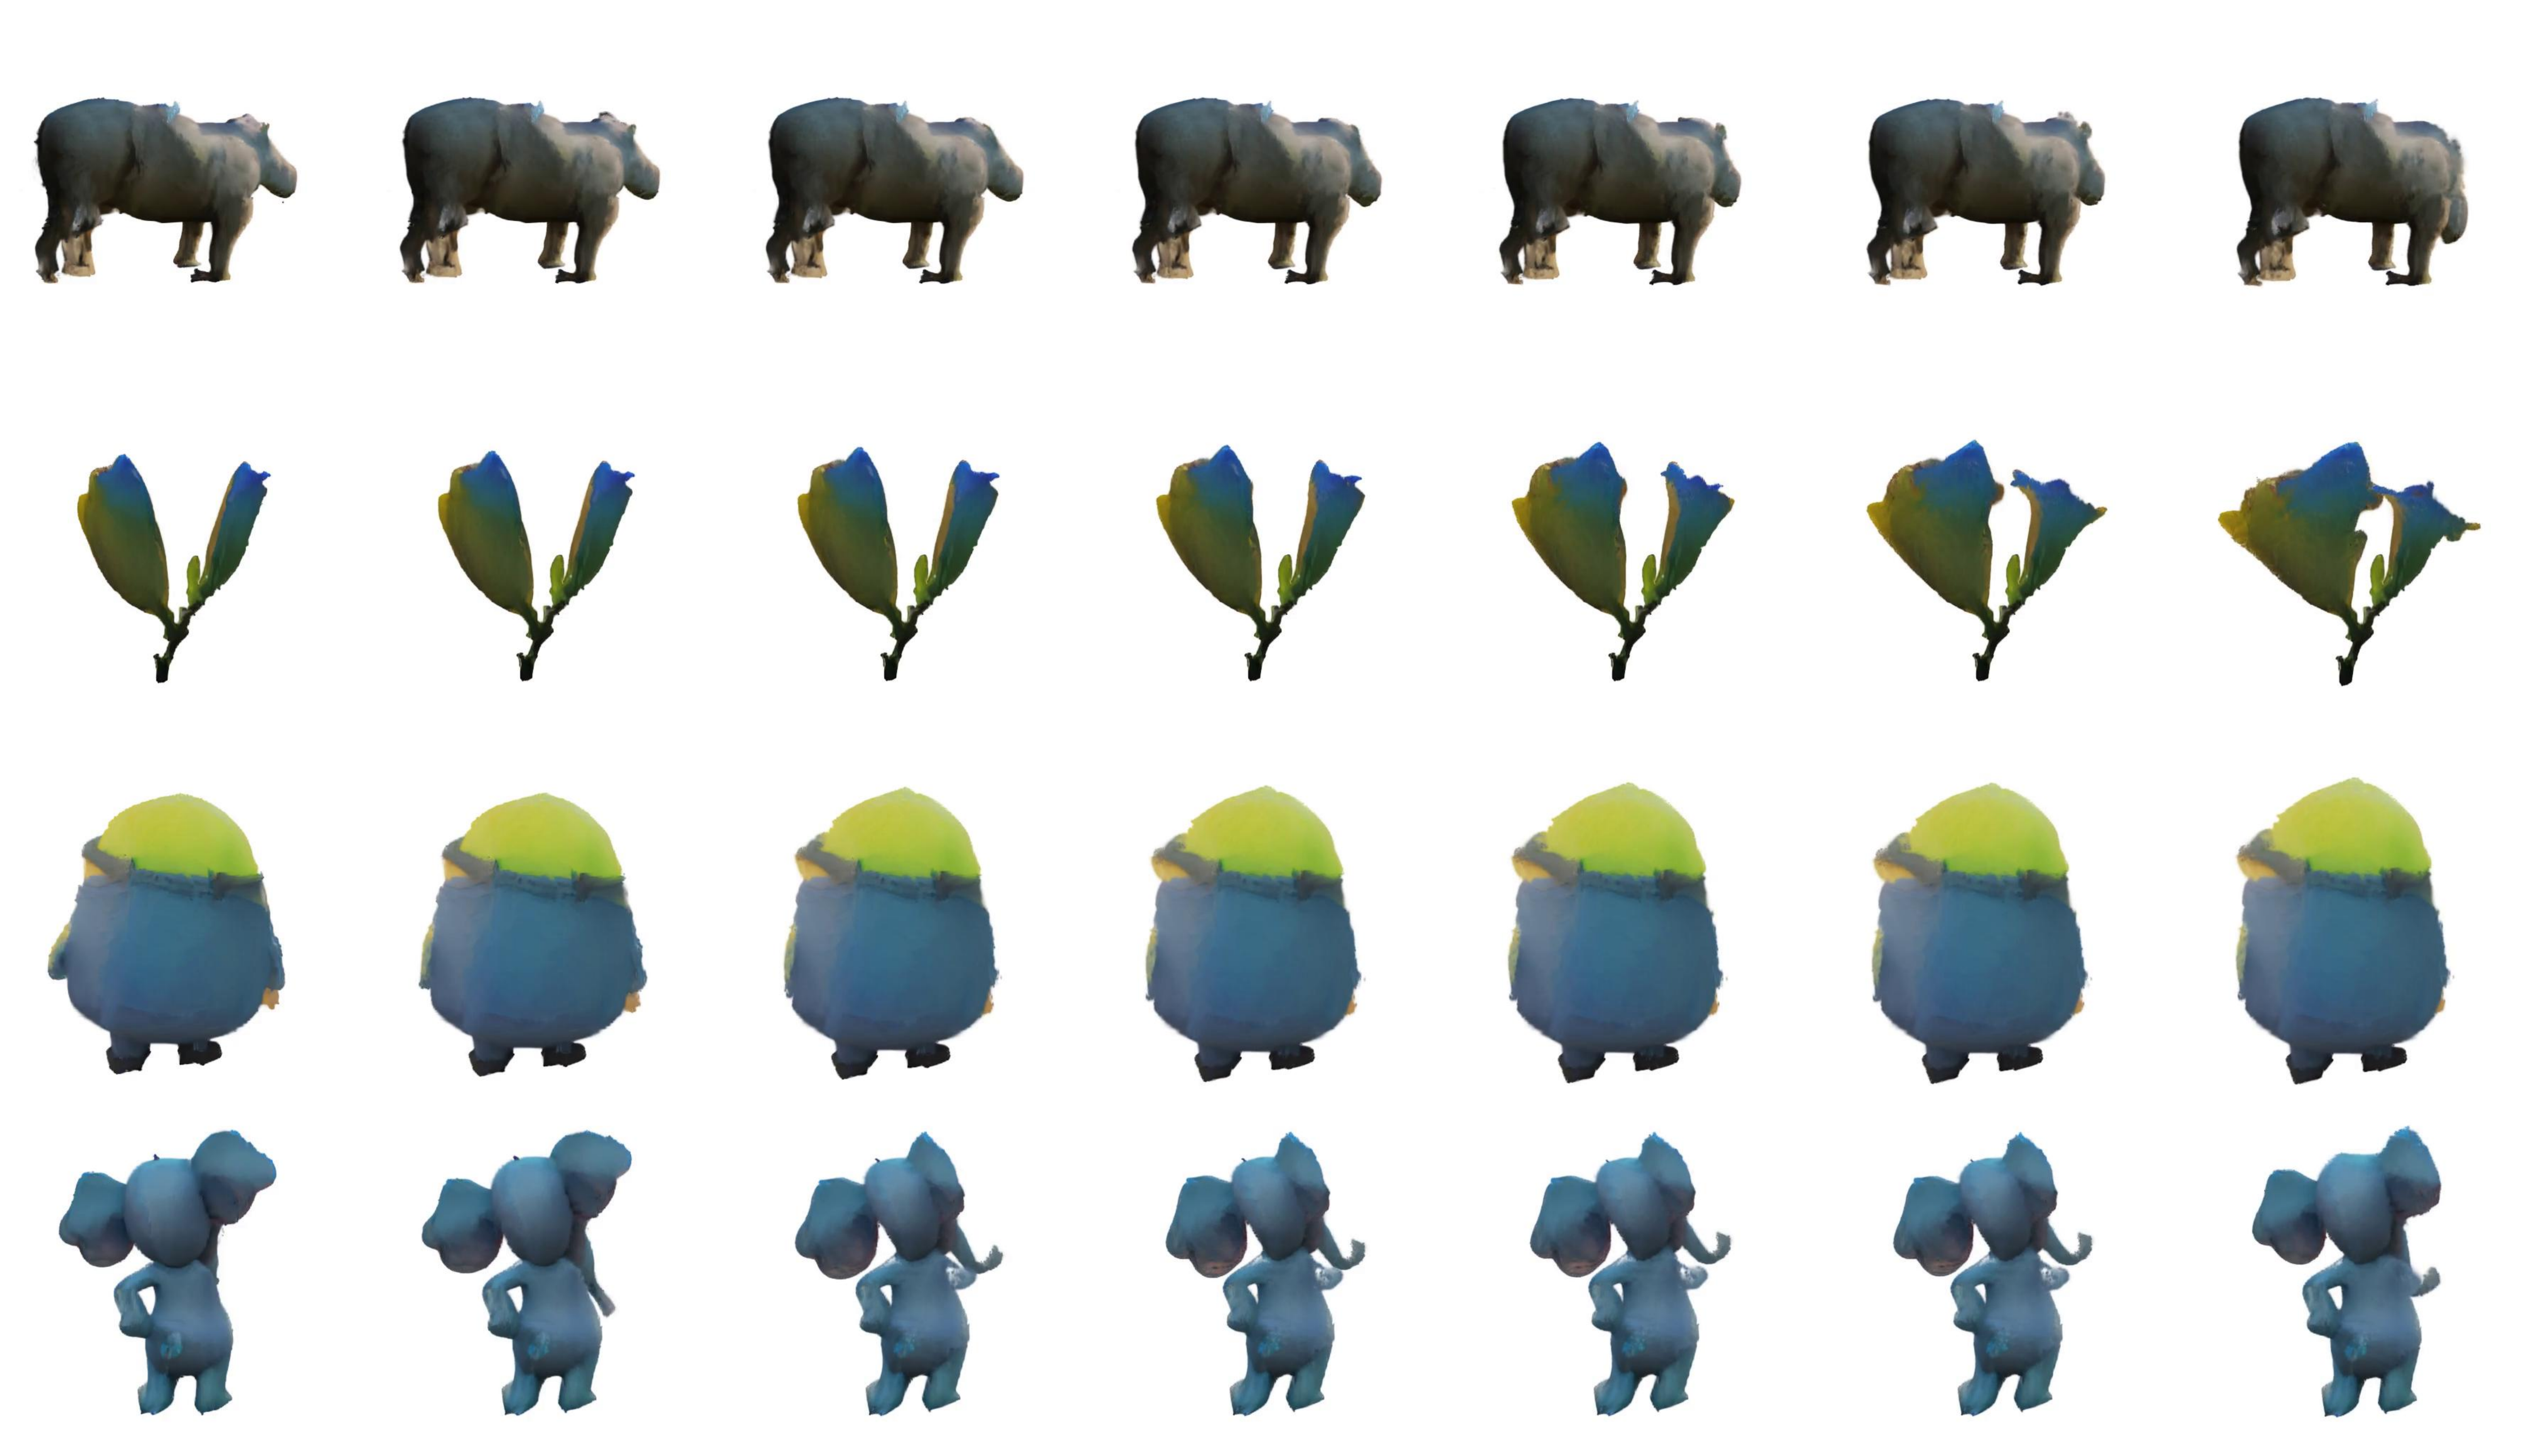}
        \caption{With the refinement stage, appearance drift can be addressed, leading to results with better spatial-temporal consistency.}
    \end{subfigure}0
    \hfill
    \caption{More visualizations of ablation studies on whether incorporating the refinement stage.}
    \label{fig:supply_ablation_3}
\end{figure*}

\section{More visualizations of comparisons with state-of-the-art methods}\label{More visualizations of comparisons with state-of-the-art method}
In this section, we present additional detailed visual comparisons between our proposed method and other state-of-the-art approaches. As demonstrated in Fig.~\ref{fig:supply_compaisons_1}, Fig.~\ref{fig:supply_compaisons_2} and Fig.~\ref{fig:supply_compaisons_4}, Consistent4D~\cite{jiang2023consistent4d} tends to produce over-saturated outputs due to the limitations of SDS, while SV4D~\cite{xie2024sv4d} results in overly blurred outputs due to domain gap issues. By integrating the ideas of Consistent4D and SV4D, where anchor multi-view sequences are first generated through a multi-view diffusion model followed by SDS-based refinement, STAG4D~\cite{zeng2025stag4d} achieves improved results. However, it still exhibits noticeable noise and unrealistic patterns. Moreover, due to limitations in the training datasets, both SV4D and STAG4D struggle to generate 4D objects from longer input videos, hindering their practical applications. In comparison, our proposed AR4D achieves clearer renderings, enhanced spatial-temporal consistency, and improved alignment with input prompts.

\begin{figure*}[t]
    \centering
    \begin{subfigure}[b]{1\textwidth}
        \centering
        \includegraphics[width=0.85\textwidth]{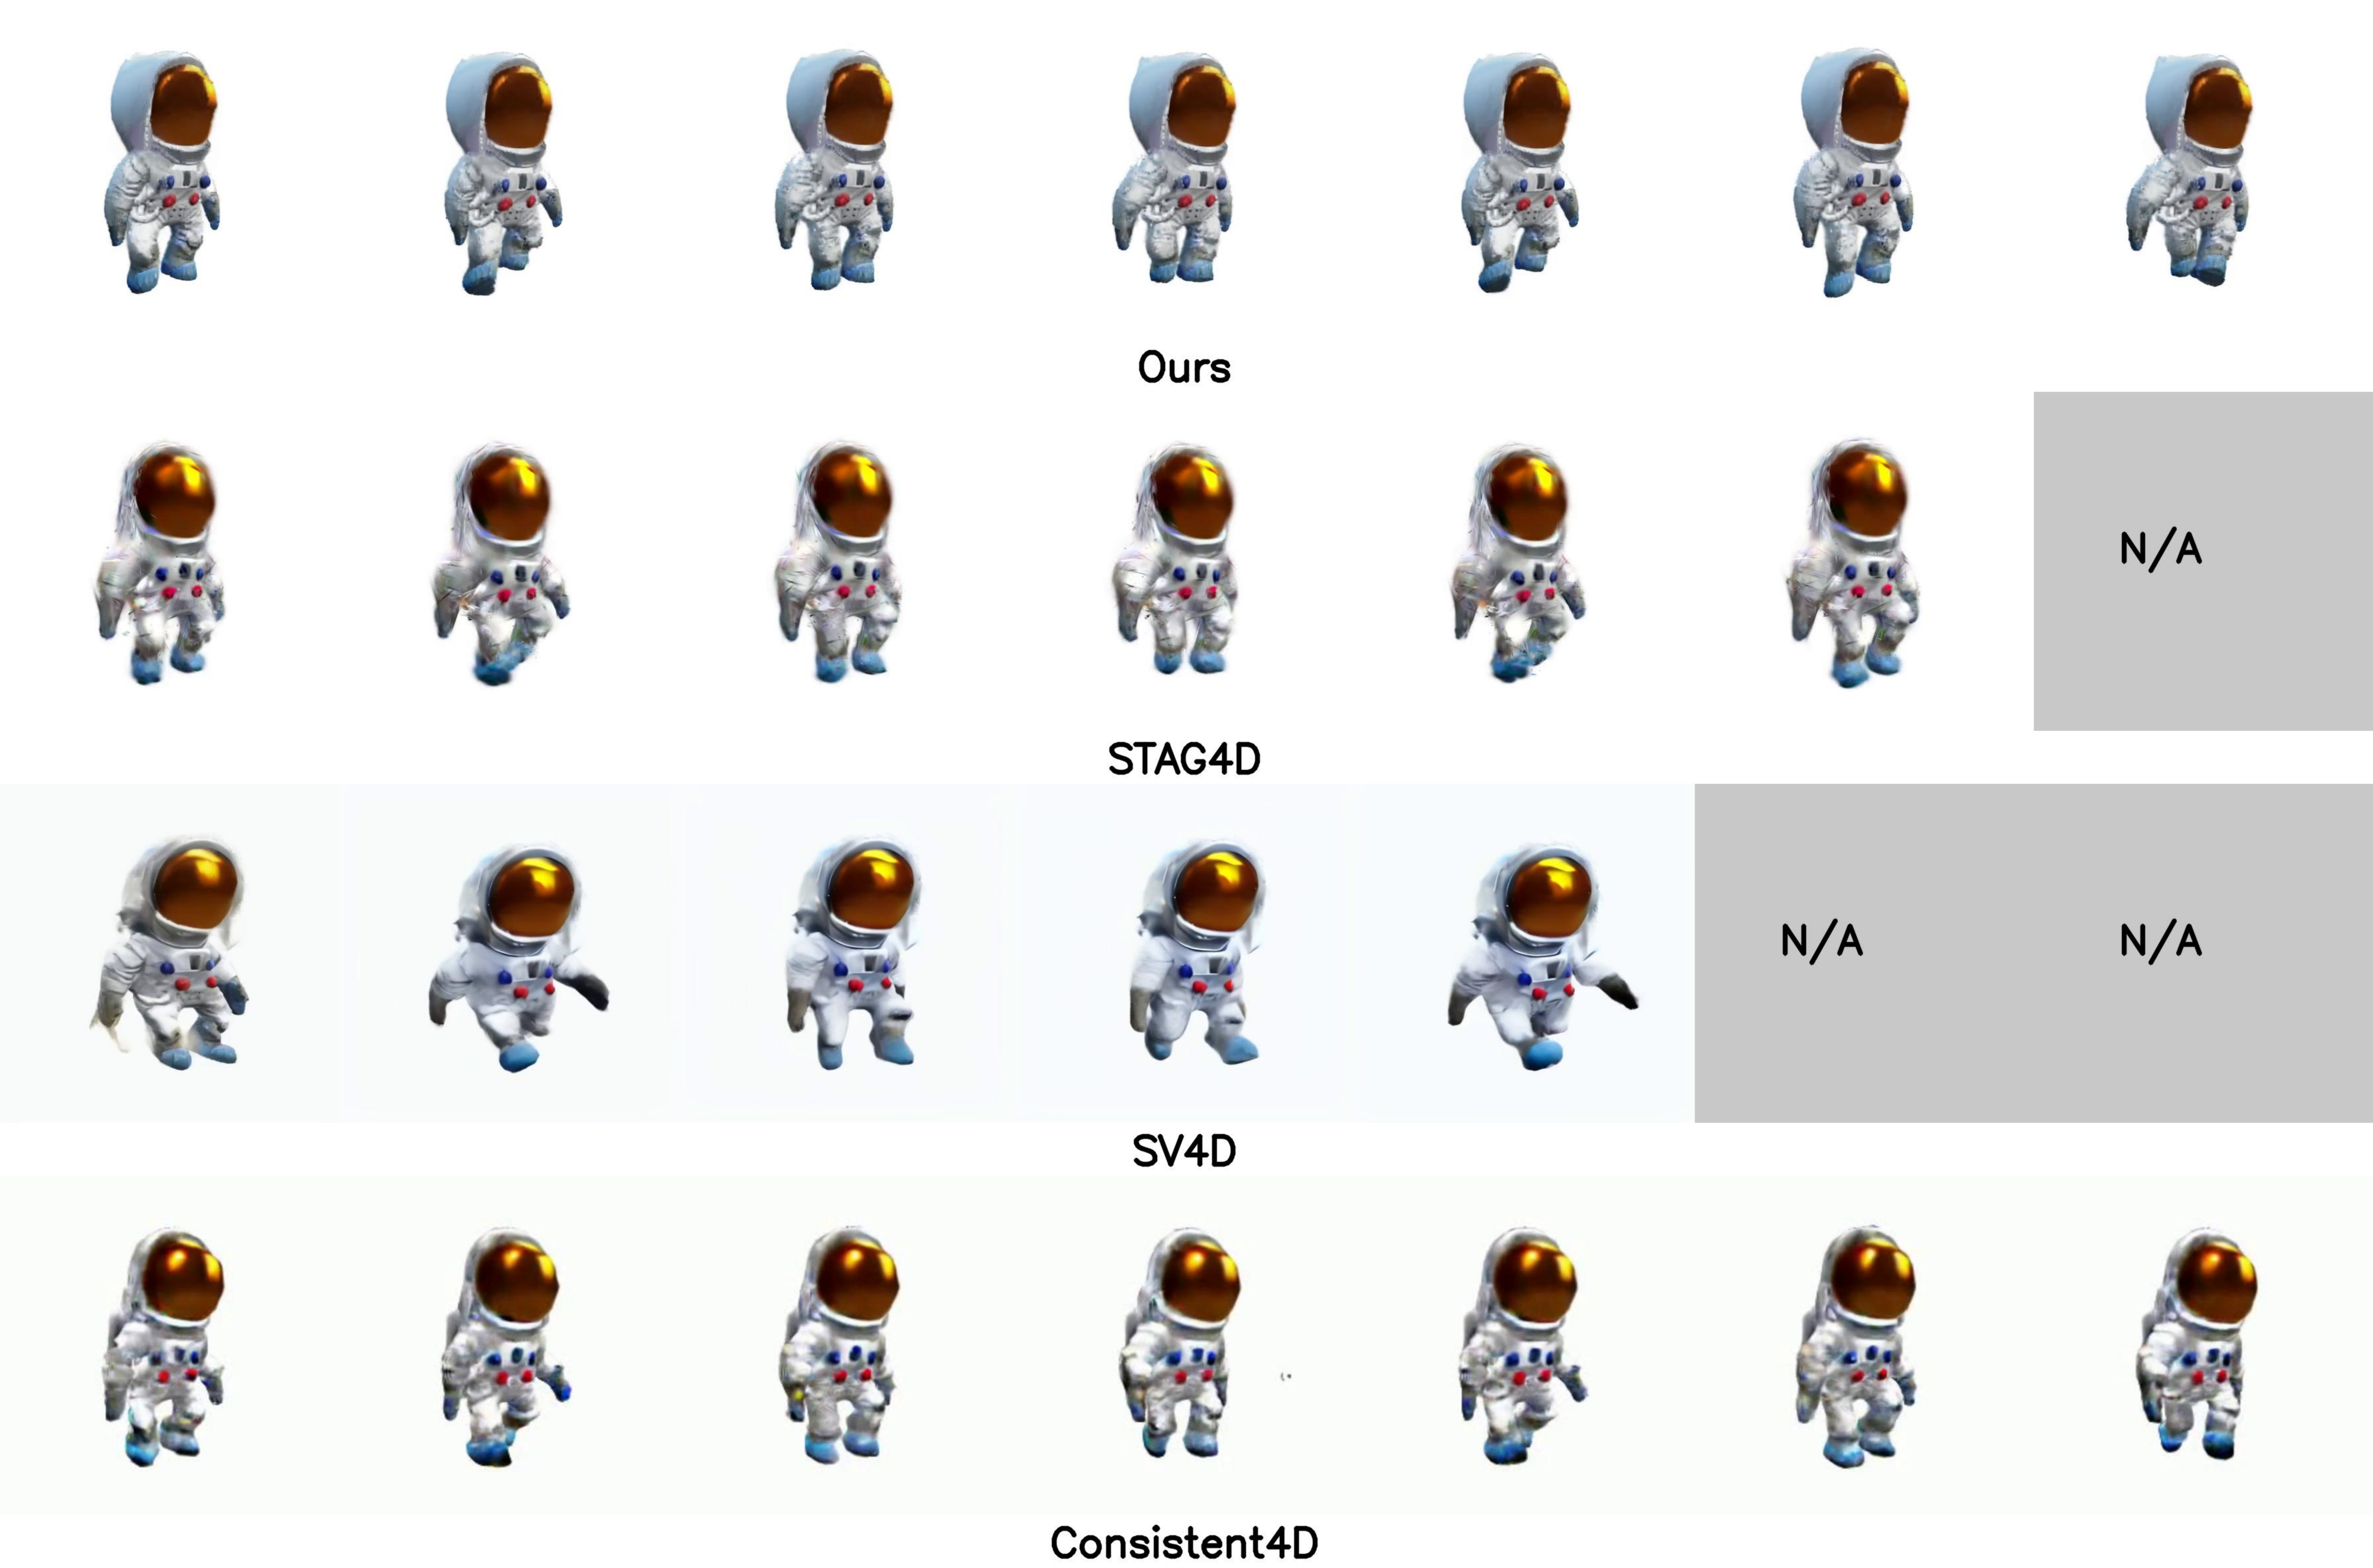}
        \caption{Comparison of novel-view videos rendered by our method and other state-of-the-art methods at novel view 1.}
    \end{subfigure}
    \hfill
    \begin{subfigure}[b]{1\textwidth}
        \centering
        \includegraphics[width=0.85\textwidth]{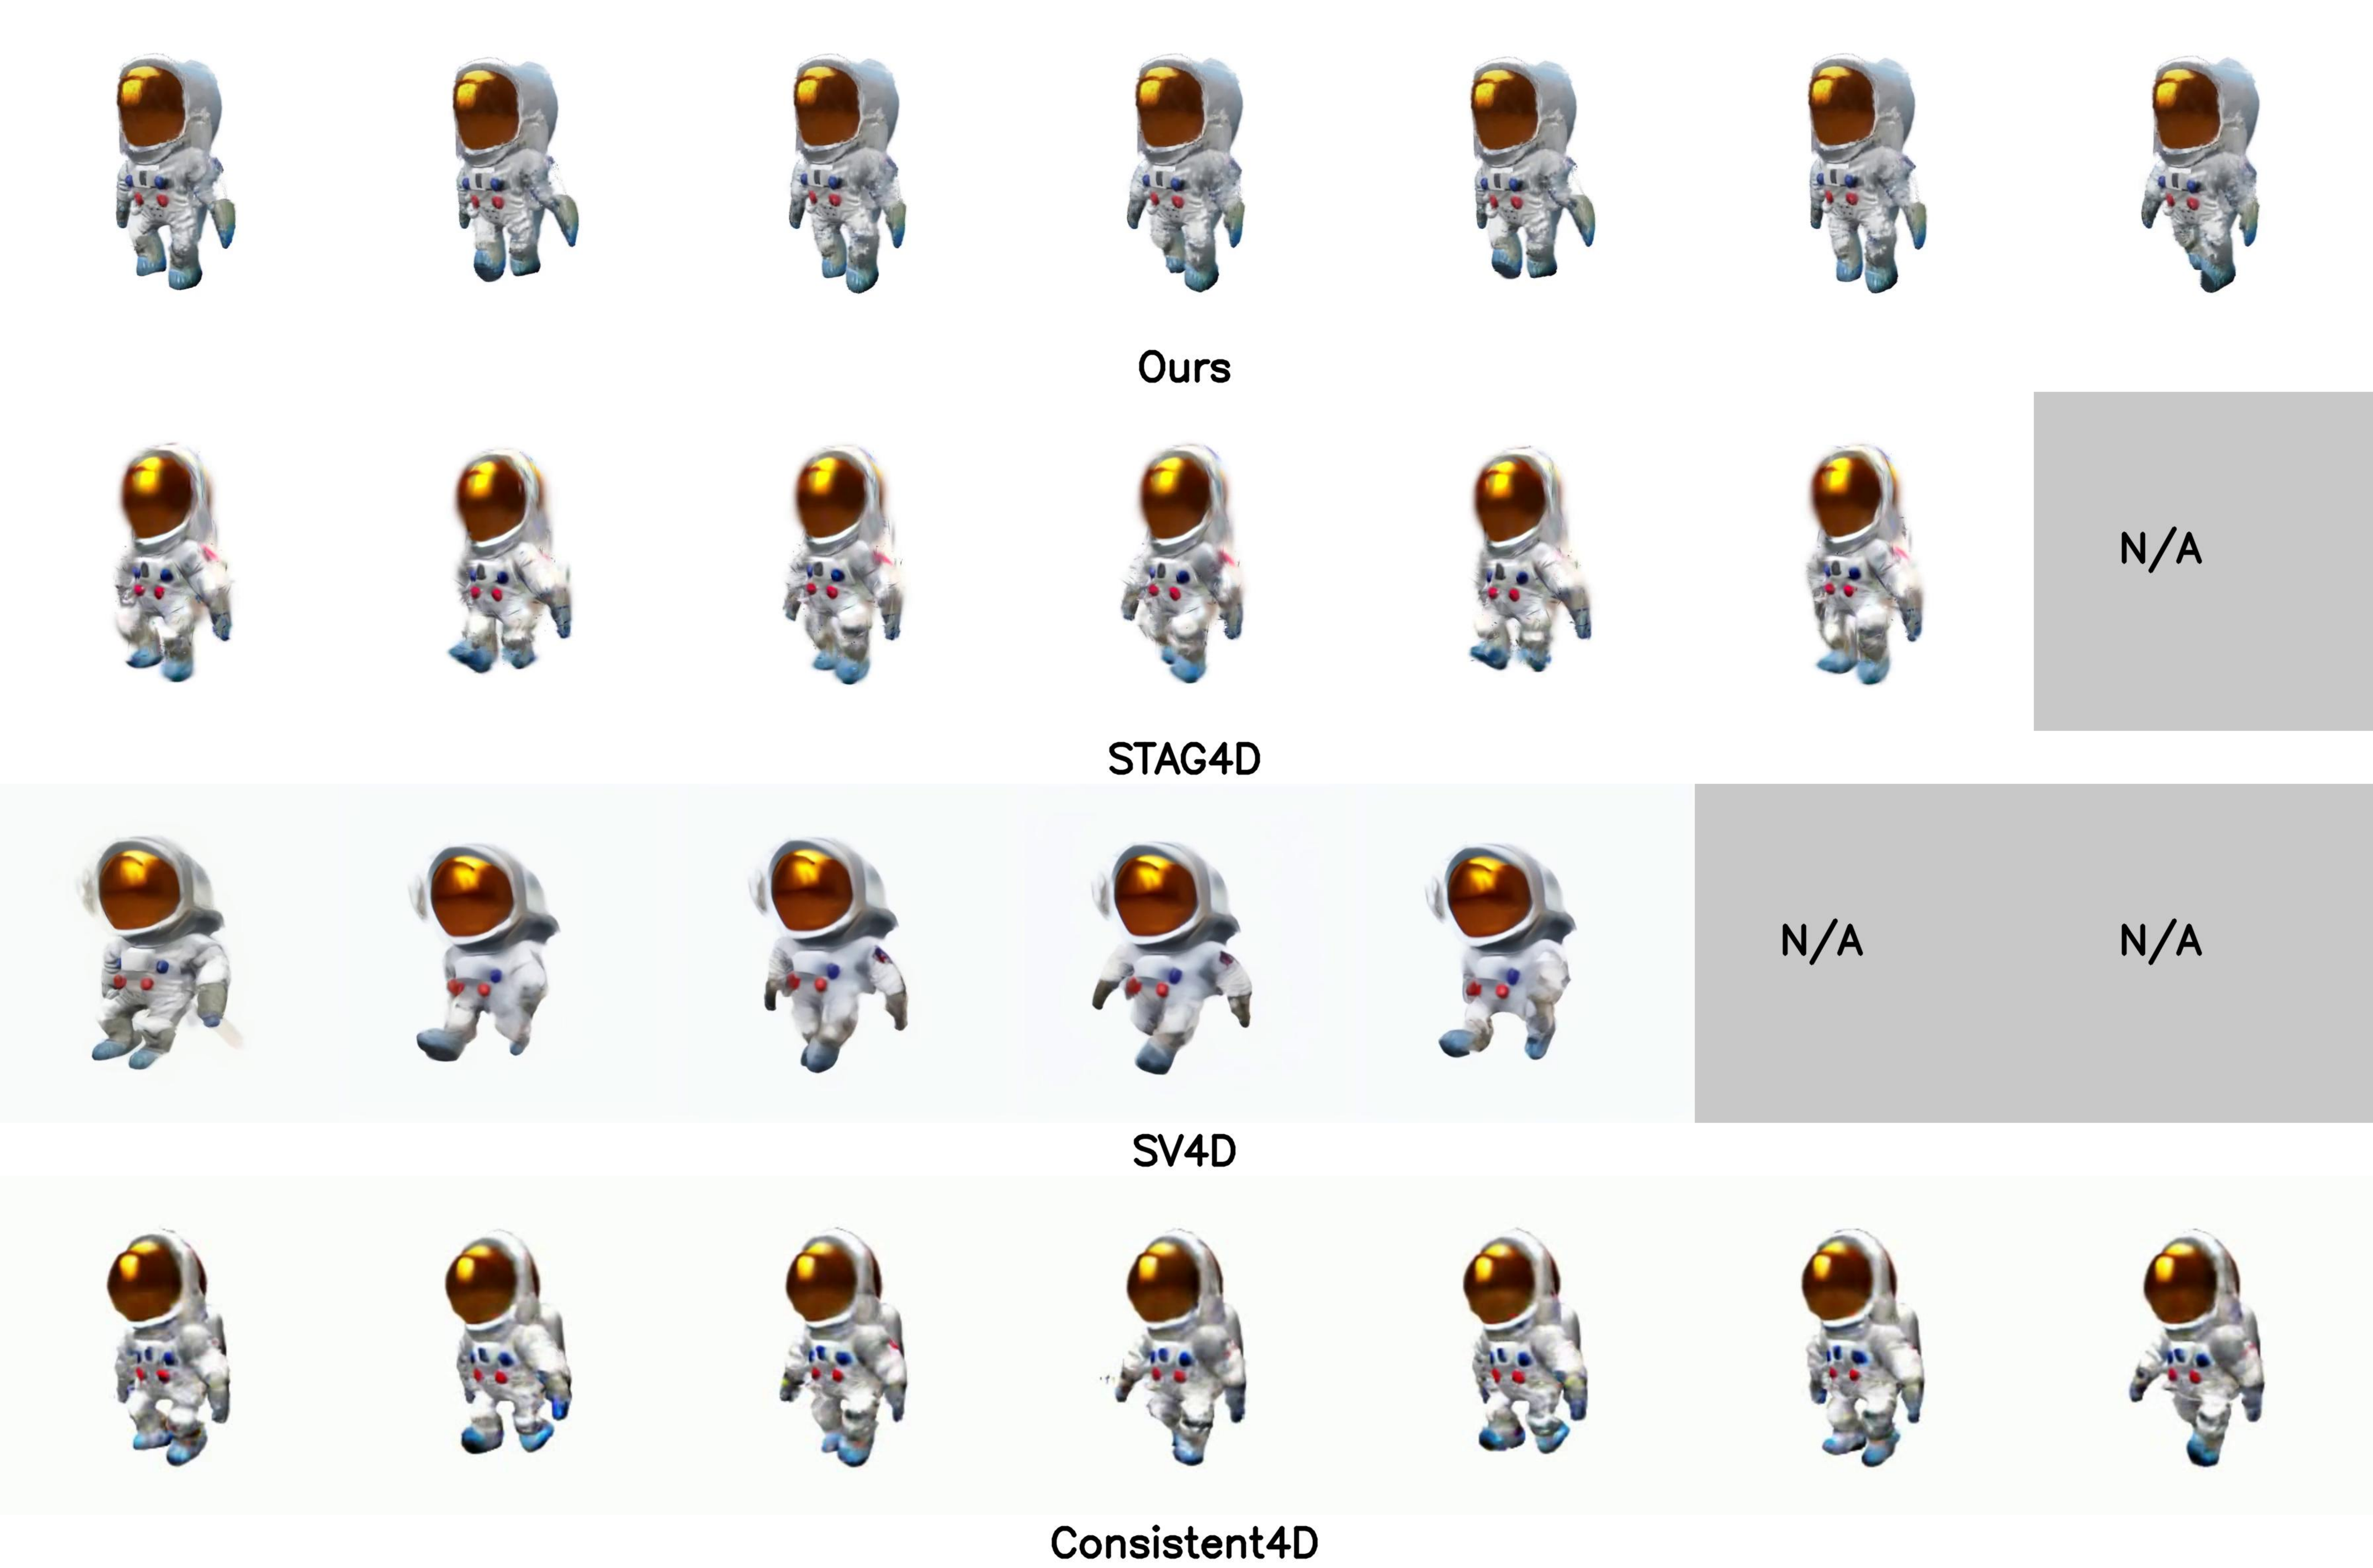}
        \caption{Comparison of novel-view videos rendered by our method and other state-of-the-art methods at novel view 2.}
    \end{subfigure}
    \hfill
    \caption{More visualizations of comparison of novel-view videos rendered by our method and other state-of-the-art methods at different novel views on the task of Video-to-4D. $\textbf{\textit{N/A}}$ indicates that the corresponding method fails to generate novel views for the current frame.
}
    \label{fig:supply_compaisons_1}
\end{figure*}

\begin{figure*}[t]
    \centering
    \begin{subfigure}[b]{1\textwidth}
        \centering
        \includegraphics[width=0.85\textwidth]{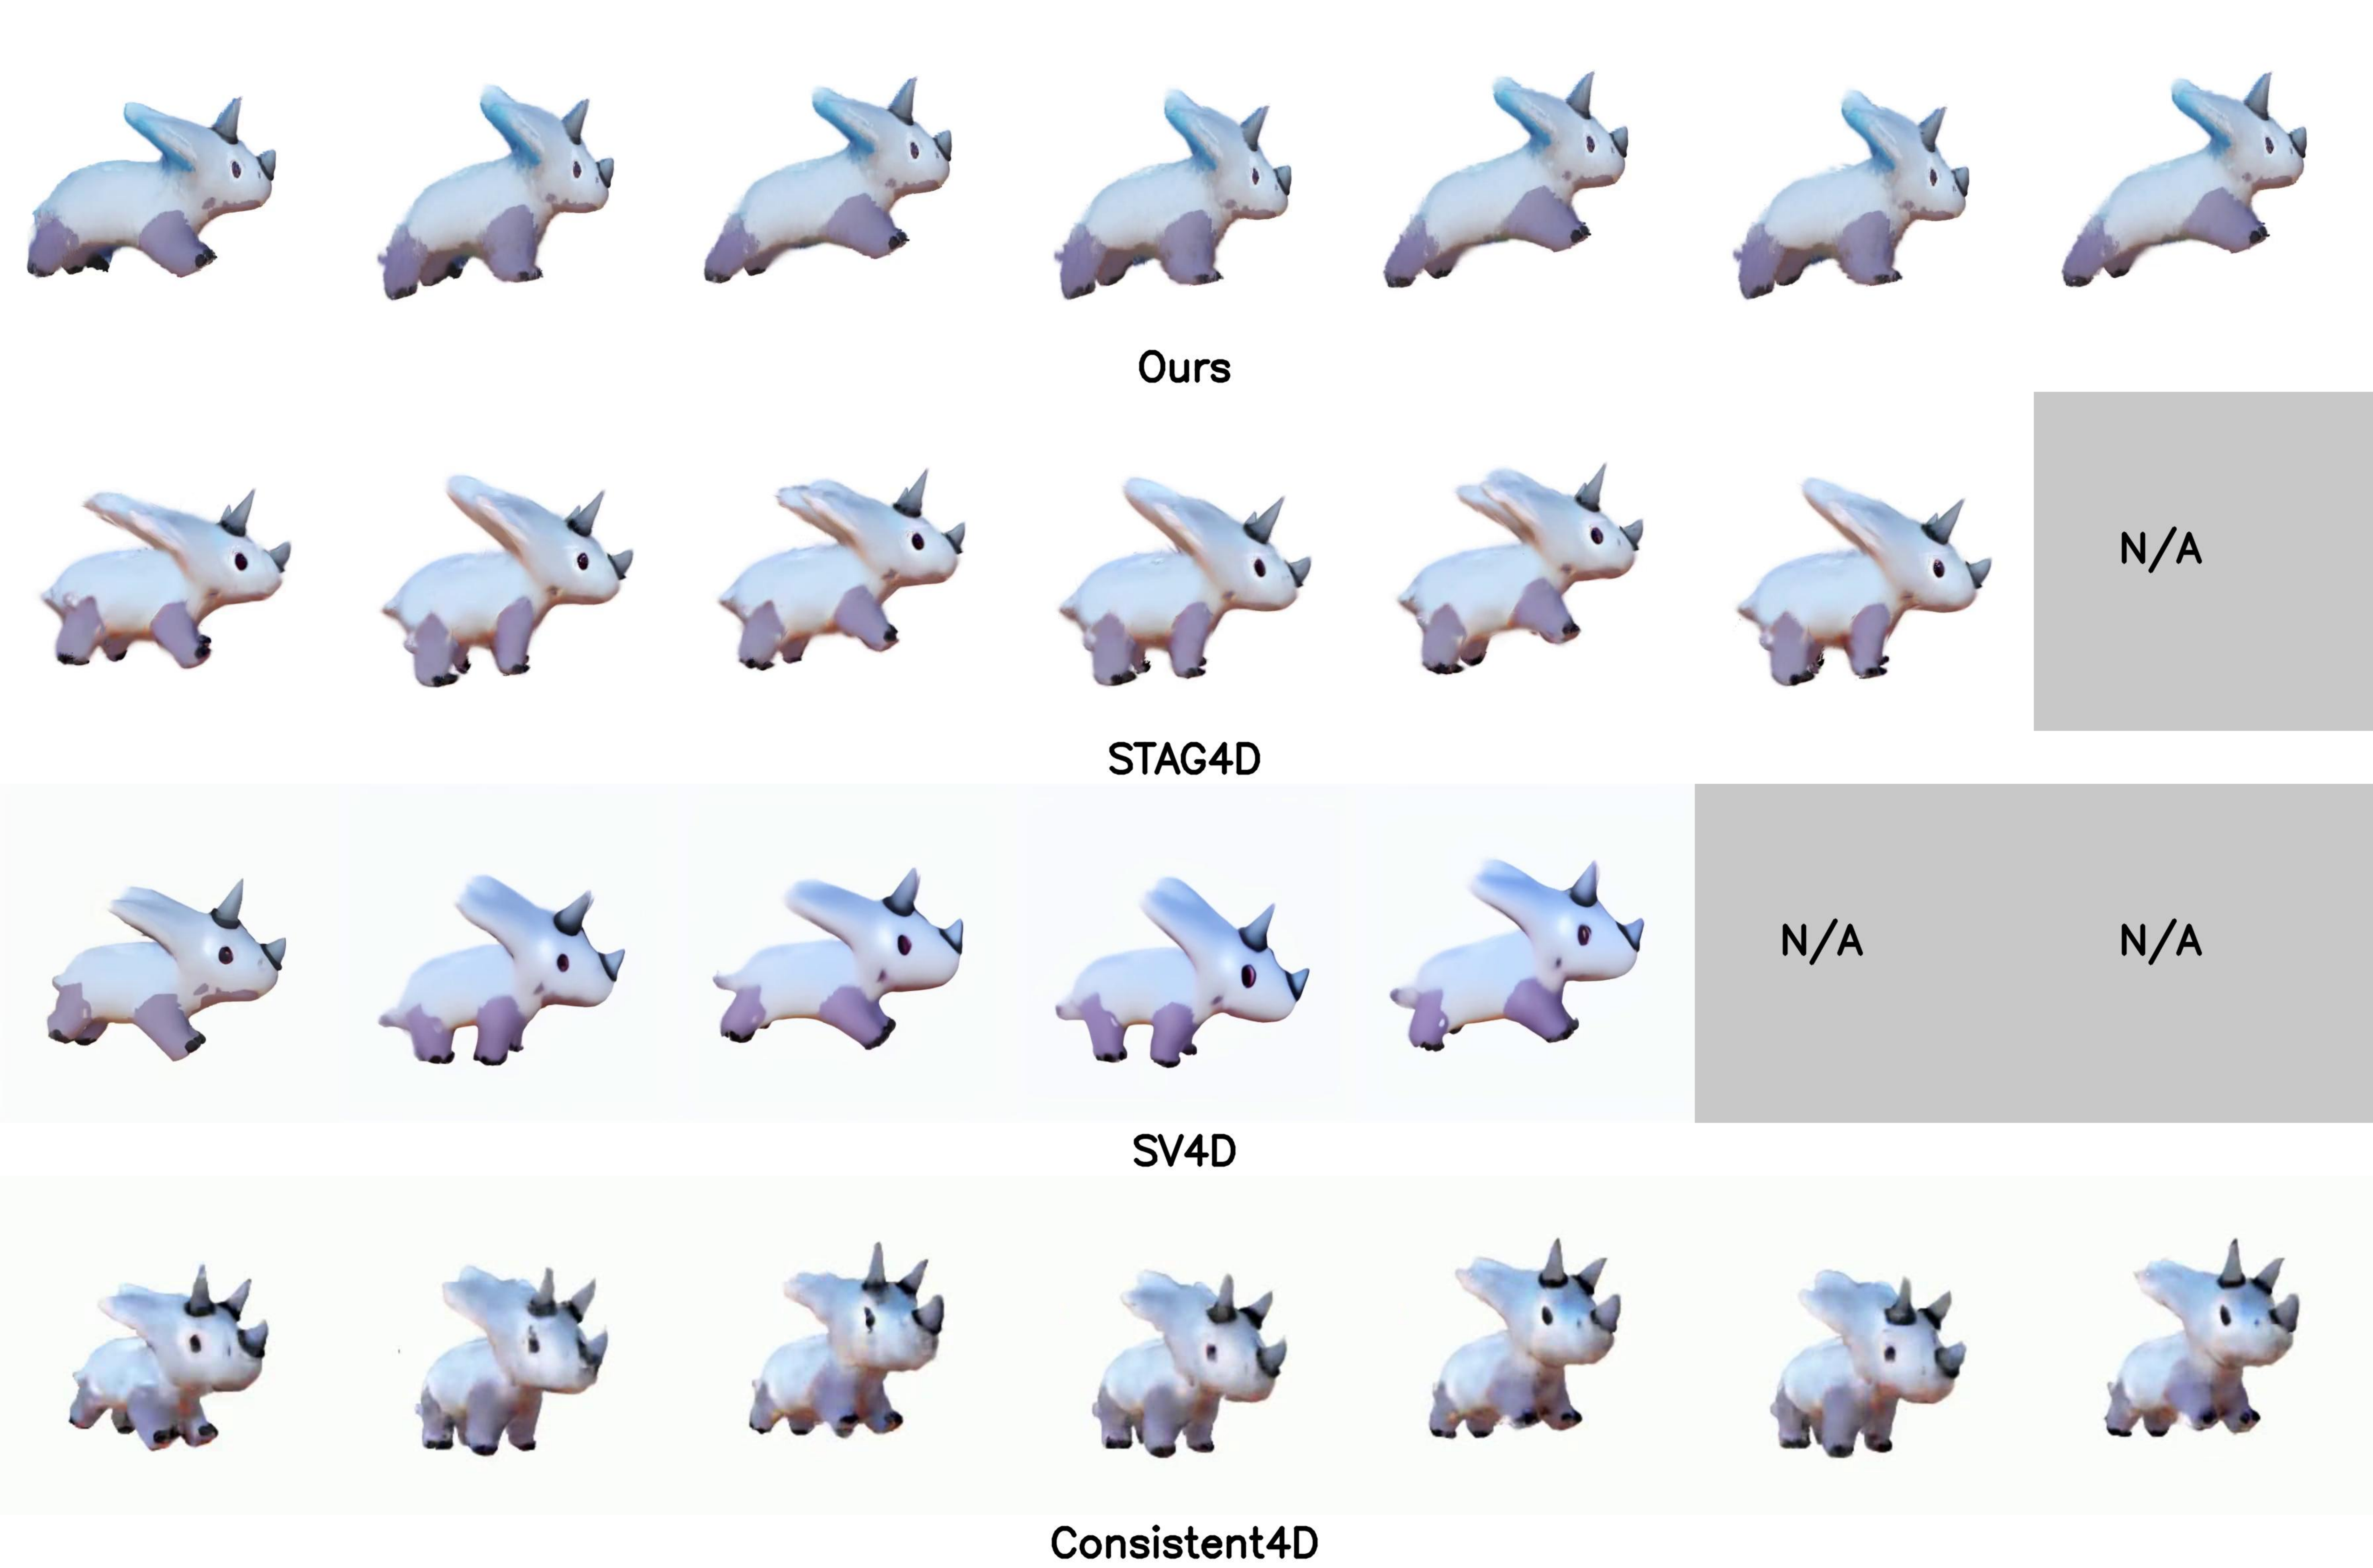}
        \caption{Comparison of novel-view videos rendered by our method and other state-of-the-art methods at novel view 1.}
    \end{subfigure}
    \hfill
    \begin{subfigure}[b]{1\textwidth}
        \centering
        \includegraphics[width=0.85\textwidth]{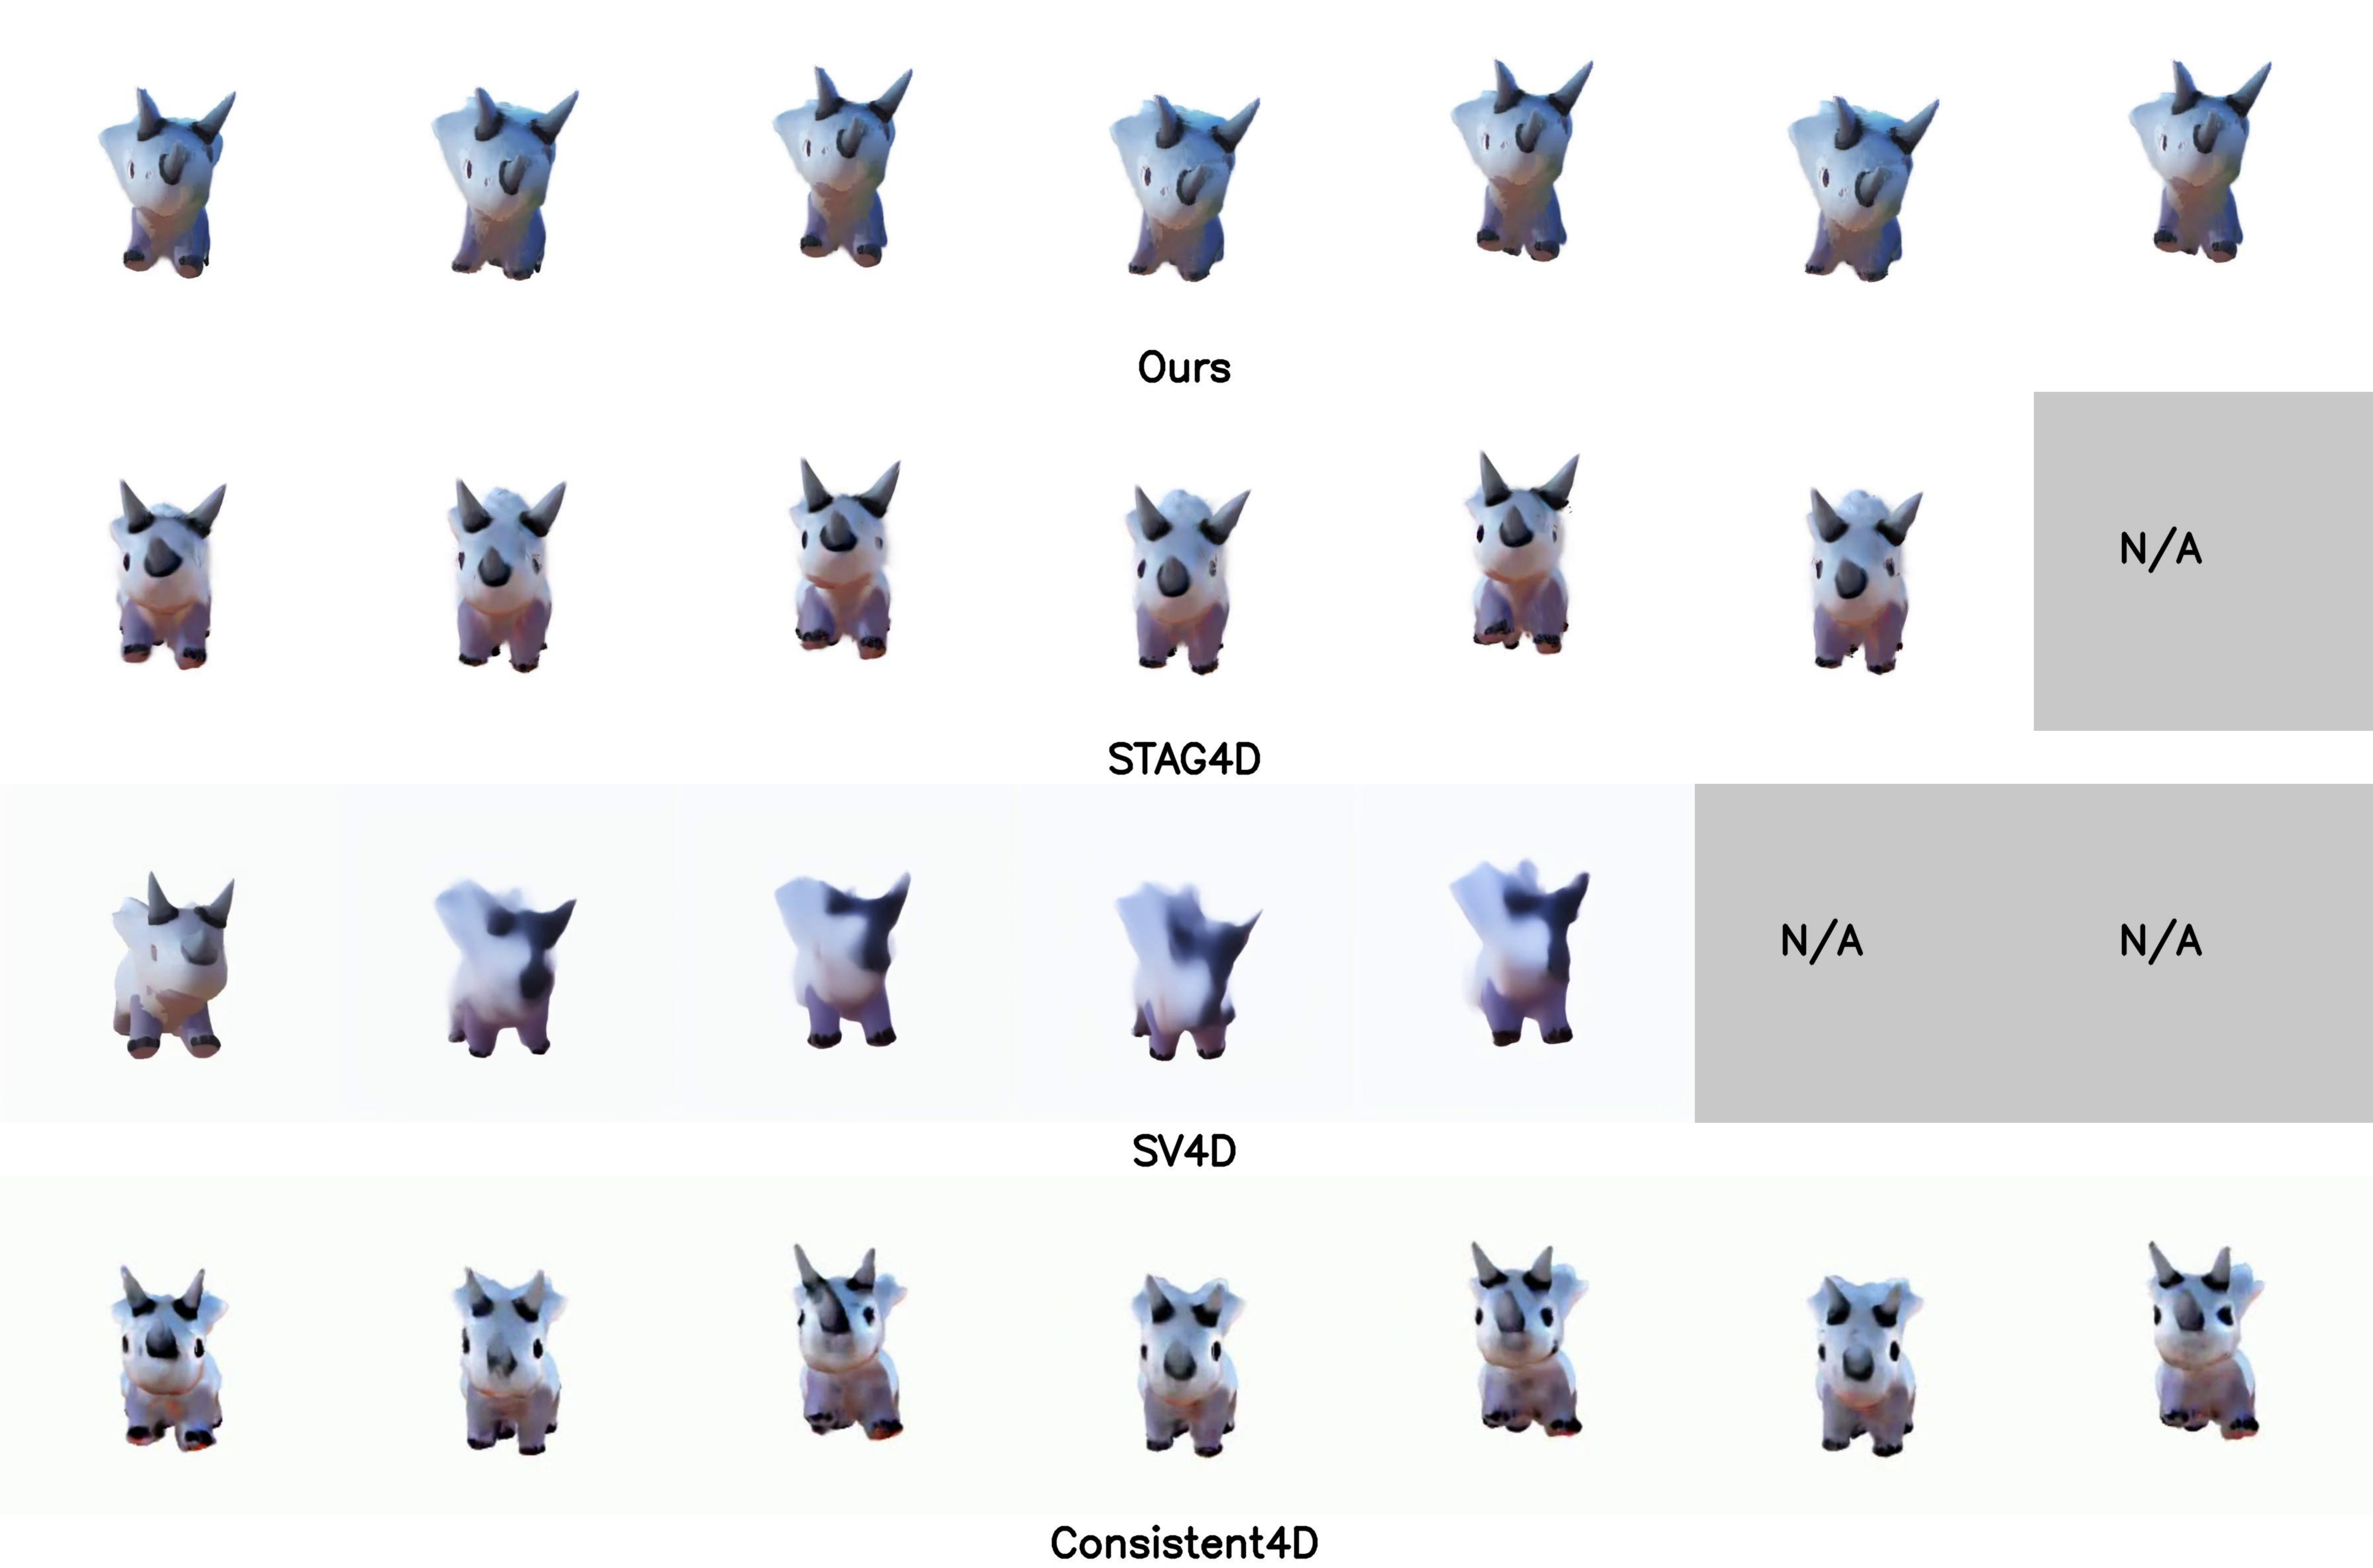}
        \caption{Comparison of novel-view videos rendered by our method and other state-of-the-art methods at novel view 2.}
    \end{subfigure}
    \hfill
    \caption{More visualizations of comparison of novel-view videos rendered by our method and other state-of-the-art methods at different novel views on the task of Video-to-4D. $\textbf{\textit{N/A}}$ indicates that the corresponding method fails to generate novel views for the current frame.}
    \label{fig:supply_compaisons_2}
\end{figure*}

\begin{figure*}[t]
    \centering
    \begin{subfigure}[b]{1\textwidth}
        \centering
        \includegraphics[width=0.73\textwidth]{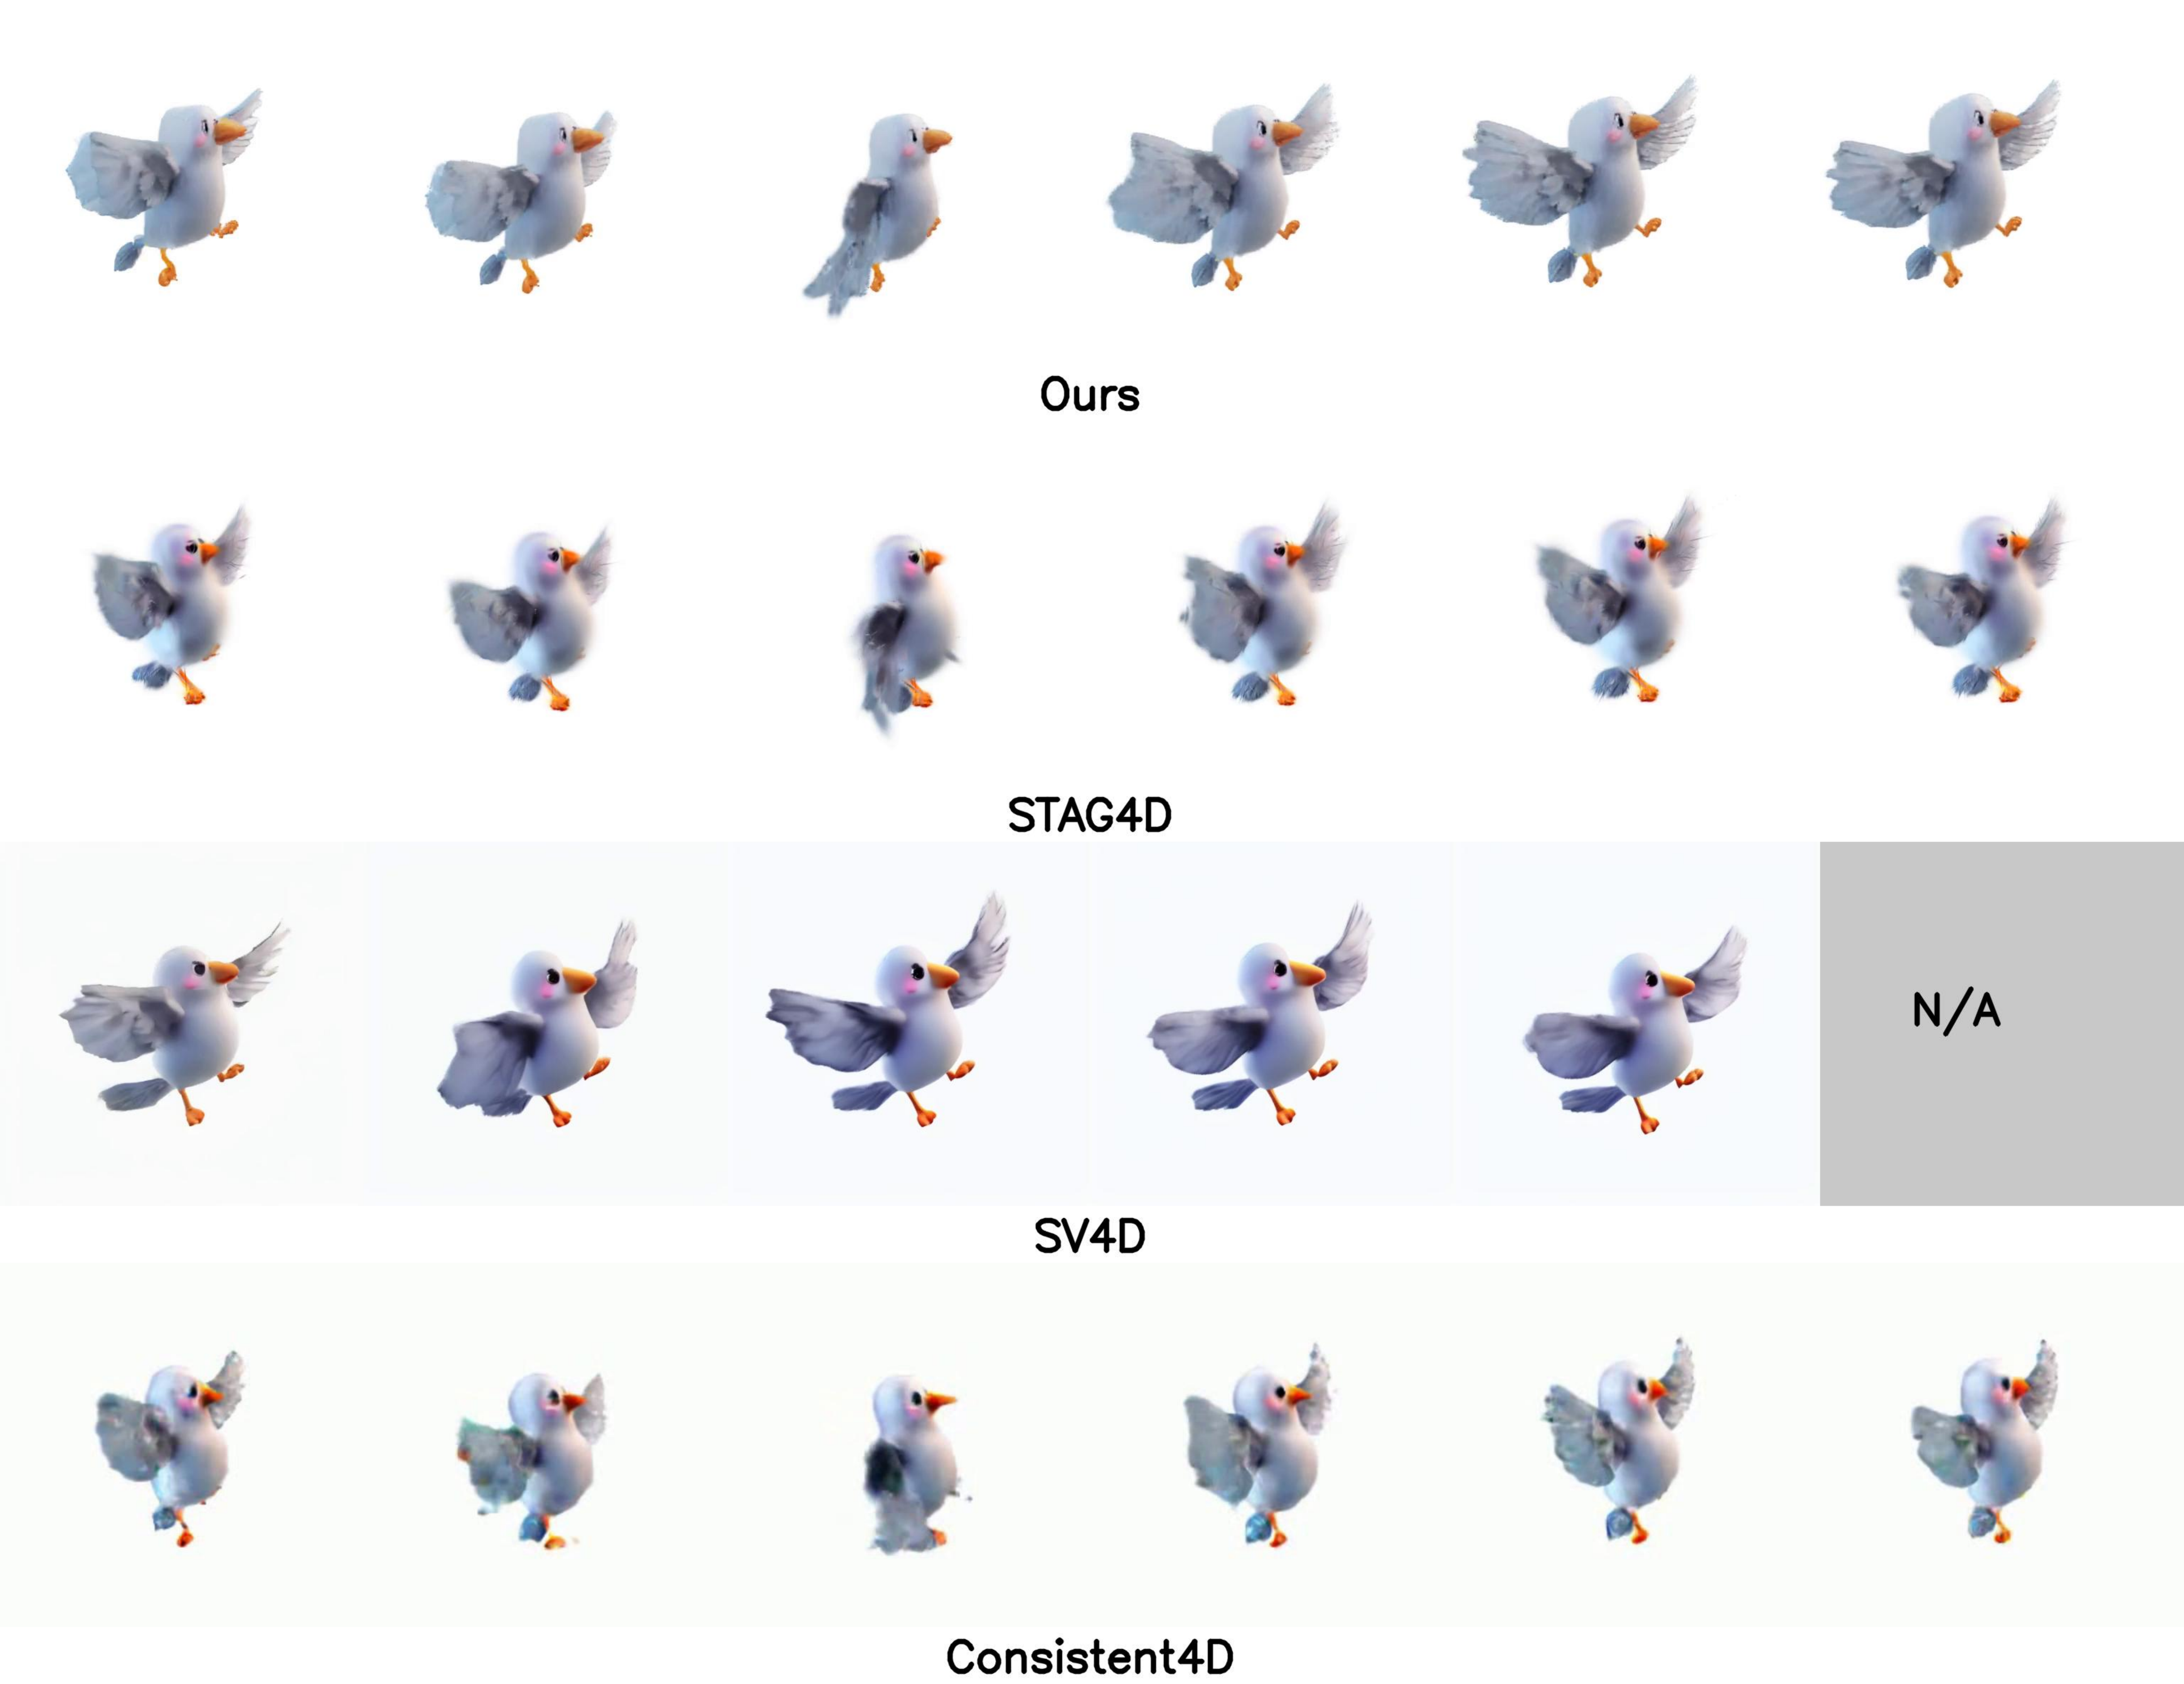}
        \caption{Comparison of novel-view videos rendered by our method and other state-of-the-art methods at novel view 1.}
    \end{subfigure}
    \hfill
    \begin{subfigure}[b]{1\textwidth}
        \centering
        \includegraphics[width=0.73\textwidth]{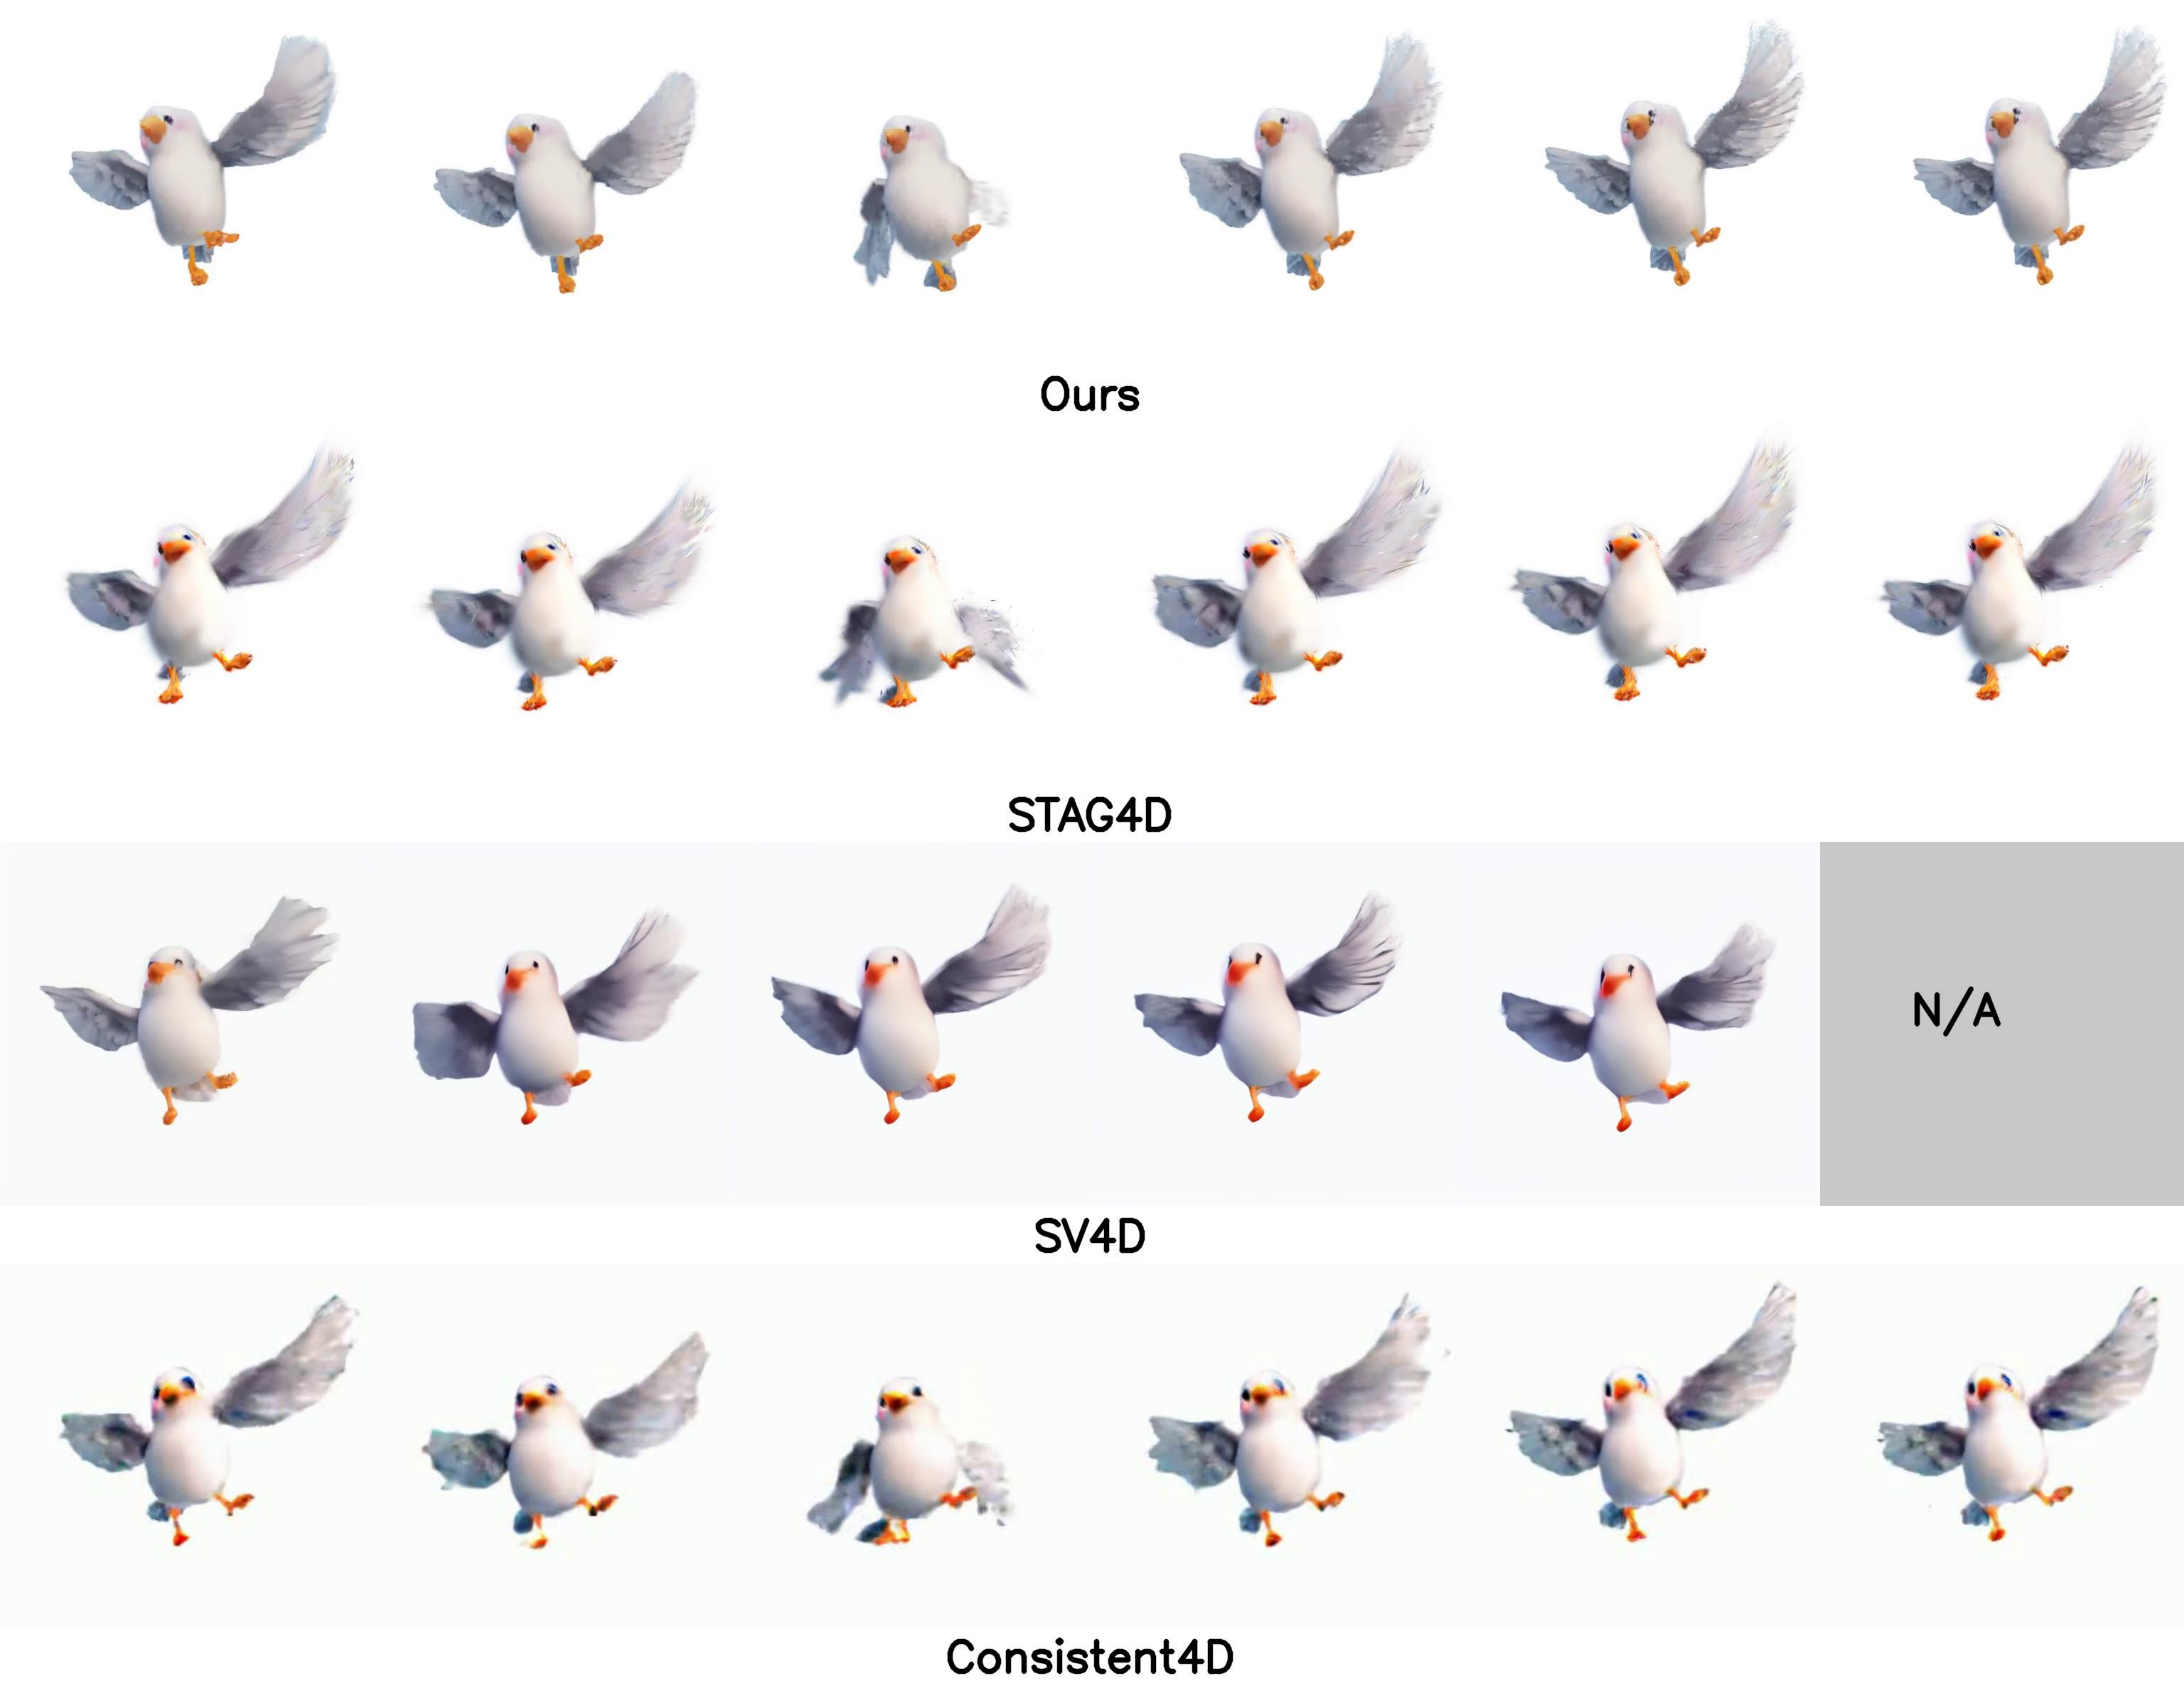}
        \caption{Comparison of novel-view videos rendered by our method and other state-of-the-art methods at novel view 2.}
    \end{subfigure}
    \hfill
    \caption{More visualizations of comparison of novel-view videos rendered by our method and other state-of-the-art methods at different novel views on the task of Text-to-4D. $\textbf{\textit{N/A}}$ indicates that the corresponding method fails to generate novel views for the current frame.}
    \label{fig:supply_compaisons_4}
\end{figure*}

\section{More visualizations of 4D assets generated by AR4D}\label{More visualizations of 4D assets generated by AR4D}
In this section, we provide more results of the 4D assets generated by our proposed AR4D. As demonstrated in Fig.~\ref{fig:supply_additional_results_1}, Fig.~\ref{fig:supply_additional_results_2}, Fig.~\ref{fig:supply_additional_results_3}, Fig.~\ref{fig:supply_additional_results_4}, Fig.~\ref{fig:supply_additional_results_5}, and Fig.~\ref{fig:supply_additional_results_6}, the rendered novel-view videos exhibit superior spatial-temporal consistency.

\begin{figure*}[t]
    \centering
\includegraphics[width=1\linewidth]{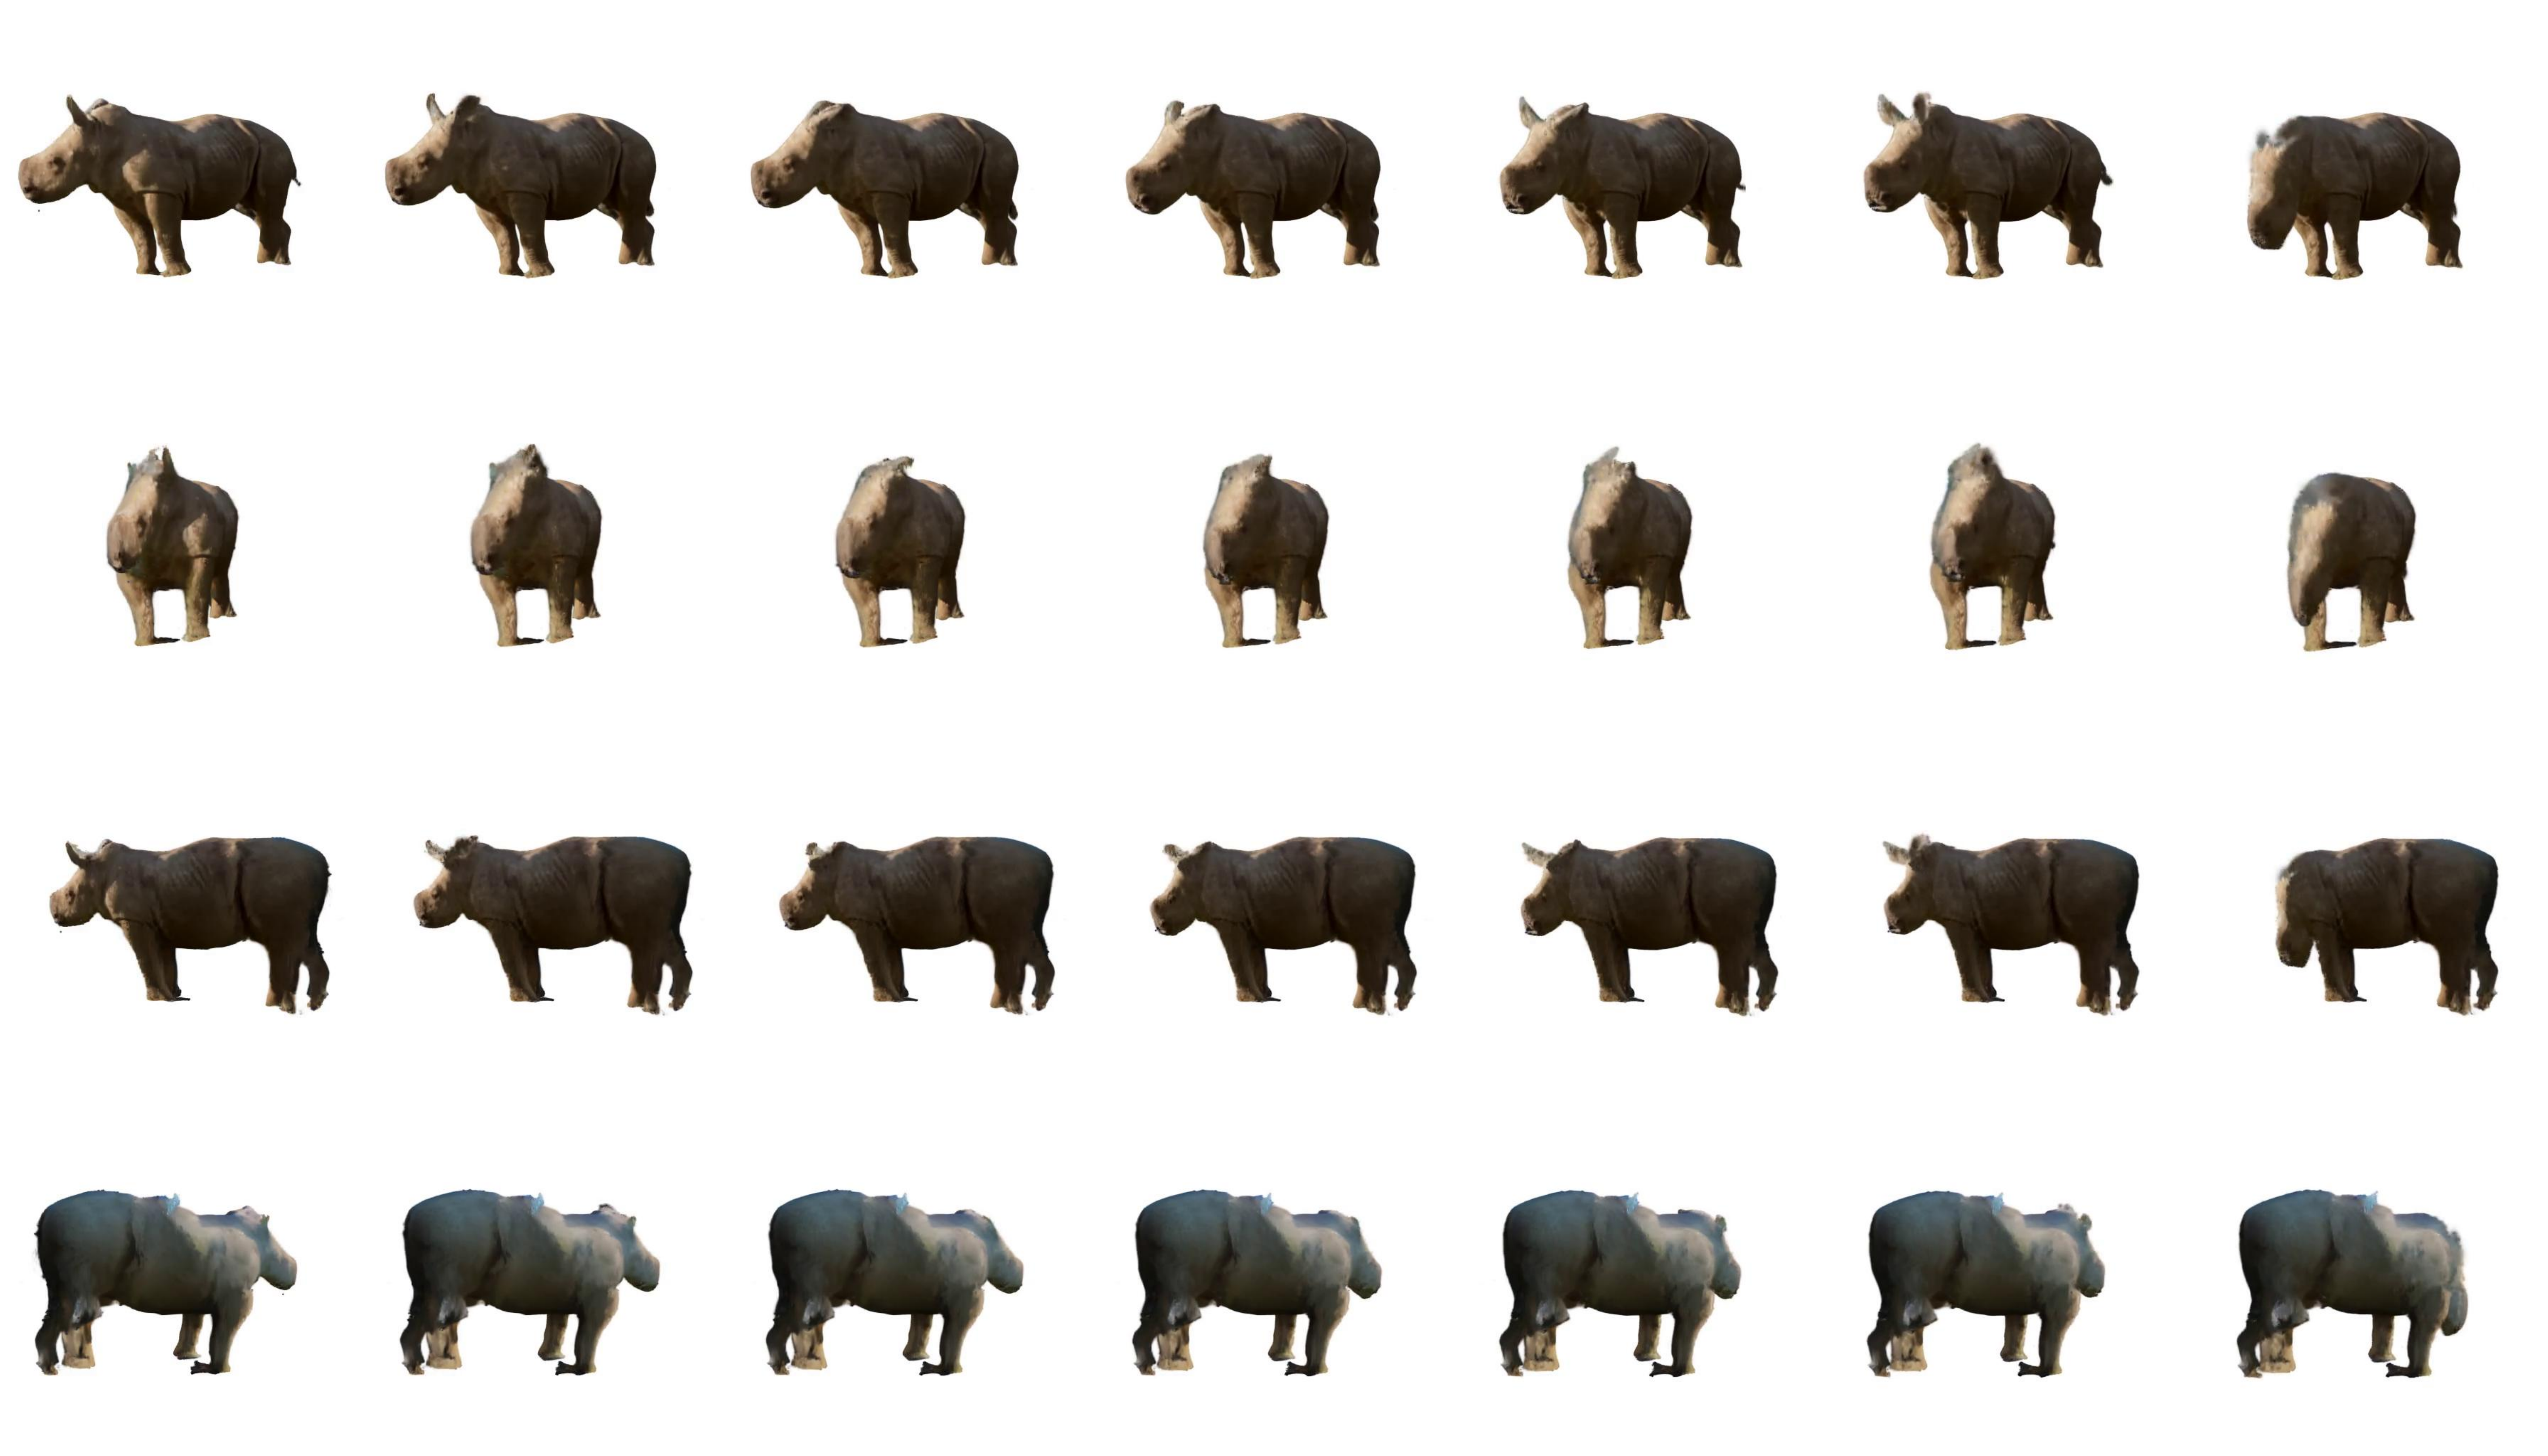}
    \caption{Additional results of multi-view videos rendered by AR4D, with the azimuth angles of $\ang{0},\ang{-45}, \ang{45}, \ang{180}$ respectively.}
    \label{fig:supply_additional_results_1}
\end{figure*}

\begin{figure*}[t]
    \centering
\includegraphics[width=1\linewidth]{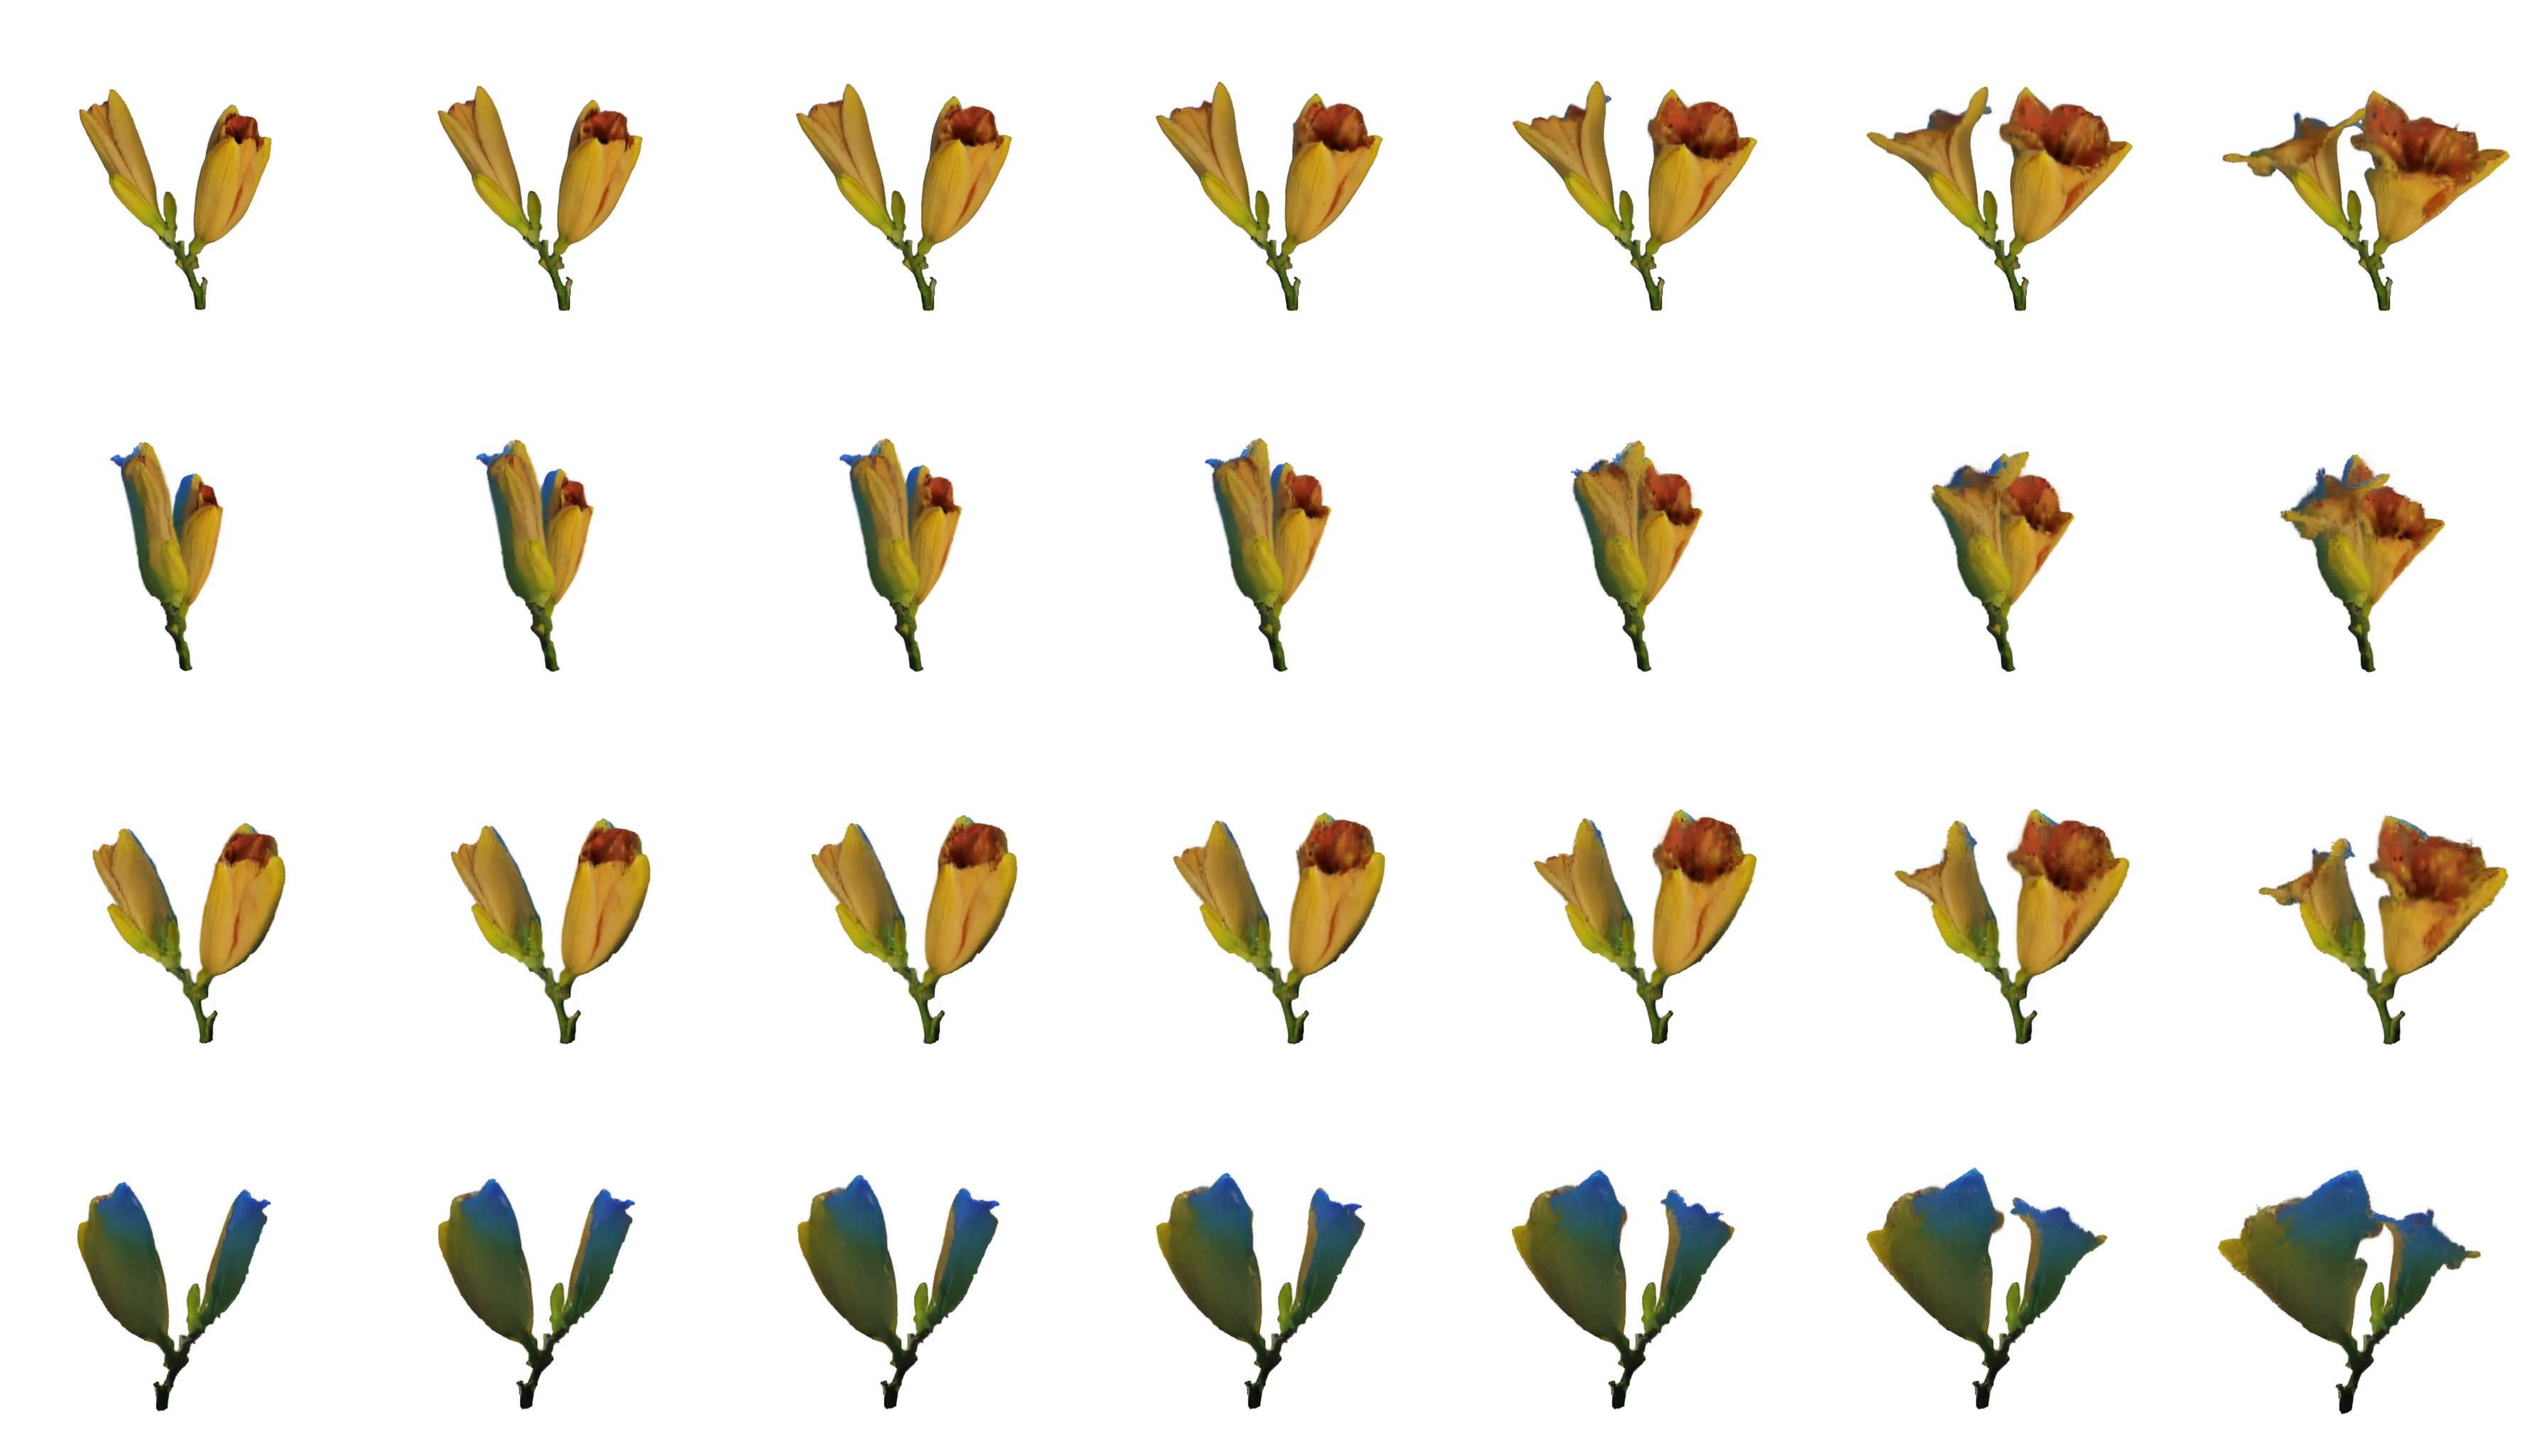}
    \caption{Additional results of multi-view videos rendered by AR4D, with the azimuth angles of $\ang{0},\ang{-45}, \ang{45}, \ang{180}$ respectively.}
    \label{fig:supply_additional_results_2}
\end{figure*}

\begin{figure*}[t]
    \centering
\includegraphics[width=1\linewidth]{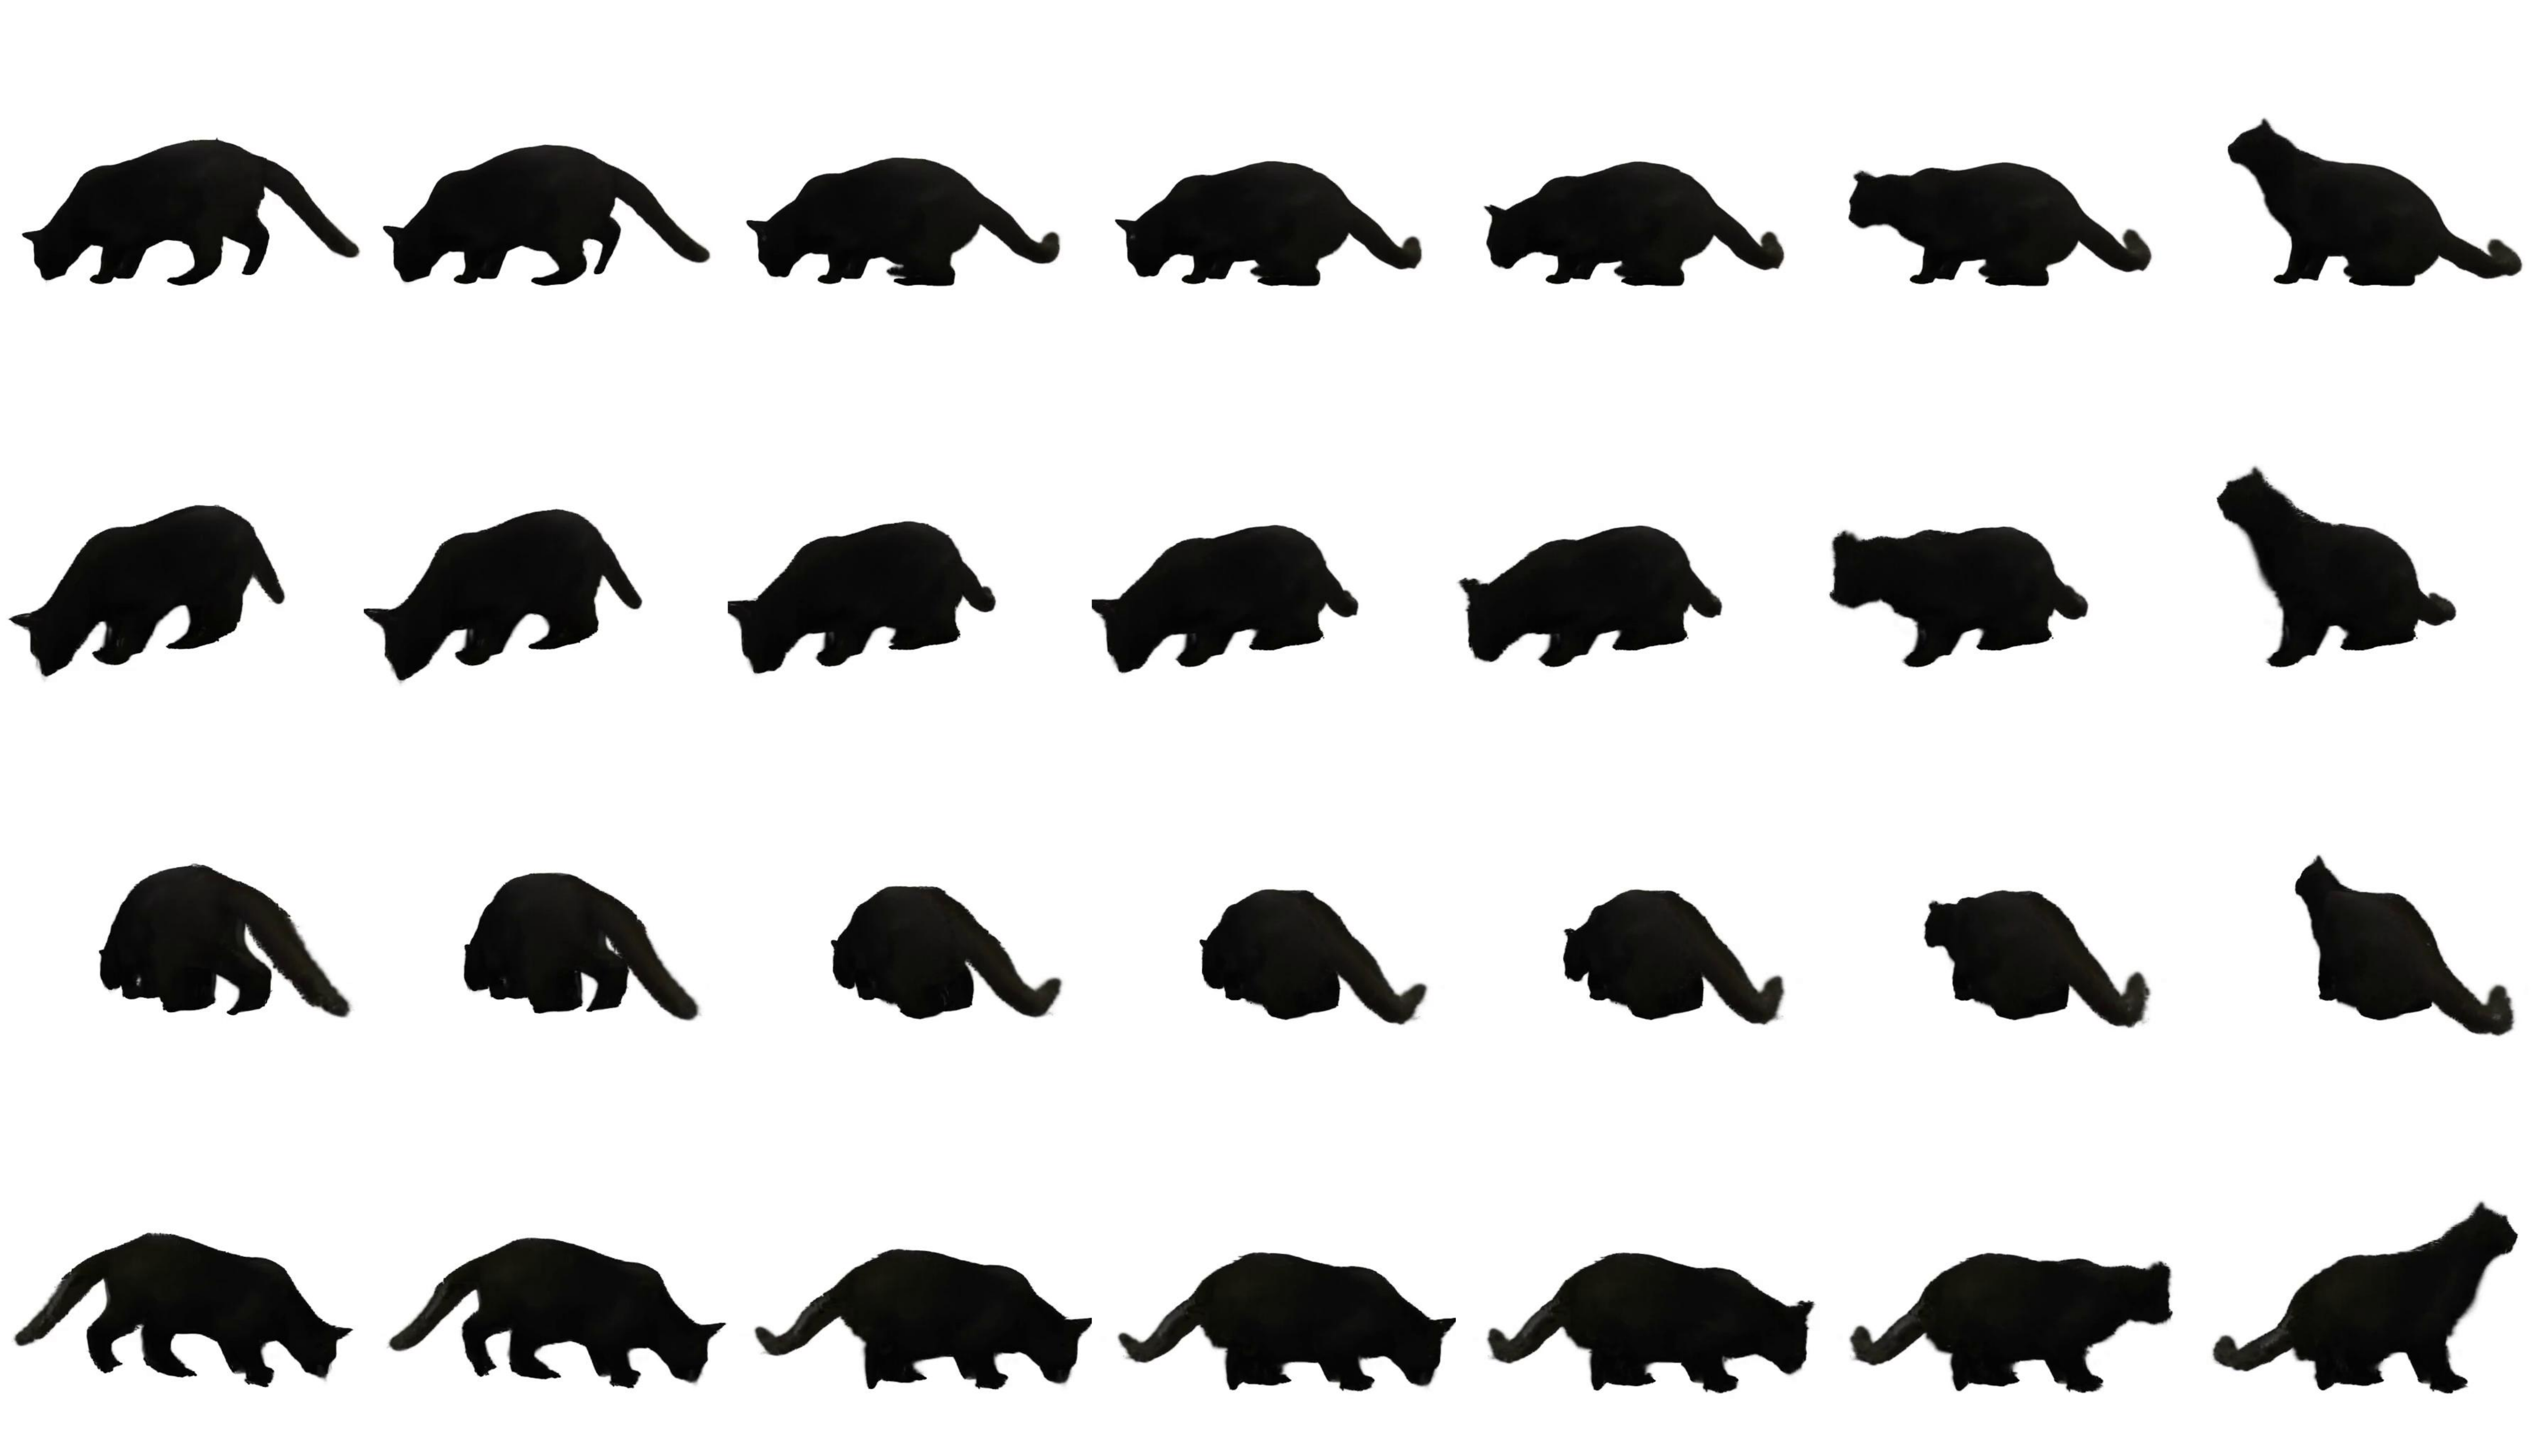}
    \caption{Additional results of multi-view videos rendered by AR4D, with the azimuth angles of $\ang{0},\ang{-45}, \ang{45}, \ang{180}$ respectively.}
    \label{fig:supply_additional_results_3}
\end{figure*}

\begin{figure*}[t]
    \centering
\includegraphics[width=1\linewidth]{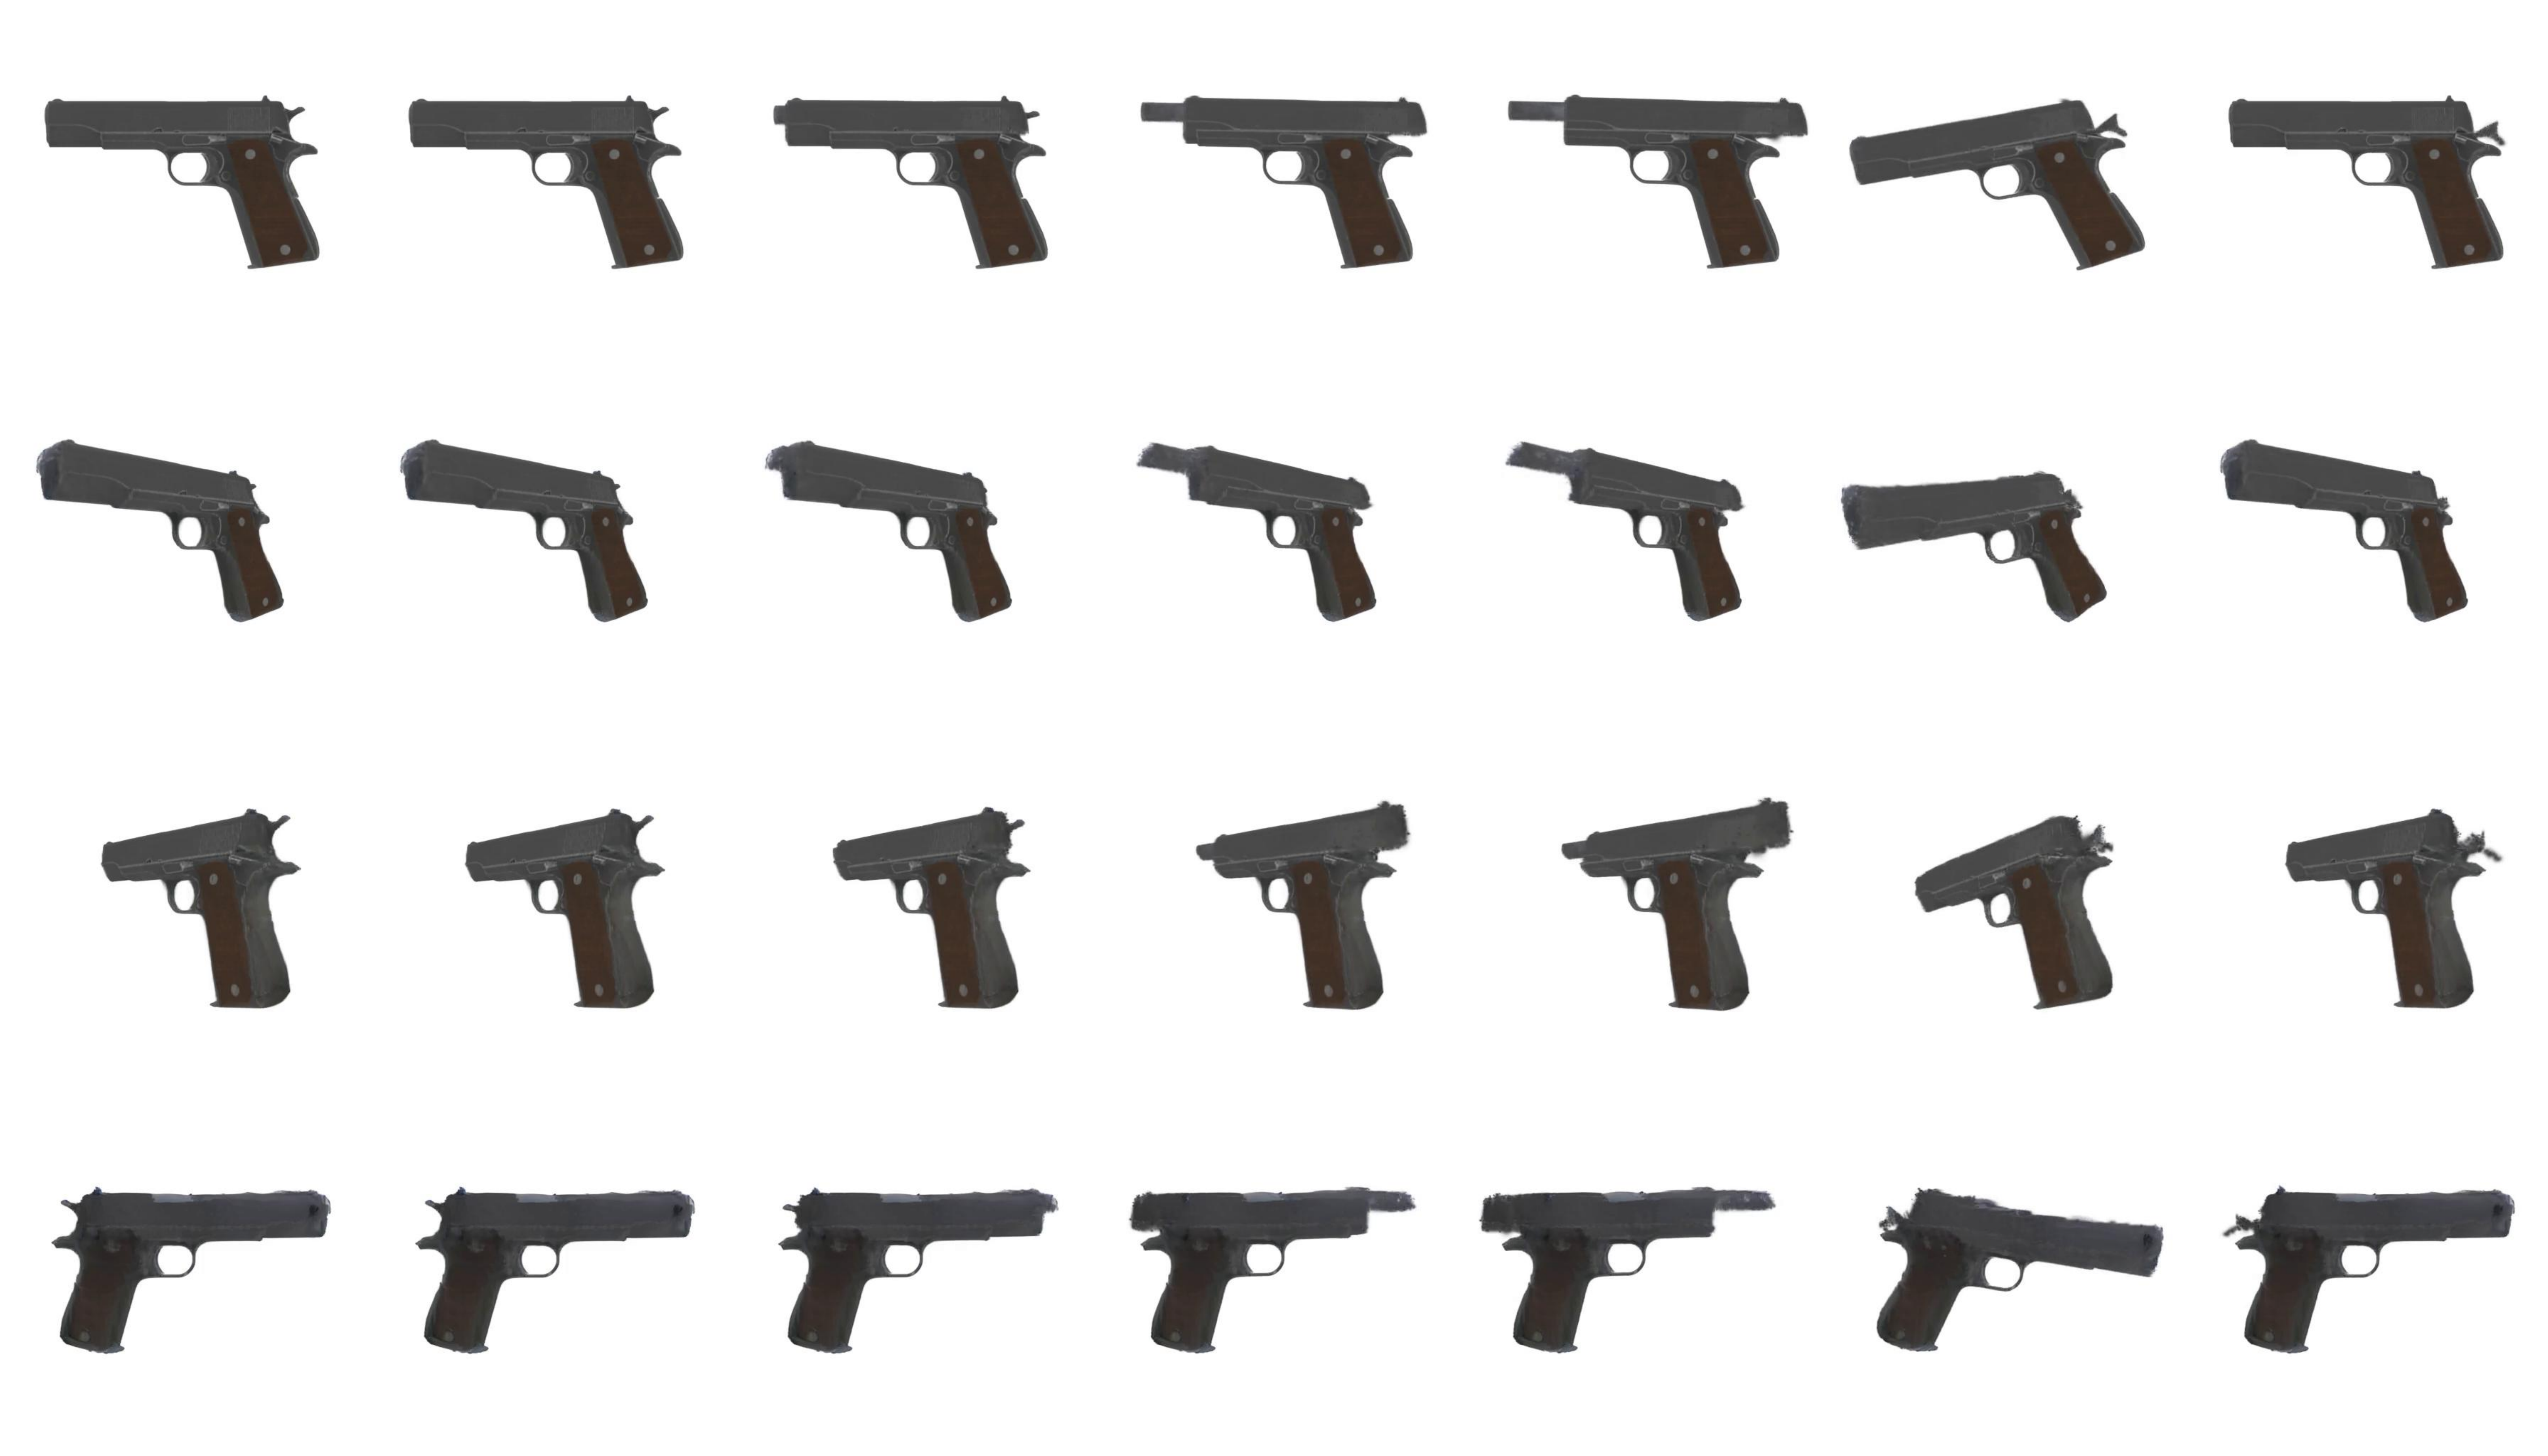}
    \caption{Additional results of multi-view videos rendered by AR4D, with the azimuth angles of $\ang{0},\ang{-45}, \ang{45}, \ang{180}$ respectively.}
    \label{fig:supply_additional_results_4}
\end{figure*}

\begin{figure*}[t]
    \centering
\includegraphics[width=1\linewidth]{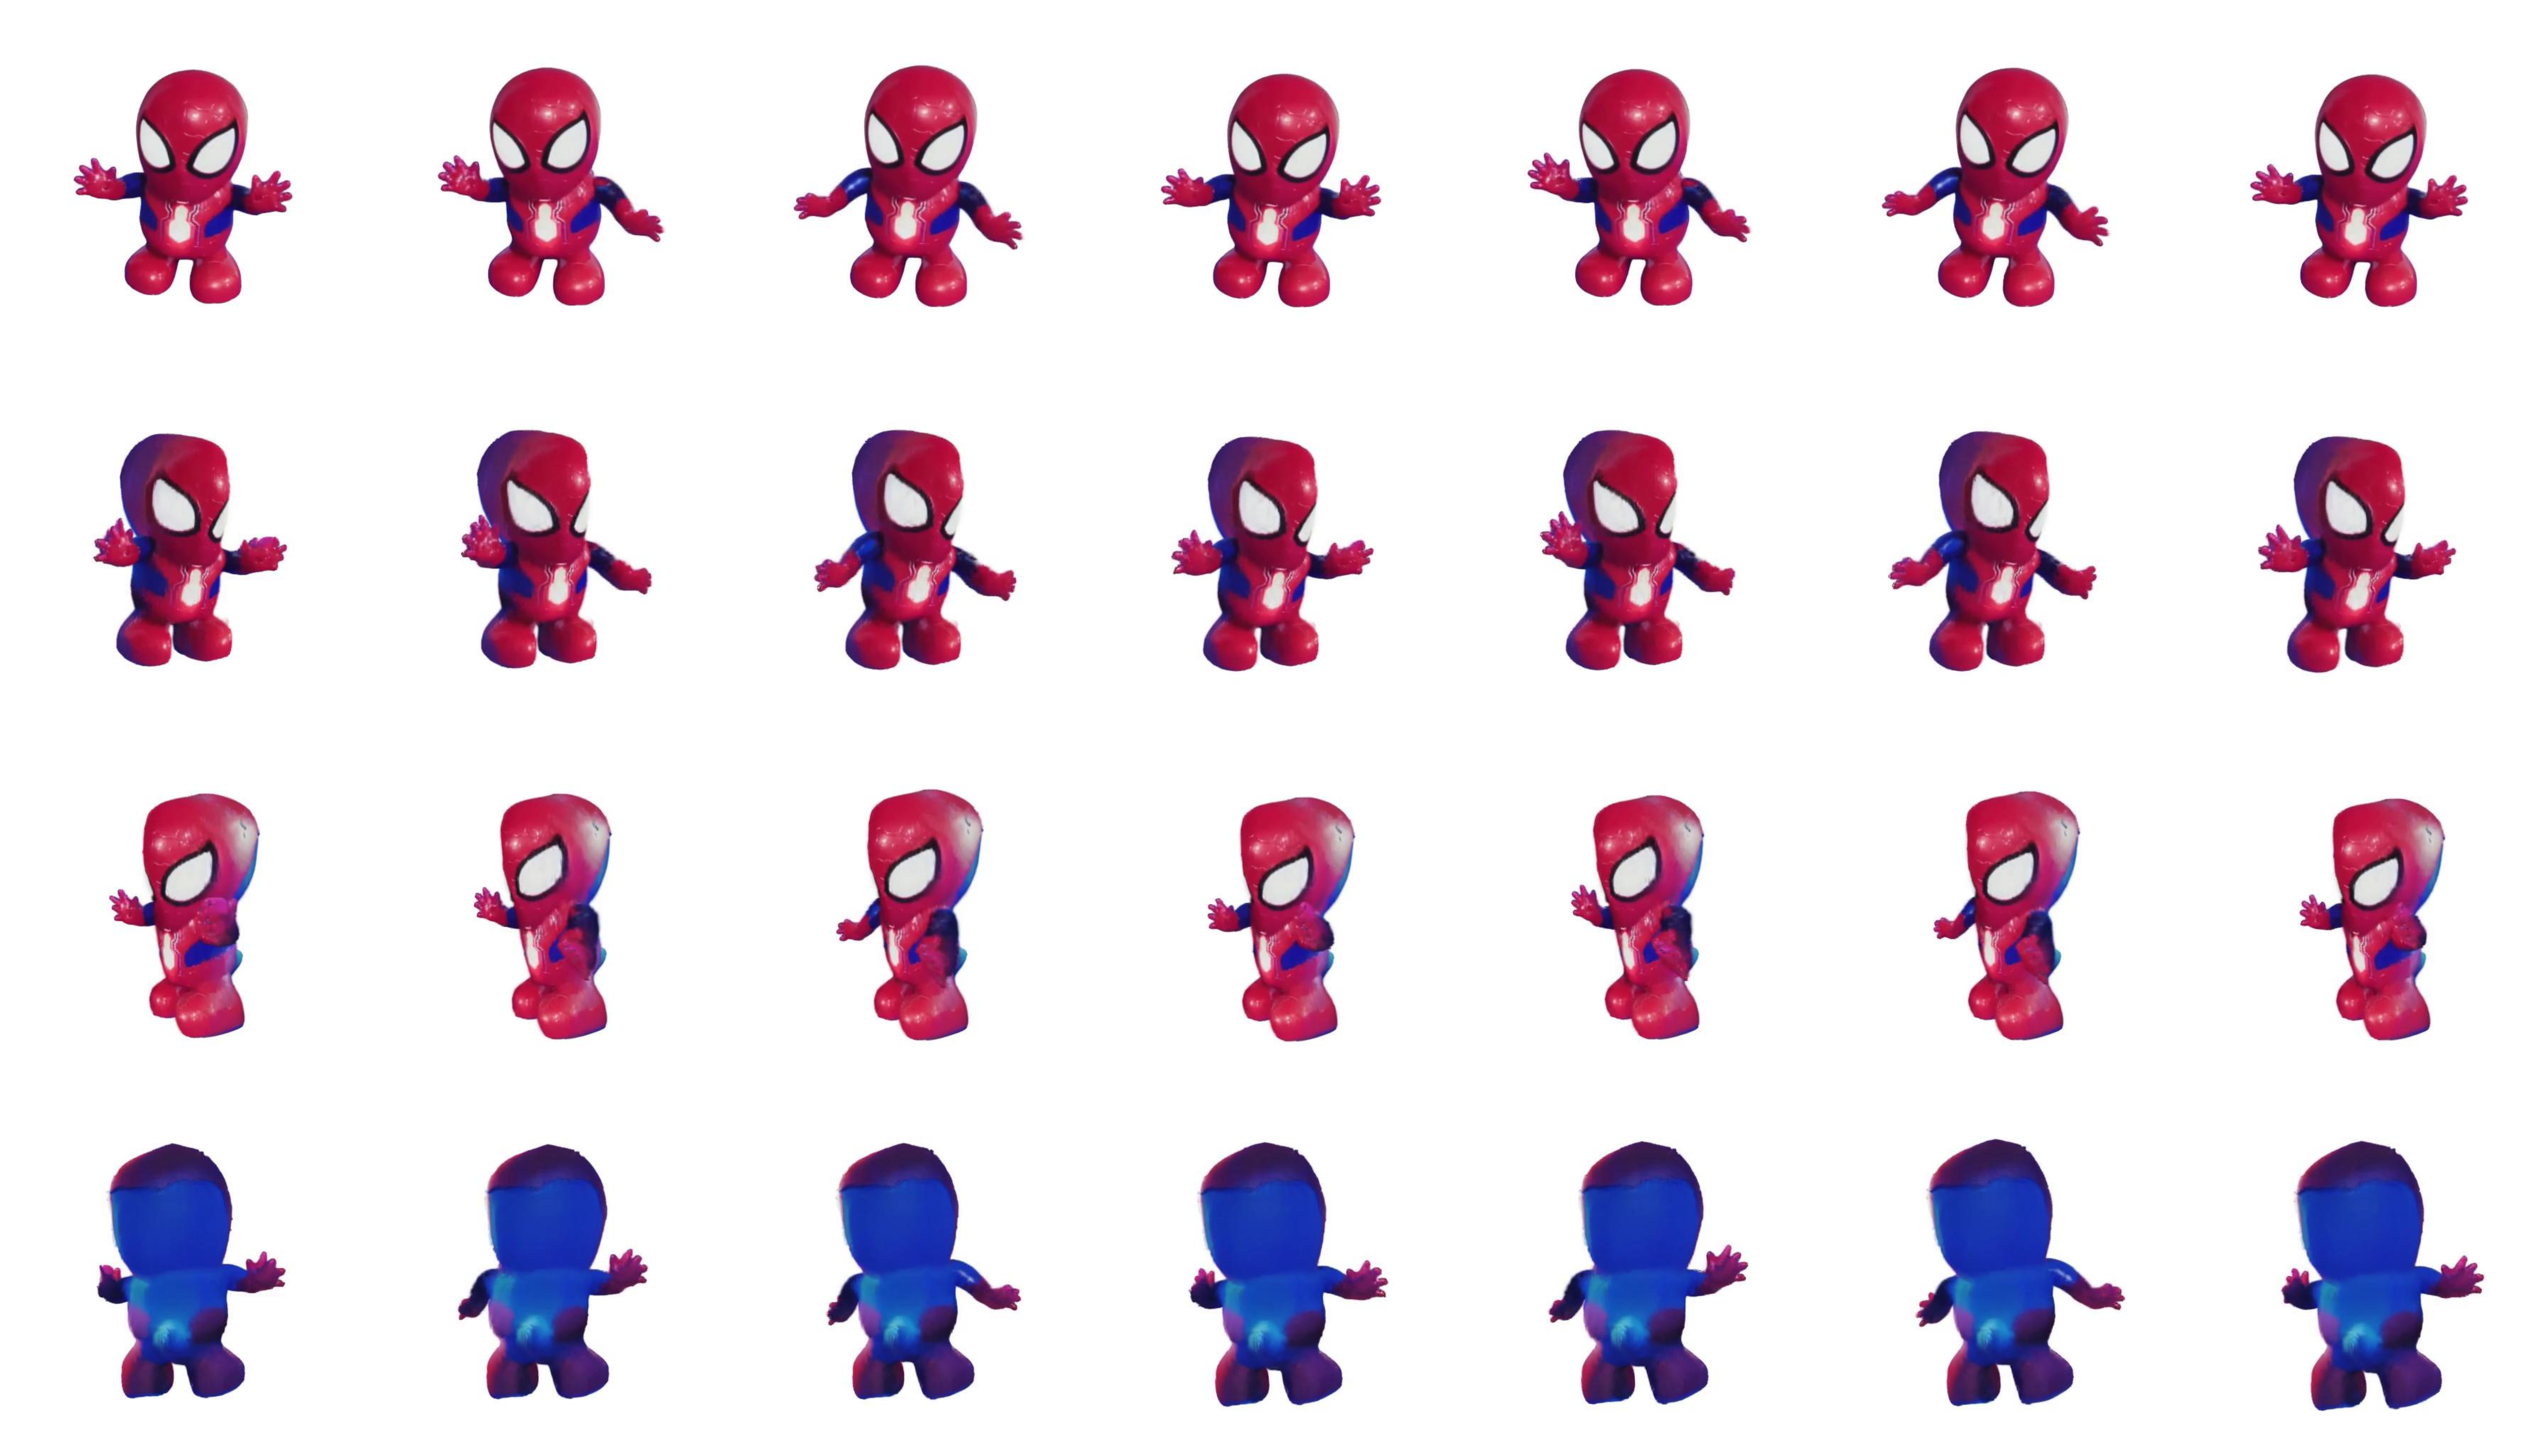}
    \caption{Additional results of multi-view videos rendered by AR4D, with the azimuth angles of $\ang{0},\ang{-45}, \ang{45}, \ang{180}$ respectively.}
    \label{fig:supply_additional_results_5}
\end{figure*}

\begin{figure*}[t]
    \centering
\includegraphics[width=1\linewidth]{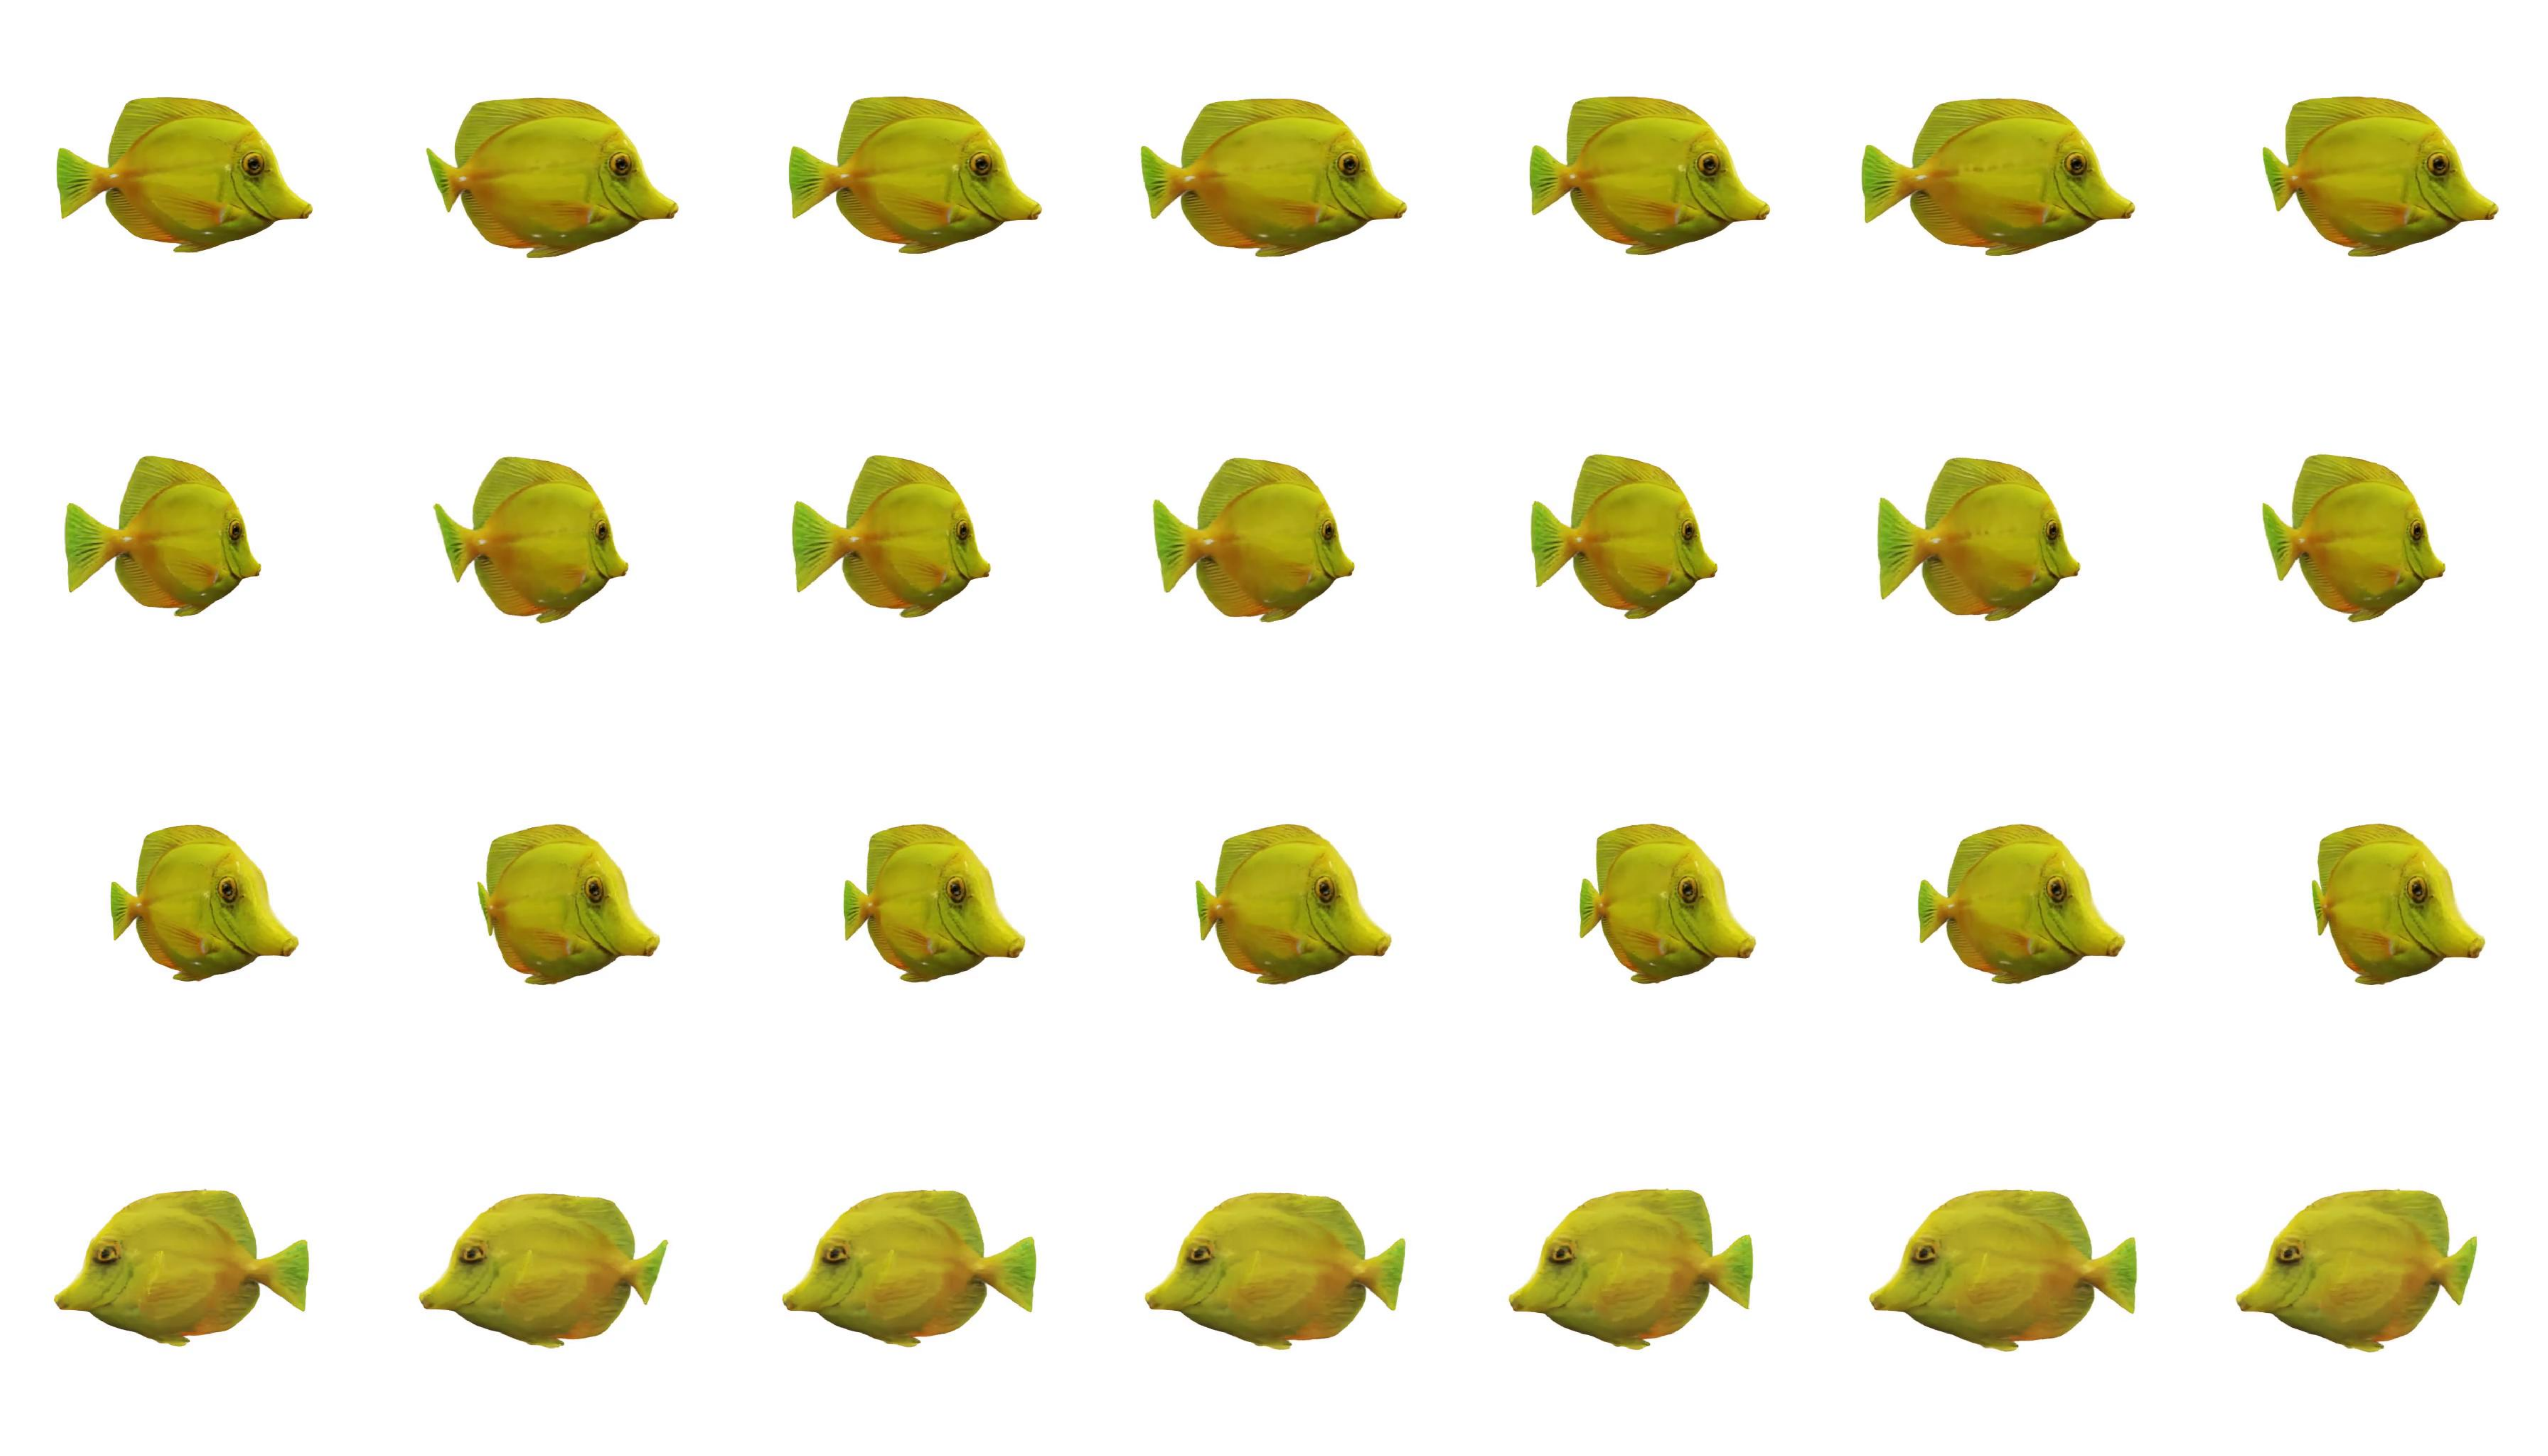}
    \caption{Additional results of multi-view videos rendered by AR4D, with the azimuth angles of $\ang{0},\ang{-45}, \ang{45}, \ang{180}$ respectively.}
    \label{fig:supply_additional_results_6}
\end{figure*}

\section{Limitations and future works}\label{Limitations and future works}
Our proposed method is designed to enable 4D generation from monocular videos, achieving state-of-the-art performance. However, despite the SDS-free nature of our approach, which facilitates 4D generation of complex scenes, its performance is constrained by the limitations of the pre-trained large-scale 3D reconstruction models used (e.g., Splatt3R~\cite{smart2024splatt3r}). Specifically, the method struggles with generating novel views of videos that exhibit large disparity changes. In future work, we plan to develop more advanced large-scale 3D reconstruction models and incorporate additional priors, such as optical flow, to improve the performance of 4D generation for complex scenes.
